# Supplementary material for: SVDistNet: Self-Supervised Near-Field Distance Estimation on Surround View Fisheye Cameras
Source: arXiv:2104.04420 source file (2021-04-09)
Supplement: Supplementary file 1 [file supplementary.tex]

% \section*{\textbf{Supplementary Material}}

\twocolumn 
\begin{center}  
{\noindent \large \textbf{Supplementary Material}} \\
\end{center}
In this supplementary section, we provide additional results and qualitative figures and further insight on the network and ablation studies.\par
% -------------------------------------------------
\subsection{\textbf{Vector based Self-Attention Encoders}}
\label{sec:vector-self-attention}

Most of the previous depth estimation networks~\cite{Godard2019, zhou2017unsupervised, kumar2020unrectdepthnet} use regular convolutions for capturing the local information in an image; one of the major drawbacks is that convolution lacks rotation invariance. The kernel $K$'s footprint increases the number of parameters to be learned, and due to the filter's fixed nature, aggregation of neighborhood information can not adapt to its contents. Hu~\etal~\cite{hu2019local} and Ramachandran~\etal~\cite{ramachandran2019stand} perceived that self-attention could be a feasible choice for developing models for image perception rather than merely enhancing discrete convolutional operation layers. Inspired by~\cite{zhao2020exploring}, we incorporate the self-attention network (SAN) backbone to our encoder and compare it with the standard ResNet18~\cite{he2016deep} and ResNet50~\cite{he2016deep} choice of encoder networks. Compared to the scalar attention self-attention layers used in our previous work~\cite{kumar2020syndistnet}, which are only content-adaptive and not channel-adaptive. The vector attention work of Zhao~\cite{zhao2020exploring} has a smaller footprint than the ResNet family of standard encoder heads, and the vector attention is both content and channel adaptive. The authors showcase two convolution variants, namely \emph{pairwise} and \emph{patchwise}, which may replace convolution while reducing the number of parameters and giving advantages in terms of robustness and generalization.\par
% -------------------------------------------------
\textbf{\textit{Pairwise Self-Attention}} The \emph{pairwise} self-attention module is given by:
\begin{equation}
	\label{eq:pairwise}
	z_{ij} = \sum_{ab \in \mathcal{N}_r(ij)} \eta(x_{ij}, x_{ab}) \odot \chi(x_{ab})
\end{equation}
The location of the spatial index in the feature vector $x_{ij}$ is denoted by $ij$, $\odot$ is the Hadamard product, and the aggregation of the local footprint is $\mathcal{N}_r(ij)$.
The new feature $z_{ij} \in \mathbb{R}^{d_{out}}$ is constructed by aggregating the feature vectors specified by the set of indices by the footprint $\mathcal{N}_r(ij)$. The adaptive weight vectors $\eta(x_{ij}, x_{ab})$ aggregate the feature vectors $\chi(x_{ab})$ produced by the function $\chi$. The weights $\eta(x_{ij}, x_{ab})$ required to combine the transformed features $\chi(x_{ab})$ are computed by the function $\eta$. $\eta$ is decomposed to elucidate the different forms of self-attention and is given by:
\begin{equation}
	\label{eq:pairwise-decomposition}
	\eta(x_{ij}, x_{ab}) = \zeta(\delta(x_{ij},x_{ab}))
\end{equation}
The features $x_{ij}$ and $x_{ab}$ are expressed by a single vector outputted by the relation function $\delta$. This vector is used along with the function $\zeta$ to map a vector that can be combined with $\chi(x_{ab})$ as shown in Eq.~\ref{eq:pairwise}. The $\zeta$ function allows us to explore $\delta$ relationships that generate vectors of varying dimensionality that do not need to match the $\chi(x {ab})$ dimensionality. In this paper, we choose the relation function $\delta$ to be described by the \textit{Hadamard product} form from~\cite{zhao2020exploring}.
\begin{equation}
    \delta(x_{ij}, x_{ab}) = \varphi(x_{ij})\odot\psi(x_{ab})
\end{equation}
where $\varphi$ and $\psi$ are transformations that can be trained, which suit the dimensionality of the output. The dimensionality of $\delta(x_{ij},x_{ab})$ is the same as that of the transformation functions with the Hadamard product.\par
% -------------------------------------------------
\textbf{\textit{Patchwise Self-Attention}}
The \emph{patchwise} self-attention module is given by:
\begin{equation}
	\label{eq:patchwise}
	z_{ij} = \sum_{ab \in \mathcal{N}_r(ij)} \eta(x_{\mathcal{N}_r(ij)})_{ab} \odot \chi(x_{ab})
\end{equation}
In the footprint ${\mathcal{N}_r(ij)}$, the patch of feature vectors are given by $x_{\mathcal{N}_r(ij)}$.
$\eta(x_{\mathcal{N}_r(ij)})$ and the patch  $x_{\mathcal{N}_r(ij)}$ have the same spatial dimensionality. $\eta(x_{\mathcal{N}_r(ij)})_{ab}$ is a vector located at $ab$ in that tensor, corresponding to $x_{ab}$ vector in $x_{\mathcal{N}_r(ij)}$ spatially. 
%The Patchwise self-attention concerning the features $x_{ab}$ is no longer a set operation compared to its pairwise counterpart. 
It is not permutation-invariant or cardinality-invariant: the $\eta(x_{\mathcal{N}_r(ij)}$ weight calculation will index the $x_{\mathcal{N}_r(ij)}$ feature vectors separately, by position, and can intermix information from feature vectors from various locations within the footprint. Therefore patchwise self-attention is especially more effective than standard convolution. $\eta(x_{\mathcal{N}_r(ij)})$ is decomposed by:
\begin{equation}
	\label{eq:patchwise-decomposition}
	\eta(x_{\mathcal{N}_r(ij)}) = \zeta(\delta(x_{\mathcal{N}_r(ij)})).
\end{equation}
The feature vector created by $\delta(x_{\mathcal{N}_r(ij)})$ is mapped by the function $\zeta$ to a tensor with the suitable dimensionality and it comprises of weight vectors for all locations $ab$. Feature vectors $x_{ab}$ from the patch $x_{\mathcal{N}_r(ij)}$ are combined by the function $\delta$. We specifically incorporate \textit{Concatenation} form from~\cite{zhao2020exploring} for the relation function $\delta$.
\begin{equation}
    \delta(x_{\mathcal{N}_r(ij)}) = [\varphi(x_{ij}), [ \psi(x_{ab})]_{\forall ab \in \mathcal{N}_r(ij)}]
\end{equation}
The pairwise and patchwise self-attention operations can be used to build residual blocks~\cite{he2016deep} for the encoder that perform both feature aggregation and transformation.\par
% -------------------------------------------------
\subsection{\textbf{Post Processing}} 
\label{subsec:postprocessing}

This subsection provides a brief overview of how the depth maps get post-processed and converted to a representation directly used by motion planning. The prime purpose of surround-view cameras is to aid 360$^\circ$ near-field sensing around the car. Low-speed maneuvering like parking requires very high accuracy of the order of 5 cm and the ability to detect small objects like curbs or potholes. We construct a 2D top-view heightmap grid at a 5 cm and 10m range resolution by targeting these requirements. We project the distance map from each image onto the top view and fill the height map cells with the height information. Due to a small overlap in the image's corners, we require a fusion scheme to combine the distance values. The spatial consistency of the scene across cameras can be exploited. We use a spatial smoothing filter to smoothen the current observation, which is then further filtered using a temporal smoothing filter. The filtered height map is illustrated in the bottom part of Figure~\ref{fig:mtl_pipeline}.
% -------------------------------------------------
\subsection{\textbf{Online Refinement and Run-Time Comparison}}

In Table~\ref{table:inference-ablation}, we report the frame rate of all previous approaches and our SVDistNet using different input resolutions and a 16-bit float precision ONNX model on the NVIDIA's Jetson AGX platform, operating in full power mode. All our models, including the highest resolution, are real-time capable and can be deployed in a car. The primary advantage of a single-frame distance estimator is its broad applicability. Despite this, it comes at a cost when the continuous estimation of distances on image frames are often misaligned or discontinuous. To overcome this issue, we follow the approach from~\cite{Casser2019, Chen2019b, shu2020featdepth}, where we adapt the model in an online manner, mainly for practical autonomous systems. We train the model during inference by setting the batch size to 1. We feed in the inference image and its two adjacent frames, where we carry out the refinement as described in~\cite{Casser2019}. We do not implement any data augmentation techniques during this phase. With this technique, using a minimal temporal chain of frames (\ie three-frame snippets), the distance estimates enhance significantly, qualitatively, and quantitatively, as shown in Table~\ref{table:online-refine}. With a single frame's negligible delay, our SVDistNet framework can operate in real-time, even when using online refinement.
% -------------------------------------------------
\begin{table}[t]
\captionsetup{belowskip=-6pt, skip=4pt, font= small, singlelinecheck=false}
\centering
  \small
    \setlength{\tabcolsep}{0.2em}
    \begin{tabular}{lcccc}
    \toprule
    \textbf{Method} & \textit{Dataset} & 
    \multicolumn{1}{c}{\begin{tabular}[c]{@{}c@{}} \textit{Network} \\ \textit{Resolution} \end{tabular}} &
    \multicolumn{1}{c}{\begin{tabular}[c]{@{}c@{}} \textit{Encoder} \\ \textit{head} \end{tabular}} &
    \multicolumn{1}{c}{\begin{tabular}[c]{@{}c@{}} \textit{Inference} \\ \textit{(fps)} \end{tabular}} \\
    \toprule
    \multirow{3}{*}{\begin{tabular}[c]{@{}c@{}} FisheyeDistanceNet~\cite{kumar2020fisheyedistancenet}\end{tabular}}
      & K  & 640 x 192  & \multirow{3}{*}{\begin{tabular}[c]{@{}c@{}} ResNet-18\end{tabular}} & 84 \\
      & K  & 1024 x 320 &                                                                     & 34 \\
      & WS & 512 x 256  &                                                                     & 89 \\
    \midrule
    \multirow{3}{*}{\begin{tabular}[c]{@{}c@{}} UnrectDepthNet~\cite{kumar2020unrectdepthnet}\end{tabular}}
      & K  & 640 x 192  & \multirow{4}{*}{\begin{tabular}[c]{@{}c@{}} ResNet-50\end{tabular}} & 39 \\
      & K  & 1024 x 320 &                                                                     & 16 \\
      & WS & 512 x 256  &                                                                     & 42 \\
      & WS & 1024 x 512 &                                                                     & 11 \\
    \midrule  
    \multirow{4}{*}{\begin{tabular}[c]{@{}c@{}} SynDistNet~\cite{kumar2020syndistnet}\end{tabular}}
      & K  & 640 x 192  & \multirow{3}{*}{\begin{tabular}[c]{@{}c@{}} ResNet-18\end{tabular}} & 82 \\
      & K  & 1024 x 320 &                                                                     & 33 \\
      & WS & 512 x 256  &                                                                     & 91 \\
      & WS & 1024 x 512 &                                                                     & 23 \\
      & WS & 512 x 256  & ResNet50                                                            & 42 \\
      \midrule
    \multirow{4}{*}{\begin{tabular}[c]{@{}c@{}} SVDistNet \end{tabular}}
      & K  & 640 x 192  & \multirow{2}{*}{\begin{tabular}[c]{@{}c@{}} SAN-10\end{tabular}} & 80 \\
      & K  & 1024 x 320 &                                                                  & 30 \\
      & WS & 512 x 256  &                                                                  & 87 \\
      & WS & 512 x 256  & SAN-19                                                           & 45 \\
    \bottomrule
\end{tabular}
\caption{\textbf{Ablation study on inference time (frames per second)} using ONNX 16-bit float precision models on NVIDIA's Jetson AGX device of FisheyeDistanceNet~\cite{kumar2020fisheyedistancenet}, UnrectDepthNet~\cite{kumar2020unrectdepthnet}, SynDistNet \cite{kumar2020syndistnet} and SVDistNet on the KITTI (K) and WoodScape (WS) datasets.}
\label{table:inference-ablation}
\end{table} 
% -------------------------------------------------
\begin{table}[t!]
\captionsetup{belowskip=-10pt, skip=4pt, font= small, singlelinecheck=false}
\centering
\small
\begin{adjustbox}{width=\columnwidth}
\setlength{\tabcolsep}{0.1em}
  \begin{tabular}{lccccccc}
	\toprule
    \multirow{2}{*}{\textbf{Method}} &
    \cellcolor[HTML]{7d9ebf}Abs Rel & \cellcolor[HTML]{7d9ebf}Sq Rel & \cellcolor[HTML]{7d9ebf}RMSE & \cellcolor[HTML]{7d9ebf}RMSE$_{log}$ & \cellcolor[HTML]{e8715b}$\delta<1.25$ & \cellcolor[HTML]{e8715b}$\delta<1.25^2$ & \cellcolor[HTML]{e8715b}$\delta<1.25^3$ \\
    \cmidrule(lr){2-5} \cmidrule(lr){6-8}
    &  \multicolumn{4}{c}{\cellcolor[HTML]{7d9ebf}lower is better} & \multicolumn{3}{c}{\cellcolor[HTML]{e8715b}higher is better} \\
    \toprule
     SAN10-patch & 0.044 & 0.302 & 1.274 & 0.097 & 0.906 & 0.987 & 0.995 \\
     SAN10-pair  & 0.069 & 0.353 & 1.543 & 0.111 & 0.901 & 0.985 & 0.993 \\
     SAN19-patch & 0.034 & 0.264 & 1.218 & 0.073 & 0.914 & 0.992 & 0.996 \\
     SAN19-pair  & 0.065 & 0.322 & 1.545 & 0.092 & 0.896 & 0.988 & 0.995 \\
    \bottomrule
  \end{tabular}
\end{adjustbox}
\caption{\textbf{Online refinement} of the network's distance estimates incorporating~\cite{Casser2019}, where the model is trained during the inference as well on WoodScape dataset.~\cite{yogamani2019woodscape}.}
\label{table:online-refine}
\end{table}
\vspace{-1em}
% -------------------------------------------------
\subsection{\textbf{Robust loss function strategy}}

In Table~\ref{table:robust-ablation}, we ablate the impact of the robust loss function when compared with SynDistNet~\cite{kumar2020syndistnet}. From the results, we observe that the performance is significantly improved by using the adaptive $\alpha \in (0, 2)$ variant of the loss compared to a constant value for $\alpha$. The adaptive plan of action outperforms the fixed strategies, which showcases the importance of allowing the model to regulate the robustness of its loss by making $\alpha$ a free parameter which is optimized along with the network weights during training.\par
% -------------------------------------------------
\begin{table}[!t]
\captionsetup{belowskip=-6pt, skip=4pt, font= small, singlelinecheck=false}
\centering
  \small
  \begin{adjustbox}{width=\columnwidth}
    \setlength{\tabcolsep}{0.1em}
	  \begin{tabular}{llccccccc}
	    \toprule
        \multirow{2}{*}{\textbf{Method}}  & \multirow{2}{*}{$\alpha$} & \cellcolor[HTML]{7d9ebf}Abs Rel & \cellcolor[HTML]{7d9ebf}Sq Rel & \cellcolor[HTML]{7d9ebf}RMSE & \cellcolor[HTML]{7d9ebf}RMSE$_{log}$ & \cellcolor[HTML]{e8715b}$\delta<1.25$ & \cellcolor[HTML]{e8715b}$\delta<1.25^2$ & \cellcolor[HTML]{e8715b}$\delta<1.25^3$ \\
        \cmidrule(lr){3-6} \cmidrule(lr){7-9}
        & & \multicolumn{4}{c}{\cellcolor[HTML]{7d9ebf}lower is better} & \multicolumn{3}{c}{\cellcolor[HTML]{e8715b}higher is better} \\
	    \toprule
	    \multirow{2}{*}{\begin{tabular}[c]{@{}c@{}} SynDistNet \end{tabular}}   
	    & 2    & 0.154 & 0.631 & 2.532 & 0.198 & 0.832 & 0.965 & 0.981 \\
        & 0, 2 & 0.142 & 0.537 & 2.316 & 0.179 & 0.878 & 0.971 & 0.985 \\
        \midrule
        \multirow{2}{*}{\begin{tabular}[c]{@{}c@{}} SVDistNet \end{tabular}}       
        & 2    & 0.145 & 0.564 & 2.279 & 0.186 & 0.863 & 0.966 & 0.982 \\
        & 0, 2 & 0.128 & 0.469 & 2.153 & 0.164 & 0.875 & 0.974 & 0.986 \\
	   \bottomrule
    \end{tabular}
  \end{adjustbox}
\caption{\textbf{Impact of using the robust loss function} compared to the baseline from \cite{kumar2020syndistnet} on the Fisheye WoodScape dataset~\cite{yogamani2019woodscape}.}
%We witness significant performance gains when replacing the \lone loss with various variants of the robust loss function.}
\label{table:robust-ablation}
\end{table}

% -------------------------------------------------
\begin{table}[!t]
\centering
\begin{adjustbox}{width=\columnwidth}
\captionsetup{belowskip=-16pt, skip=4pt, font= small, singlelinecheck=false}
\begin{tabular}{@{}lcccc@{}}
\toprule
\multicolumn{1}{l}{\textbf{Method}} 
& \textit{\begin{tabular}[c]{@{}c@{}}No. of\\ Frames\end{tabular}} 
& \textit{GT} 
& \cellcolor[HTML]{7d9ebf}\textit{Sequence 09} 
& \cellcolor[HTML]{e8715b}\textit{Sequence 10} \\ 
\midrule
    ORB-SLAM~\cite{mur2015orb}                   & 5 & \ch & 0.014 $\pm$ 0.008 & 0.012 $\pm$ 0.011 \\
    DF-Net~\cite{zou2018df}                      & 5 & \ch & 0.017 $\pm$ 0.007 & 0.015 $\pm$ 0.009 \\
    SfMLearner~\cite{zhou2017unsupervised}       & 5 & \ch & 0.016 $\pm$ 0.009 & 0.013 $\pm$ 0.009 \\
    Klodt et al.~\cite{klodt2018supervising}     & 5 & \ch & 0.014 $\pm$ 0.007 & 0.013 $\pm$ 0.009 \\
    GeoNet~\cite{Yin2018}                        & 5 & \ch & 0.012 $\pm$ 0.007 & 0.012 $\pm$ 0.009 \\
    Struct2Depth~\cite{Casser2019}               & 5 & \ch & 0.011 $\pm$ 0.006 & 0.011 $\pm$ 0.010 \\
    Ranjan~\cite{Ranjan2019}                     & 5 & \ch & 0.011 $\pm$ 0.006 & 0.011 $\pm$ 0.010 \\ 
    PackNet-SfM~\cite{Guizilini2020a}            & 5 & \ch & 0.010 $\pm$ 0.005 & 0.009 $\pm$ 0.008 \\
    PackNet-SfM~\cite{Guizilini2020a}            & 5 & \xm & 0.014 $\pm$ 0.007 & 0.012 $\pm$ 0.008 \\
    SVDistNet                                      & 5 & \ch & \textbf{0.009} $\pm$ \textbf{0.004} & 0.008 $\pm$ \textbf{0.005} \\
    SVDistNet                                      & 5 & \xm & 0.010 $\pm$ 0.005 & 0.010 $\pm$ 0.008 \\
    \midrule
    DDVO~\cite{Wang2018e}                        & 3 & \ch & 0.045 $\pm$ 0.108 & 0.033 $\pm$ 0.074 \\
    Vid2Depth~\cite{mahjourian2018unsupervised}  & 3 & \ch & 0.013 $\pm$ 0.010 & 0.012 $\pm$ 0.011 \\
    EPC++~\cite{Luo2019a}                        & 3 & \ch & 0.013 $\pm$ 0.007 & 0.012 $\pm$ 0.008 \\
    SVDistNet                                      & 3 & \ch & \textbf{0.011} $\pm$ \textbf{0.006} & \textbf{0.010} $\pm$ \textbf{0.007} \\
    SVDistNet                                      & 3 & \xm & 0.012 $\pm$ 0.007 & 0.011 $\pm$ 0.008 \\
    \midrule
    Monodepth2~\cite{Godard2019}                   & 2 & \ch & 0.017 $\pm$ 0.008 & 0.015 $\pm$ 0.010 \\
    SVDistNet                                      & 2 & \ch & \textbf{0.015} $\pm$ \textbf{0.007} & \textbf{0.013} $\pm$ \textbf{0.007} \\
    SVDistNet                                      & 2 & \xm & 0.016 $\pm$ 0.008 & 0.014 $\pm$ 0.009 \\
    \bottomrule
    \end{tabular}
  \end{adjustbox}
\caption{\textbf{Evaluation of the pose estimation} on the KITTI Odometry Benchmark~\cite{geiger2013vision}.}
\label{table:supplementary-pose-ate}
\vspace{-2em}
\end{table}

% -------------------------------------------------
\subsection{\textbf{Pose Estimation Results}}

The PoseNet is an ego-motion predictor consisting of a SAN10-patch encoder. We apply the Siamese (twin network) notion where we feed $I_t$ and $I_t'$ individually to a shared self-attention encoder and concatenate the output features from the twin network before feeding it to the pose decoder as shown in Fig.~\ref{fig:mtl_pipeline} predicting a relative pose between the images. Compared to our previous works~\cite{kumar2020fisheyedistancenet, kumar2020syndistnet, kumar2020unrectdepthnet}, where we used Euler angles, we chose quaternions to represent the 3D rotation. The design choice is mainly due to its continuous and smooth representation of rotation, smaller memory footprint than rotation matrices and they are much more efficient than both matrix, and angle/axis representations used in~\cite{Godard2019, shu2020featdepth}.\par 
In Table~\ref{table:supplementary-pose-ate}, we report the average trajectory error (ATE) in meters, where we train our method on sequences 00-08 and evaluate on Sequences 09 and 10, the same as the baseline methods. For evaluation, we follow the evaluation protocol defined in~\cite{zhou2017unsupervised}. Note that all the methods except our SVDistNet and PackNet-SfM utilize ground-truth at test-time to scale the prediction for a scale consistent result. We predict independent transformations for each of the four frame-to-frame transformations belonging to the five-frames set to evaluate our two-frame ego-motion model on the five-frame test sequences. We combine these different transformations to form local trajectories. We outperform the previous methods listed in Table~\ref{table:supplementary-pose-ate}, mainly by applying our bundle adjustment framework inflicted by our cross-sequence distance consistency loss~\cite{kumar2020fisheyedistancenet} induces more constraints and simultaneously optimizes distances and camera pose for an implicitly extended training input sequence. This provides additional consistency constraints that are not induced by previous methods.\par
% -------------------------------------------------
\begin{table*}[htpb]
\centering
\captionsetup{belowskip=-12pt, font= small, singlelinecheck=false}
\scalebox{1.25}{
\begin{tabular}{ll}
\toprule
$\textbf{Abs Rel}: \frac{1}{|N|}\sum_{i\in N}\frac{\mid d_{i}-d_{i}^{*}\mid}{d_{i}^{*}}$
&$\textbf{RMSE}:\sqrt{\frac{1}{|N|}\sum_{i\in N}\parallel d_{i}-d_{i}^{*} \parallel^{2}}$\\
$\textbf{Sq Rel}:\frac{1}{|N|}\sum_{i\in N}\frac{\parallel d_{i}-d_{i}^{*}\parallel^{2}}{d_{i}^{*}}$
&$\textbf{RMSE log}: \sqrt{\frac{1}{|N|}\sum_{i\in N}\parallel \log (d_{i})- \log (d_{i}^{*}) \parallel^{2}}$ \\
\multicolumn{2}{l}{\textbf{Accuracies} $\mathbf{\delta}_\mathbf{t}:
\frac{1}{|N|}|\{d \in N| \: \max(\frac{d_{i}}{d_{i}^{*}}, \frac{d_{i}^{*}}{d_{i}}) \: < 1.25^t\}|\times 100\%$} \\
\bottomrule
\end{tabular}
}
\caption{Performance indicators for depth evaluation. where $d_{i}$ and  $d_{i}^{*}$ denotes the predicted and ground truth depth value of pixel $i$ respectively. $N$ denotes the set of a total number of pixels with real-depth/distance values in an image, $|.|$ returns the number of the input set elements.}
\end{table*}
% -------------------------------------------------
\begin{table*}[!ht]
\captionsetup{belowskip=-12pt, font= small, singlelinecheck=false}

\centering
{
\small
\setlength{\tabcolsep}{0.3em}
\begin{tabular}{c|llccccccc}
\toprule
& \multirow{2}{*}{\textbf{Method}}
& Train
& \cellcolor[HTML]{7d9ebf}Abs Rel & \cellcolor[HTML]{7d9ebf}Sq Rel & \cellcolor[HTML]{7d9ebf}RMSE & \cellcolor[HTML]{7d9ebf}RMSE$_{log}$ & \cellcolor[HTML]{e8715b}$\delta<1.25$ & \cellcolor[HTML]{e8715b}$\delta<1.25^2$ & \cellcolor[HTML]{e8715b}$\delta<1.25^3$ \\
\cmidrule(lr){4-7} \cmidrule(lr){8-10}
& & & \multicolumn{4}{c}{\cellcolor[HTML]{7d9ebf}lower is better} & \multicolumn{3}{c}{\cellcolor[HTML]{e8715b}higher is better} \\
\toprule
\parbox[t]{2mm}{\multirow{33}{*}{\rotatebox[origin=c]{90}{Original~\cite{Eigen_14}}}}
& SfMLearner~\cite{zhou2017unsupervised}      & M & 0.208 & 1.768 & 6.958 & 0.283 & 0.678 & 0.885 & 0.957 \\
& DNC~\cite{yang2017unsupervised}             & M & 0.182 & 1.481 & 6.501 & 0.267 & 0.725 & 0.906 & 0.963 \\
& Vid2Depth~\cite{mahjourian2018unsupervised} & M & 0.163 & 1.240 & 6.220 & 0.250 & 0.762 & 0.916 & 0.968 \\
& LEGO~\cite{yang2018lego}                    & M & 0.162 & 1.352 & 6.276 & 0.252 & 0.783 & 0.921 & 0.969 \\
& Kumar~\cite{Kumar2018a}                & M & 0.211 & 1.979 & 6.154 & 0.263 & 0.731 & 0.897 & 0.959 \\
& Wang \etal~\cite{wang2019unsupervised}      & M & 0.158 & 1.277 & 5.858 & 0.233 & 0.785 & 0.929 & 0.973 \\
& GeoNet~\cite{Yin2018}                       & M & 0.155 & 1.296 & 5.857 & 0.233 & 0.793 & 0.931 & 0.973 \\
& Cycle-SfM~\cite{sun2019cycle}               & M & 0.162 & 1.349 & 5.847 & 0.239 & 0.784 & 0.925 & 0.969 \\
& Li \etal~\cite{li2019sequential}            & M & 0.150 & 1.127 & 5.564 & 0.229 & 0.823 & 0.936 & 0.974 \\
& DDVO~\cite{Wang2018e}                & M & 0.151 & 1.257 & 5.583 & 0.228 & 0.810 & 0.936 & 0.974 \\
& DF-Net~\cite{zou2018df}                     & M & 0.150 & 1.124 & 5.507 & 0.223 & 0.806 & 0.933 & 0.973 \\
& GANVO~\cite{almalioglu2019ganvo}            & M & 0.150 & 1.141 & 5.448 & 0.216 & 0.808 & 0.939 & 0.975 \\
& Bian~\cite{bian2019unsupervised}            & M & 0.137 & 1.089 & 5.439 & 0.217 & 0.830 & 0.942 & 0.975 \\
& EPC++~\cite{Yang2018c}                      & M & 0.141 & 1.029 & 5.350 & 0.216 & 0.816 & 0.941 & 0.976 \\
& CC~\cite{Ranjan2019}             & M & 0.140 & 1.070 & 5.326 & 0.217 & 0.826 & 0.941 & 0.975 \\
& Struct2Depth~\cite{Casser2019}              & M & 0.141 & 1.036 & 5.291 & 0.215 & 0.816 & 0.945 & 0.979 \\
& LearnK~\cite{Gordon2019}                    & M & 0.128 & 0.959 & 5.230 & 0.212 & 0.845 & 0.947 & 0.976 \\
& SIGNet~\cite{Meng2019a}                & M & 0.133 & 0.905 & 5.181 & 0.208 & 0.825 & 0.947 & 0.981 \\
& DualNet~\cite{Zhou2019}                     & M & 0.121 & 0.837 & 4.945 & 0.197 & 0.853 & 0.955 & 0.982 \\
& OmegaNet~\cite{tosi2020distilled}           & M & 0.126 & 0.835 & 4.937 & 0.199 & 0.844 & 0.953 & 0.982 \\
& SuperDepth~\cite{pillai2019superdepth}      & M & 0.116 & 1.055 & -     & 0.209 & 0.853 & 0.948 & 0.977 \\
& Monodepth2~\cite{Godard2019}                & M & 0.115 & 0.903 & 4.863 & 0.193 & 0.877 & 0.959 & 0.981 \\
& PackNet-SfM~\cite{Guizilini2020a}           & M & 0.111 & 0.829 & 4.788 & 0.199 & 0.864 & 0.954 & 0.980 \\
& FisheyeDistanceNet~\cite{kumar2020fisheyedistancenet} & M & 0.117 & 0.867 & 4.739 & 0.190 & 0.869 & 0.960 & 0.982 \\
& SGDepth~\cite{Klingner2020}                 & M & 0.113 & 0.880 & 4.695 & 0.192 & 0.884 & 0.961 & 0.981 \\
& Patil \etal~\cite{patil2020don}             & M & 0.111 & 0.821 & 4.650 & 0.187 & 0.883 & 0.961 & 0.982 \\
& UnRectDepthNet~\cite{kumar2020unrectdepthnet} & M & 0.107 & 0.721 & 4.564 & 0.178 & 0.894 & 0.971 & 0.986 \\
& SynDistNet~\cite{kumar2020syndistnet}       & M & 0.109 & 0.718 & 4.516 & 0.180 & 0.896 & 0.973 & 0.986 \\
& Shu \etal~\cite{shu2020featdepth}           & M & 0.104 & 0.729 & 4.481 & 0.179 & 0.893 & 0.965 & 0.984 \\
& \textbf{SVDistNet}                          & M & \textbf{0.102} & \textbf{0.706} & \textbf{4.459} & \textbf{0.172} & \textbf{0.908} & \textbf{0.974} & \textbf{0.986} \\
\cmidrule{2-10}
& Struct2Depth~\cite{Casser2019}             & M${^*}$ & 0.109 & 0.825 & 4.750 & 0.187 &0.874 & 0.958 & 0.983 \\
& GLNet~\cite{Chen2019b}                  & M$^{*}$ & 0.099 & 0.796 & 4.743 & 0.186 &0.884 & 0.955 & 0.979 \\
& Shu \etal~\cite{shu2020featdepth}          & M$^{*}$ & 0.088 & 0.712 & 4.137 & \textbf{0.169} & 0.915 & 0.965 & 0.982 \\
& \textbf{SVDistNet}                         & M${^*}$ & \textbf{0.086} & \textbf{0.701} & \textbf{4.118} & 0.170 & \textbf{0.919} & \textbf{0.976} & \textbf{0.985} \\
\midrule
\parbox[t]{2mm}{\multirow{11}{*}{\rotatebox[origin=c]{90}{Improved~\cite{uhrig2017sparsity}}}}
& SfMLearner~\cite{zhou2017unsupervised}    & M & 0.176 & 1.532 & 6.129 & 0.244 & 0.758 & 0.921 & 0.971 \\
& Vid2Depth~\cite{mahjourian2018unsupervised} & M & 0.134 & 0.983 & 5.501 & 0.203 & 0.827 & 0.944 & 0.981 \\
& GeoNet~\cite{Yin2018}                     & M & 0.132 & 0.994 & 5.240 & 0.193 & 0.883 & 0.953 & 0.985 \\
& DDVO~\cite{Wang2018e}              & M & 0.126 & 0.866 & 4.932 & 0.185 & 0.851 & 0.958 & 0.986 \\
& EPC++~\cite{Yang2018c}                    & M & 0.120 & 0.789 & 4.755 & 0.177 & 0.856 & 0.961 & 0.987 \\
& Monodepth2~\cite{Godard2019}              & M & 0.090 & 0.545 & 3.942 & 0.137 & 0.914 & 0.983 & 0.995 \\
& PackNet-SfM~\cite{Guizilini2020a}         & M & 0.078 & 0.420 & 3.485 & 0.121 & 0.931 & 0.986 & 0.996 \\
& UnRectDepthNet~\cite{kumar2020unrectdepthnet} & M & 0.081 & 0.414 & 3.412 & 0.117 & 0.926 & 0.987 & 0.996 \\
& SynDistNet~\cite{kumar2020syndistnet}     & M & 0.076 & 0.412 & 3.406 & 0.115 & 0.931 & 0.988 & 0.996 \\
& \textbf{SVDistNet}                        & M & \textbf{0.071} & \textbf{0.405} & \textbf{3.345} & \textbf{0.106} & \textbf{0.934} & \textbf{0.988} & \textbf{0.996} \\
& \textbf{SVDistNet}                        & M${^*}$ & \textbf{0.059} & \textbf{0.392} & \textbf{3.206} & \textbf{0.097} & \textbf{0.935} & \textbf{0.989} & \textbf{0.995} \\
\bottomrule
\end{tabular}
}
\caption{\textbf{Evaluation of the KITTI Eigen split} compared to most of the previous self-supervised monocular depth estimation methods. Following best practices, we cap depths at 80\,m. We also evaluate using the \textit{Original} depth maps generated from raw point clouds as proposed by \cite{Eigen_14} as well as \textit{Improved} annotated depth maps as introduced by \cite{uhrig2017sparsity}. M indicates that sequences are trained on using the monocular approach. M${^*}$ indicates the online refinement technique~\cite{Casser2019}, where the model is trained during the inference. Note that while most approaches use median scaling concerning the ground truth at test-time for a scale-consistent prediction, we do not need to use this scaling method.}
\label{tab:kitti-monocular-results}
\end{table*}
% -------------------------------------------------
\begin{figure*}[!ht]
\captionsetup{singlelinecheck=false, justification=raggedright, font=small}
  \centering
  \resizebox{\textwidth}{!}{
  \newcommand{\turnheightnew}{0.25\columnwidth}
\centering
\setlength{\extrarowheight}{-0.5pt}
\begin{tabular}{@{\hskip 0.4mm}c@{\hskip 0.4mm}c@{\hskip 0.4mm}c@{\hskip 0.4mm}c@{\hskip 0.4mm}c@{\hskip 0.4mm}}

{\rotatebox{90}{\hspace{0mm}}} &
\includegraphics[height=\turnheightnew]{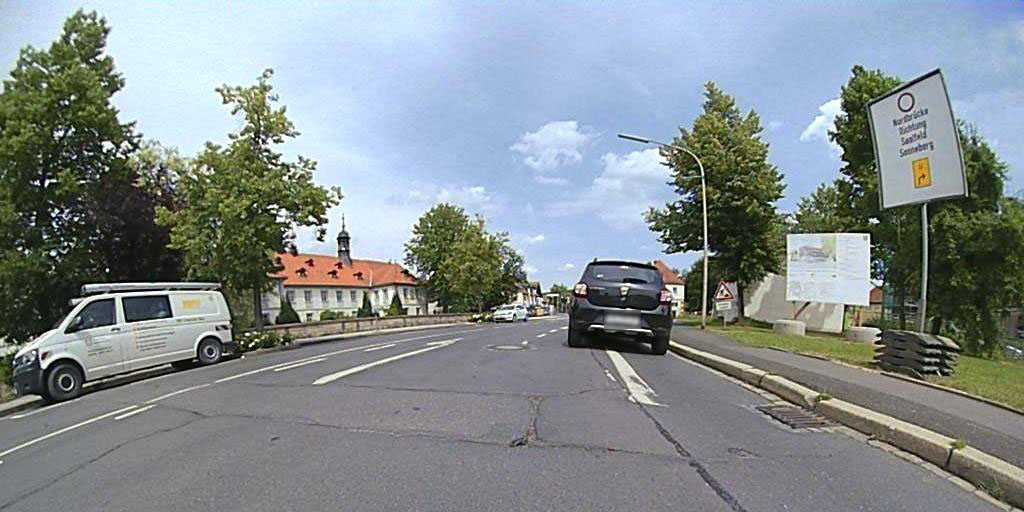} &
\includegraphics[height=\turnheightnew]{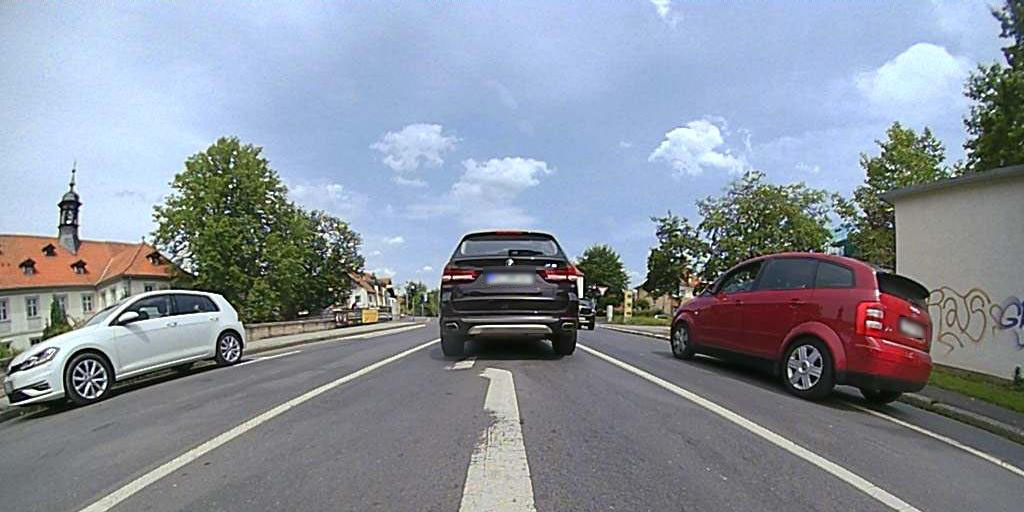} &
\includegraphics[height=\turnheightnew]{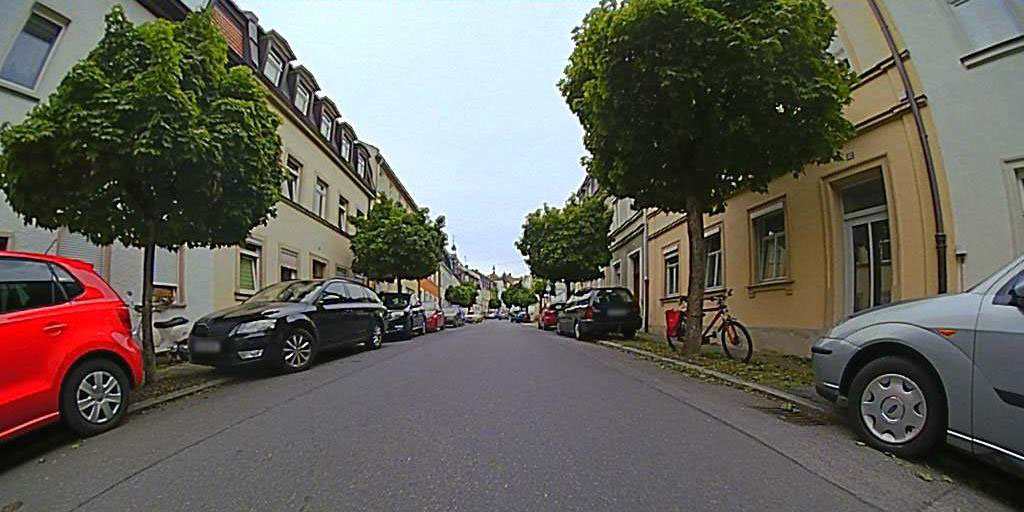} &
\includegraphics[height=\turnheightnew]{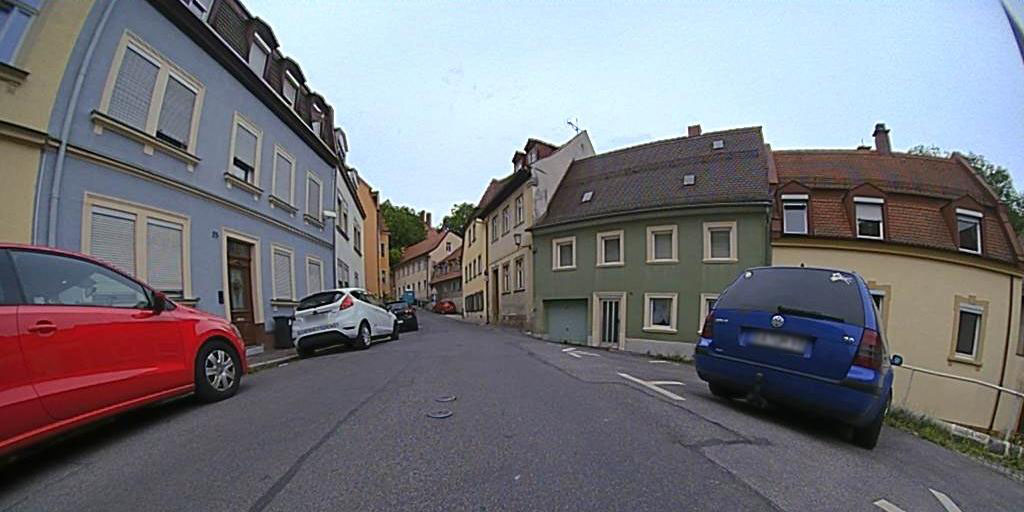}\\

{\rotatebox{90}{\hspace{0mm}}} &
\includegraphics[height=\turnheightnew]{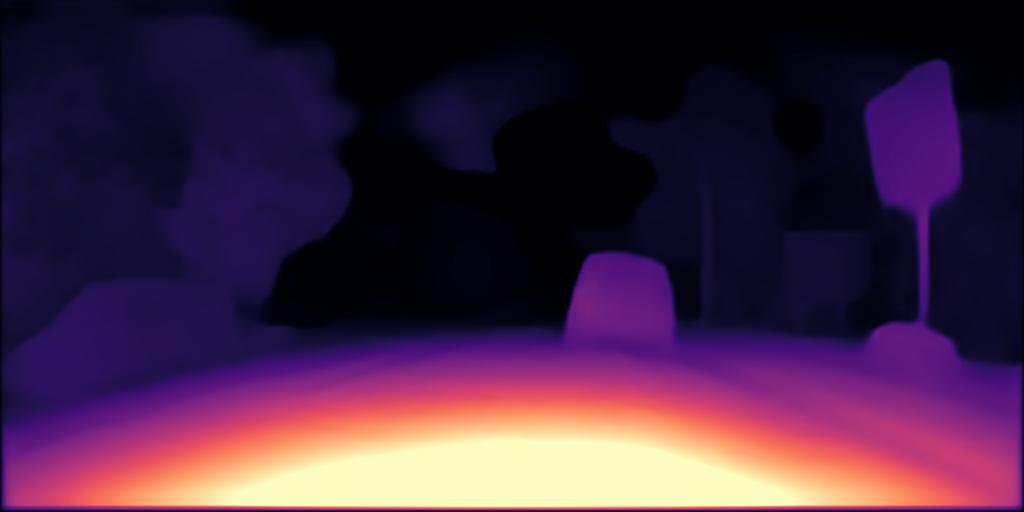} &
\includegraphics[height=\turnheightnew]{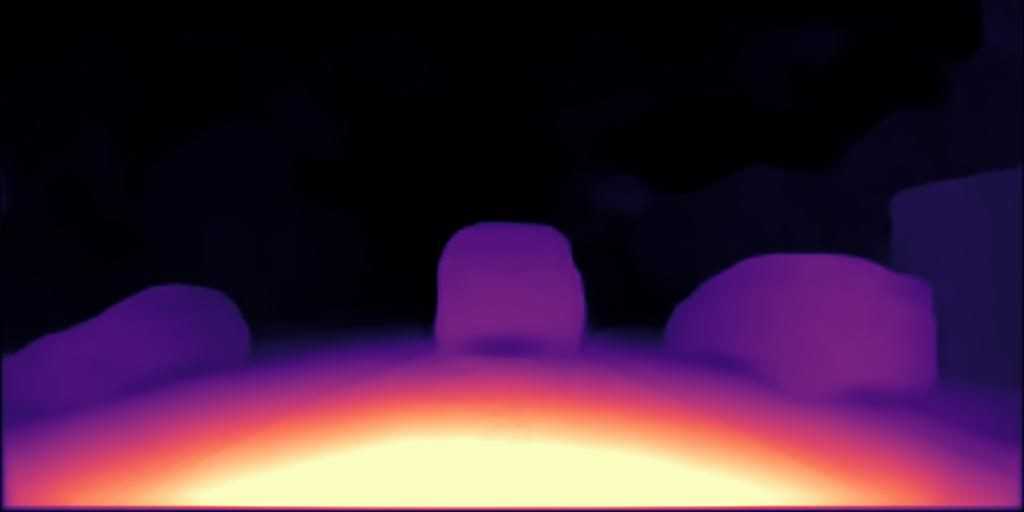} &
\includegraphics[height=\turnheightnew]{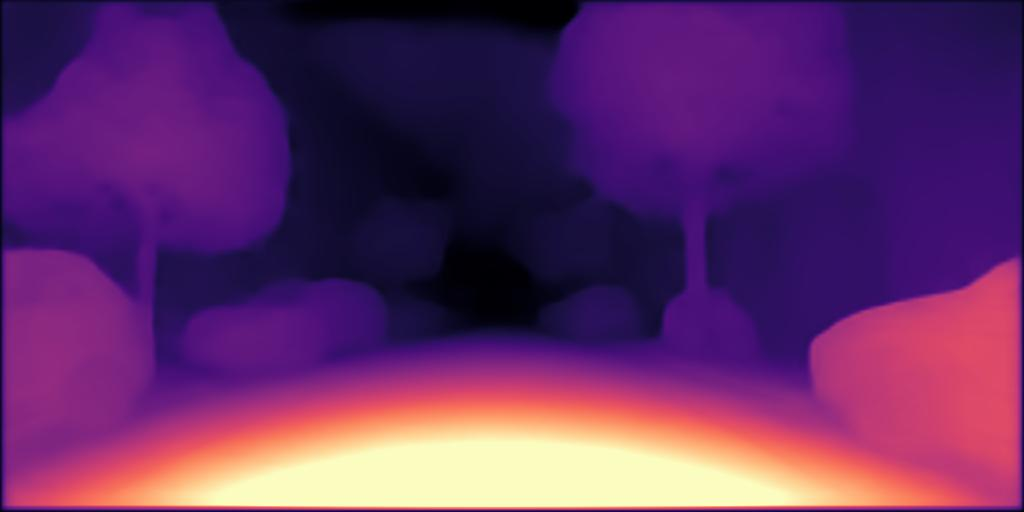} &
\includegraphics[height=\turnheightnew]{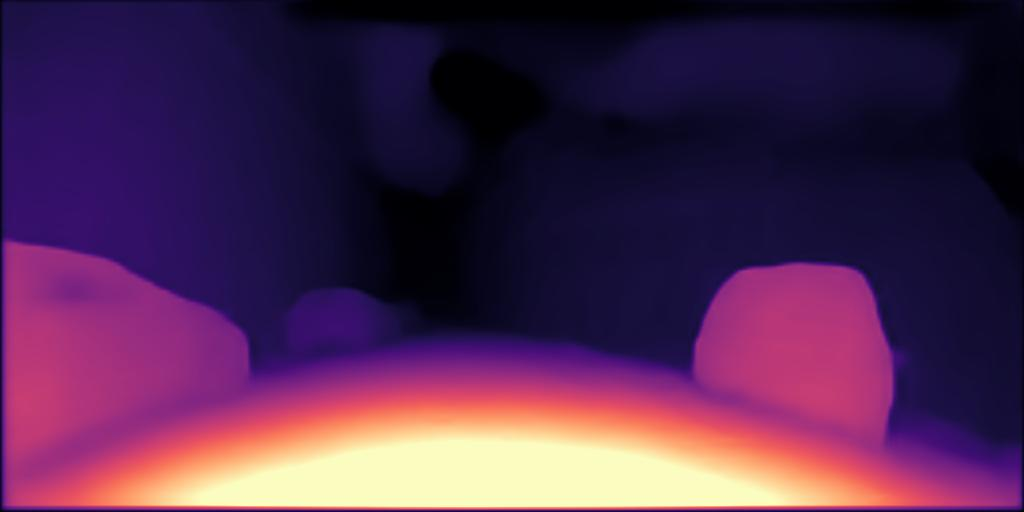}\\

% Distortion
{\rotatebox{90}{\hspace{0mm}\scriptsize}} &
\includegraphics[height=\turnheightnew]{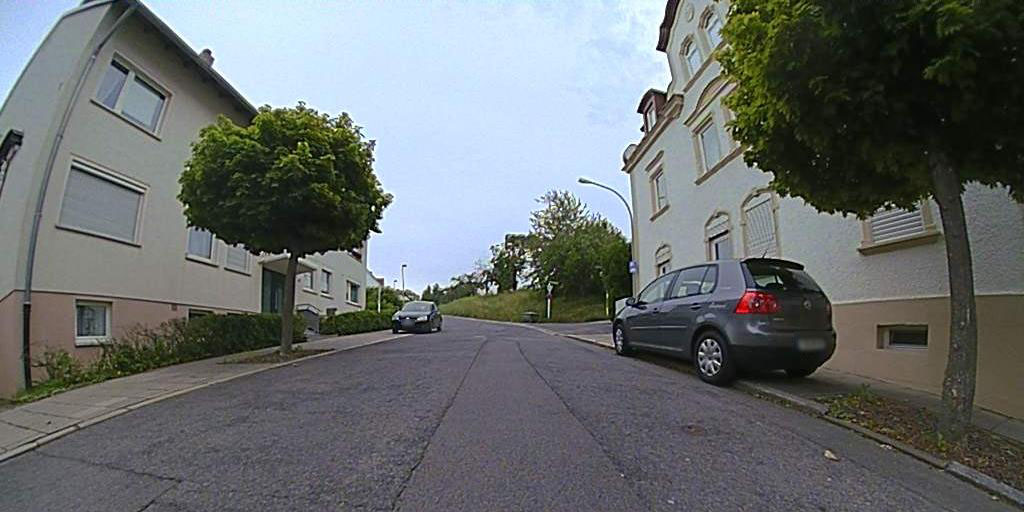} &
\includegraphics[height=\turnheightnew]{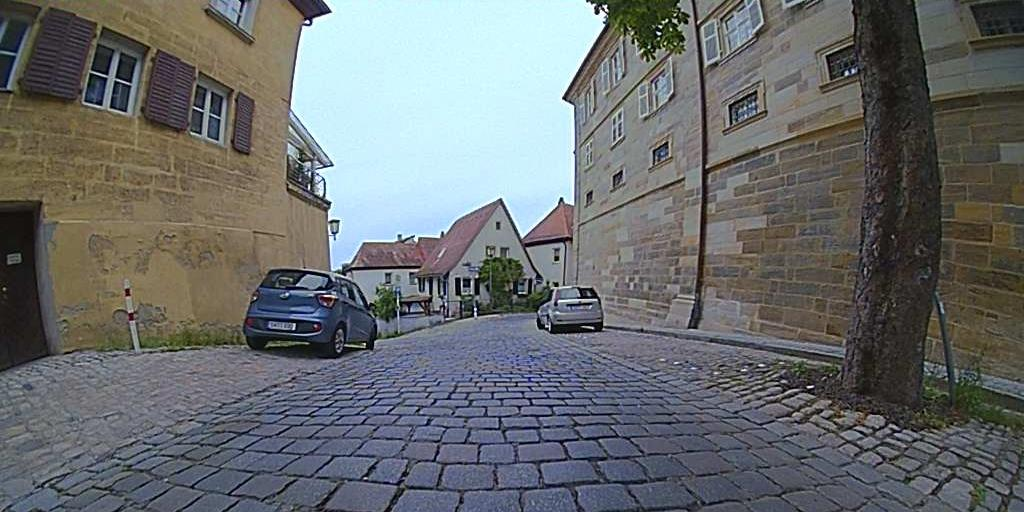} &
\includegraphics[height=\turnheightnew]{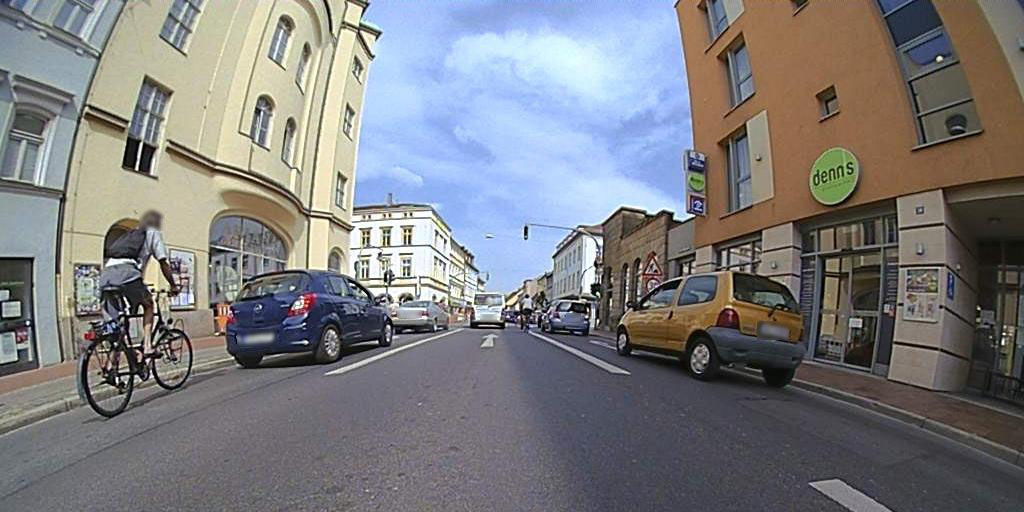} &
\includegraphics[height=\turnheightnew]{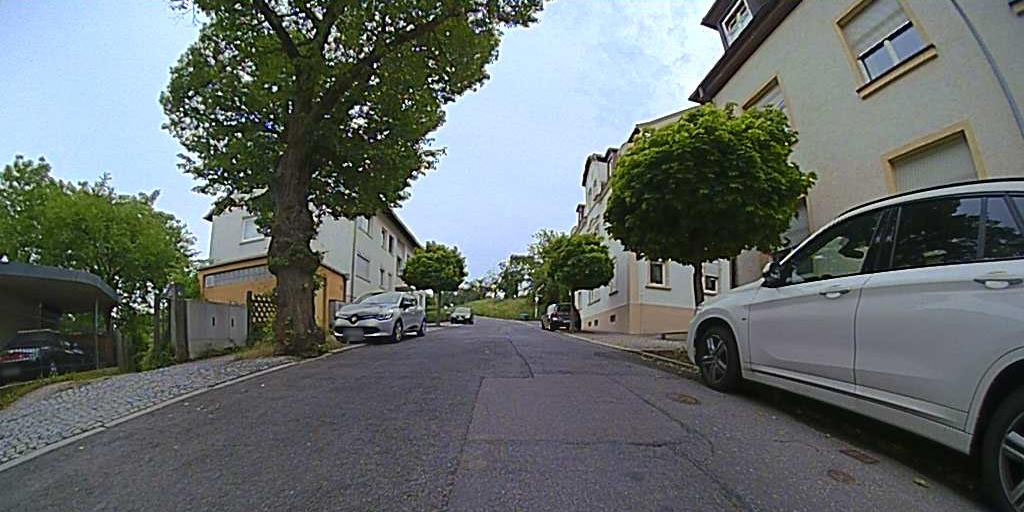} \\

{\rotatebox{90}{\hspace{0mm}\scriptsize}} &
\includegraphics[height=\turnheightnew]{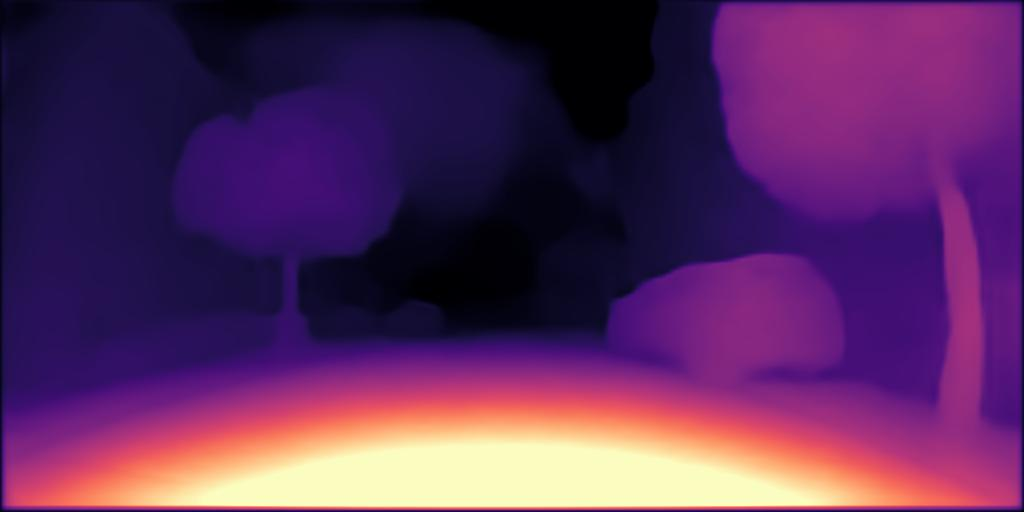} &
\includegraphics[height=\turnheightnew]{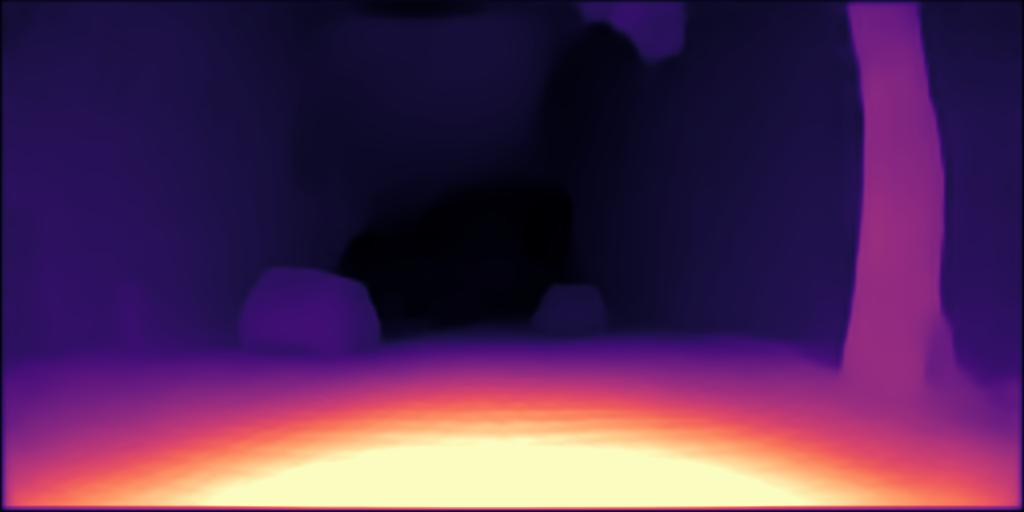} &
\includegraphics[height=\turnheightnew]{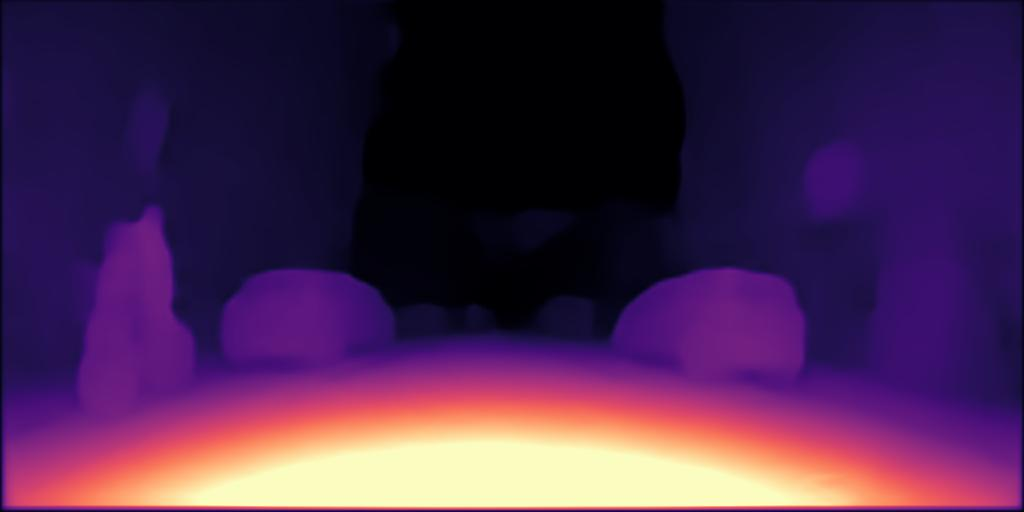} &
\includegraphics[height=\turnheightnew]{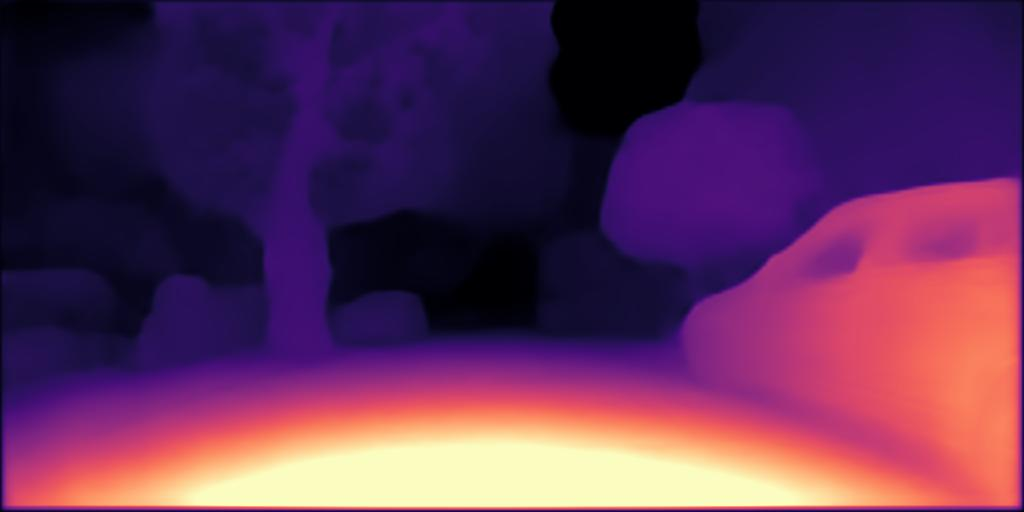} \\

% Sharp Edges
{\rotatebox{90}{\hspace{0mm}\scriptsize}} &
\includegraphics[height=\turnheightnew]{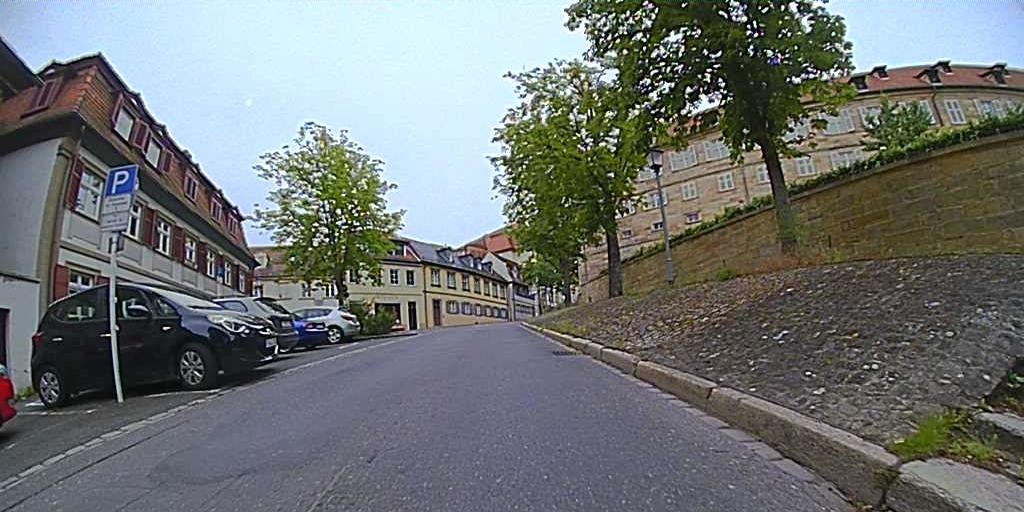} &
\includegraphics[height=\turnheightnew]{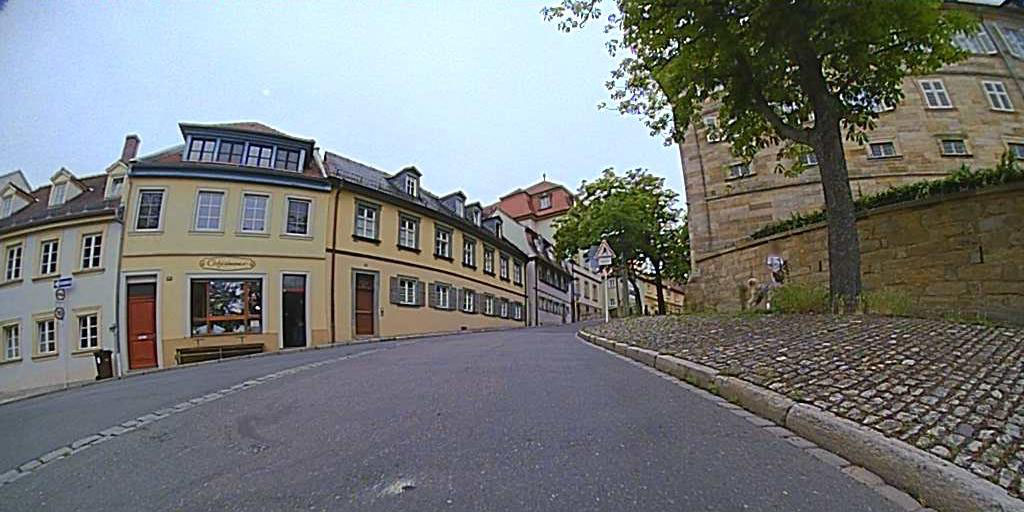} &
\includegraphics[height=\turnheightnew]{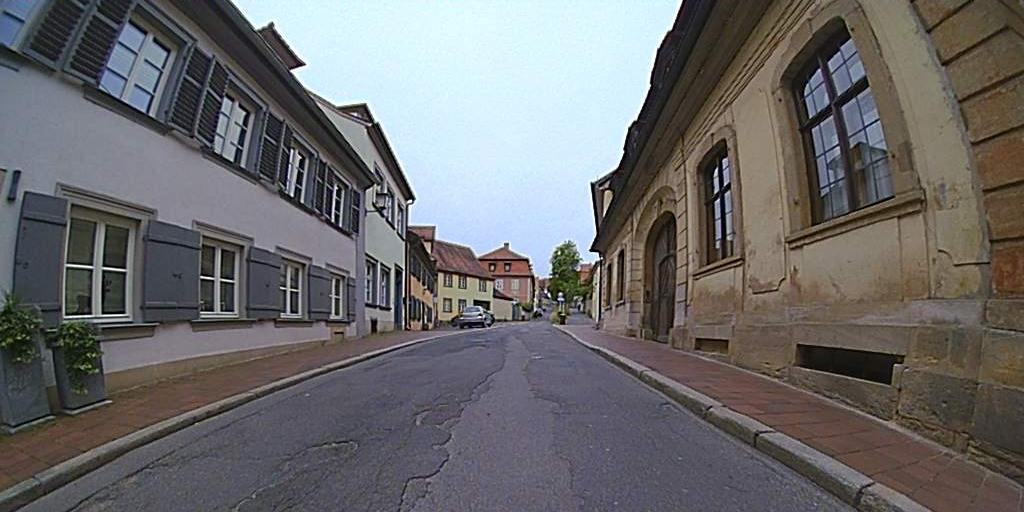} &
\includegraphics[height=\turnheightnew]{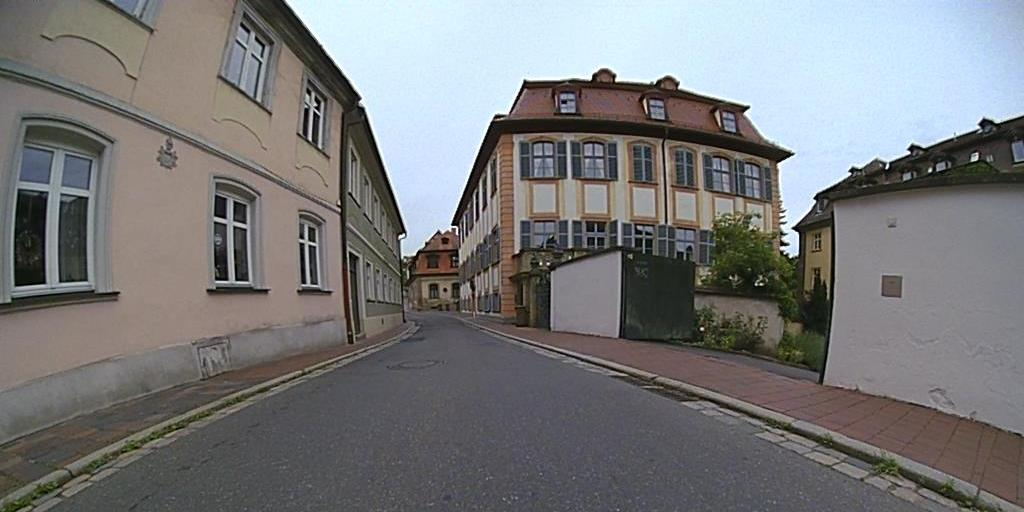} \\

{\rotatebox{90}{\hspace{0mm}\scriptsize}} &
\includegraphics[height=\turnheightnew]{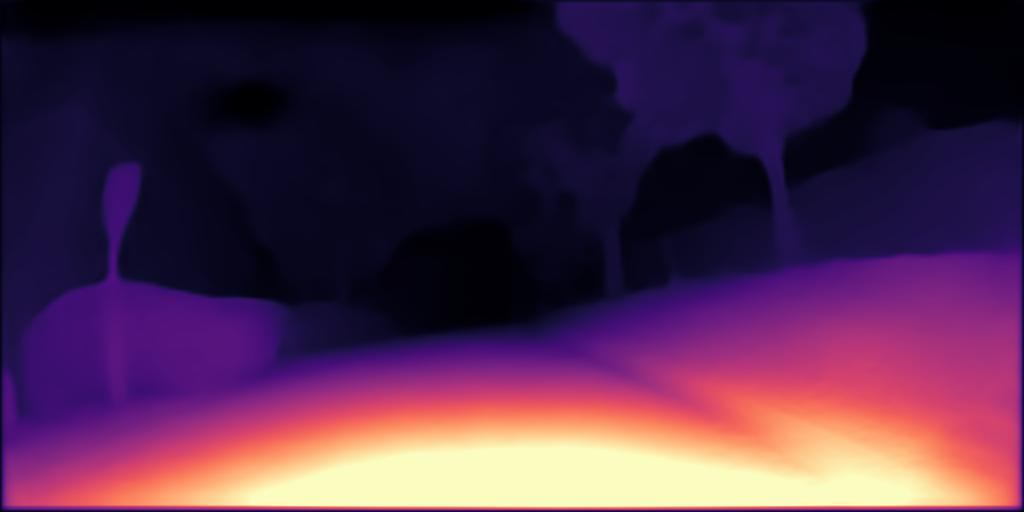} &
\includegraphics[height=\turnheightnew]{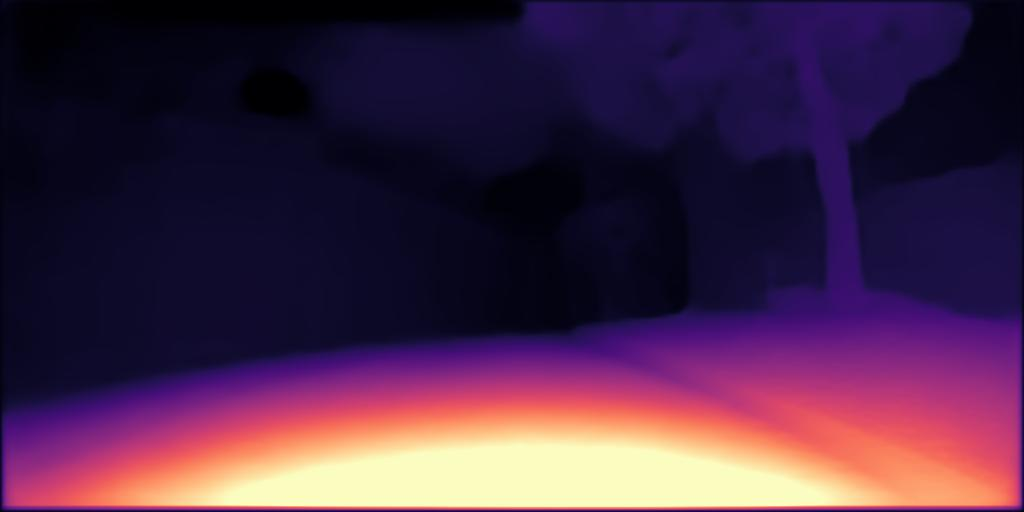} &
\includegraphics[height=\turnheightnew]{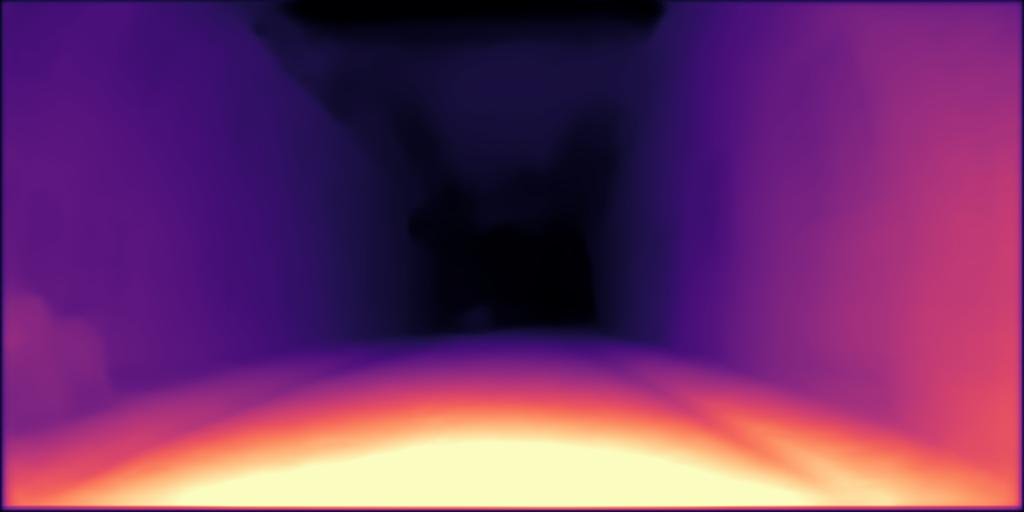} &
\includegraphics[height=\turnheightnew]{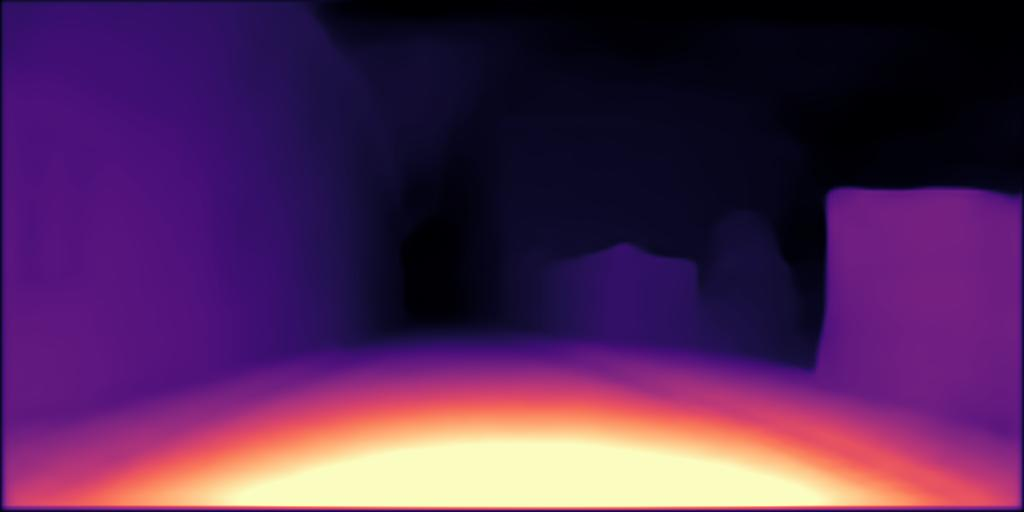} \\

% Tunnel
{\rotatebox{90}{\hspace{0mm}\scriptsize}} &
\includegraphics[height=\turnheightnew]{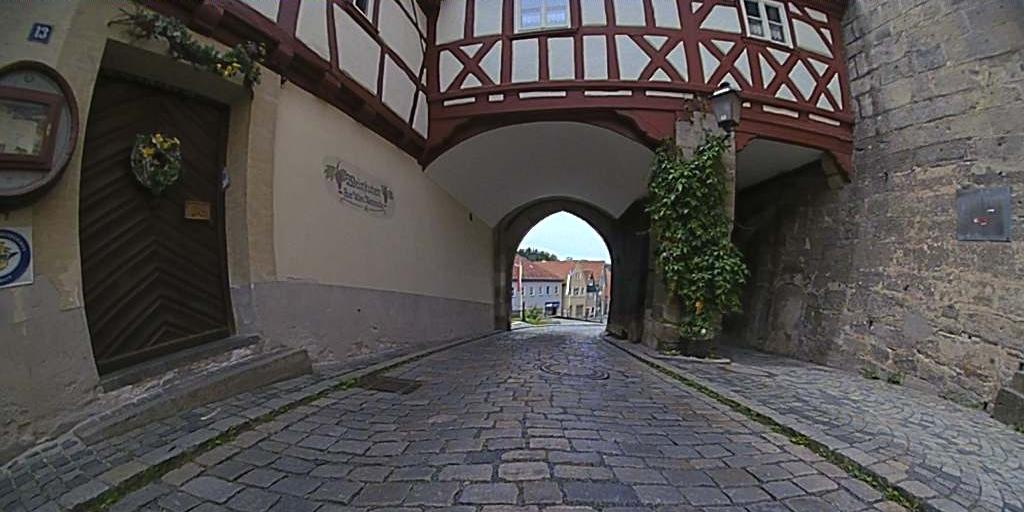} &
\includegraphics[height=\turnheightnew]{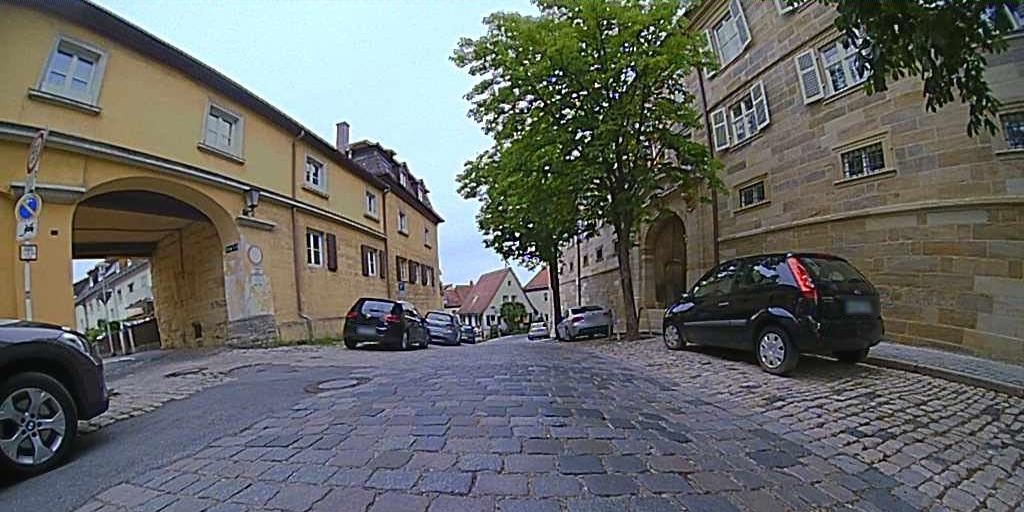} &
\includegraphics[height=\turnheightnew]{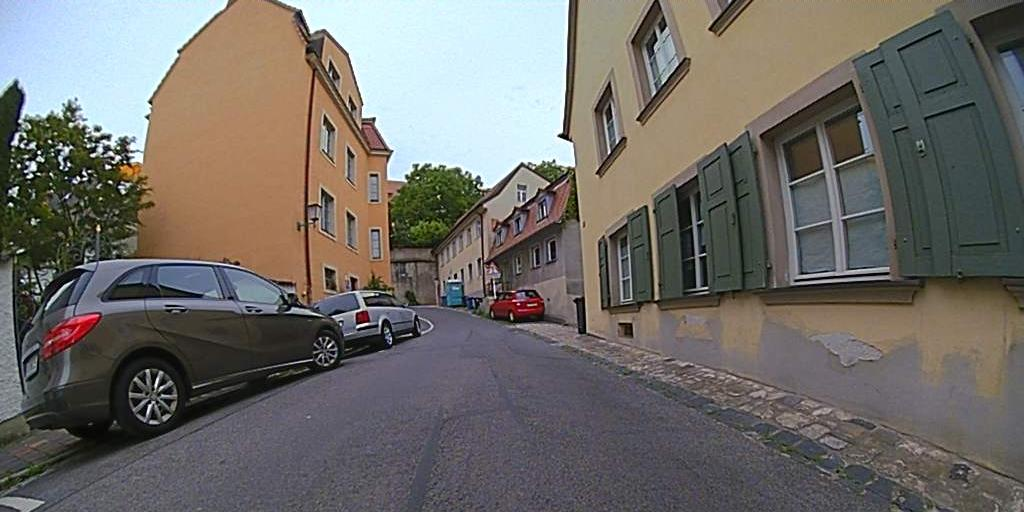} &
\includegraphics[height=\turnheightnew]{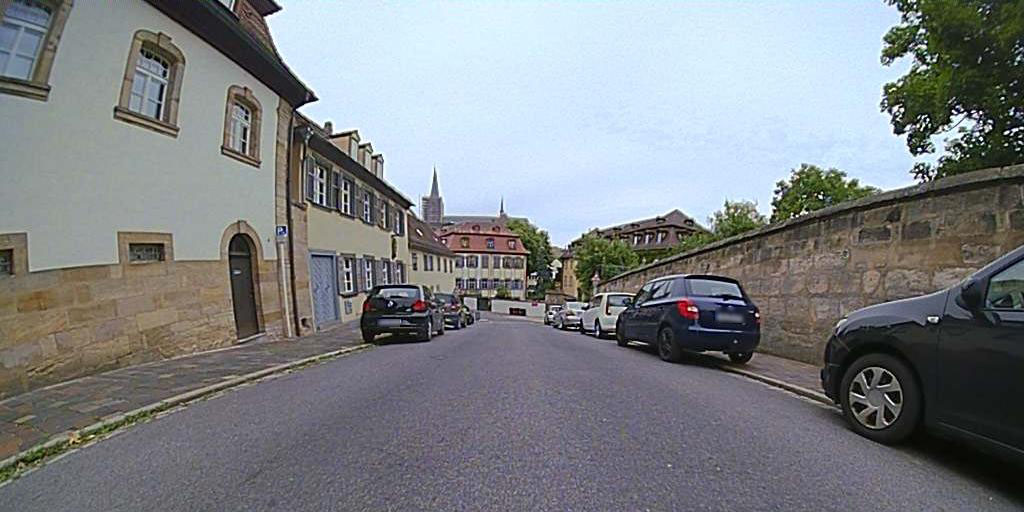} \\

{\rotatebox{90}{\hspace{0mm}\scriptsize}} &
\includegraphics[height=\turnheightnew]{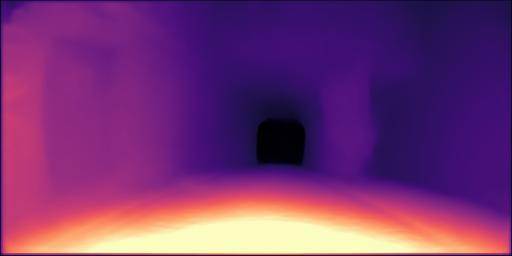} &
\includegraphics[height=\turnheightnew]{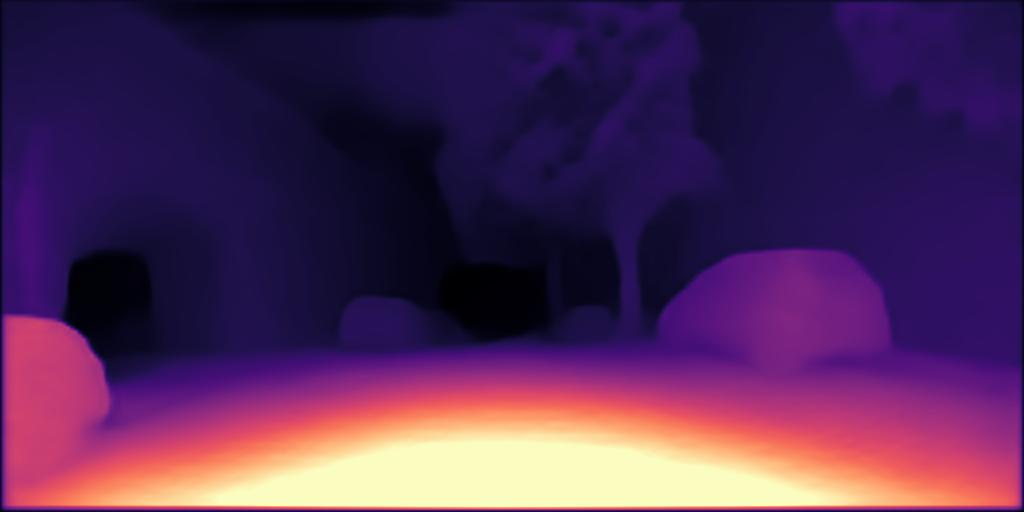} &
\includegraphics[height=\turnheightnew]{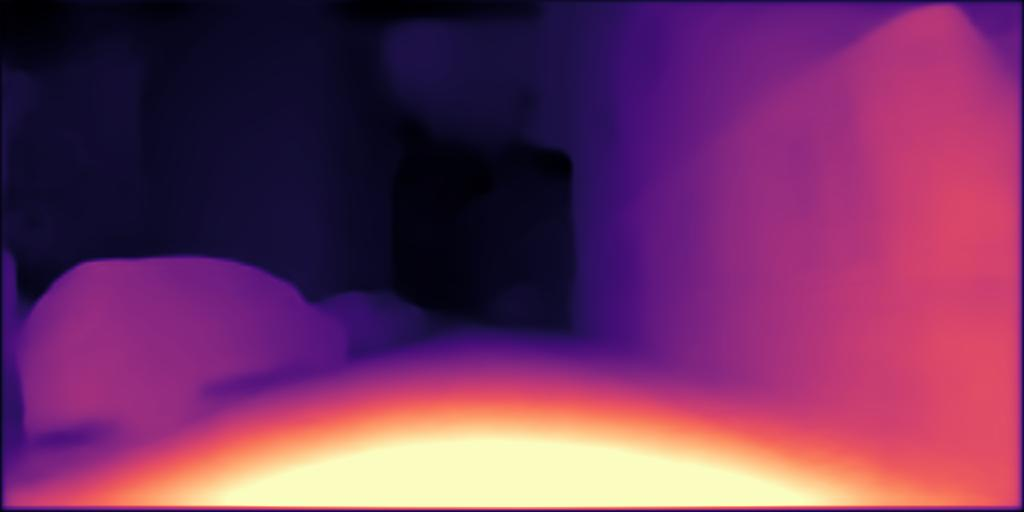} &
\includegraphics[height=\turnheightnew]{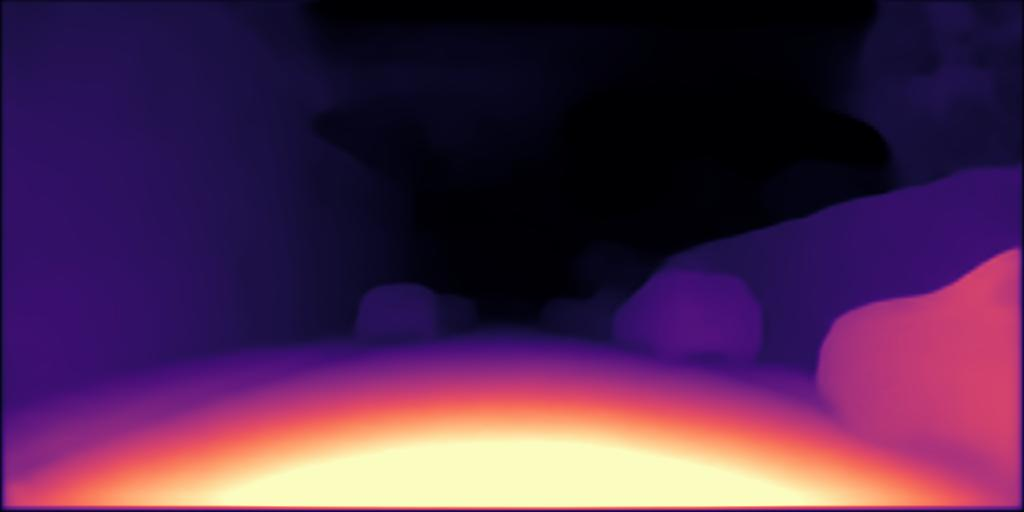} \\

%560 is left out
% Sharp
{\rotatebox{90}{\hspace{0mm}\scriptsize}} &
\includegraphics[height=\turnheightnew]{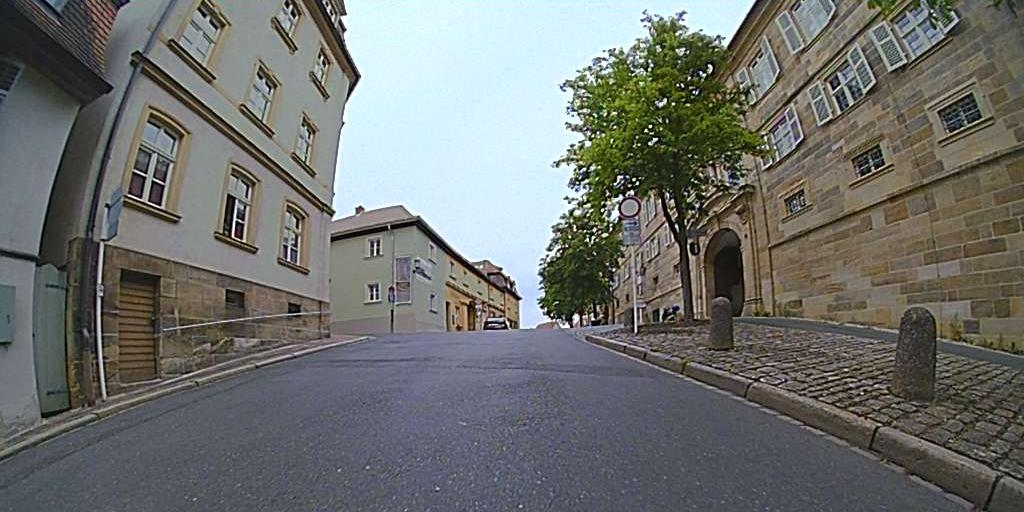} &
\includegraphics[height=\turnheightnew]{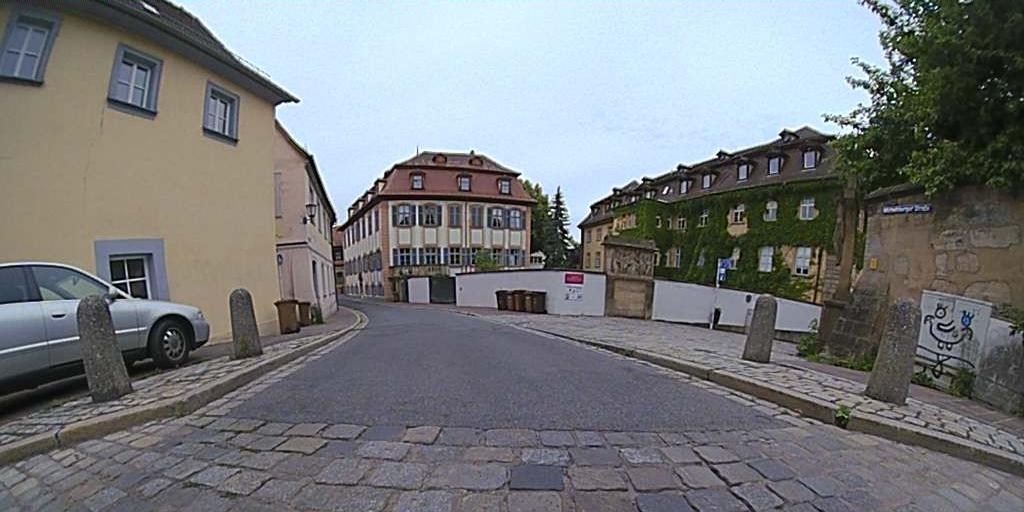} &
\includegraphics[height=\turnheightnew]{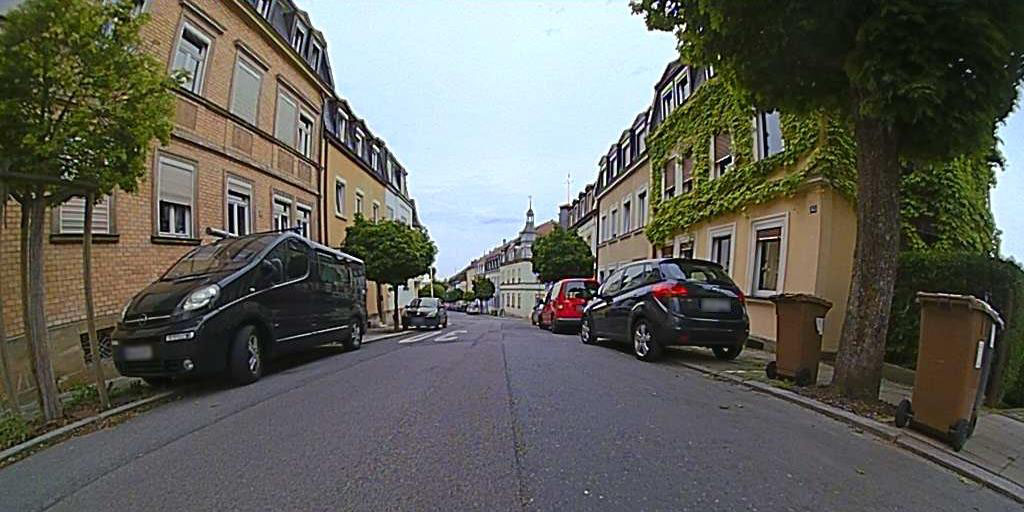} &
\includegraphics[height=\turnheightnew]{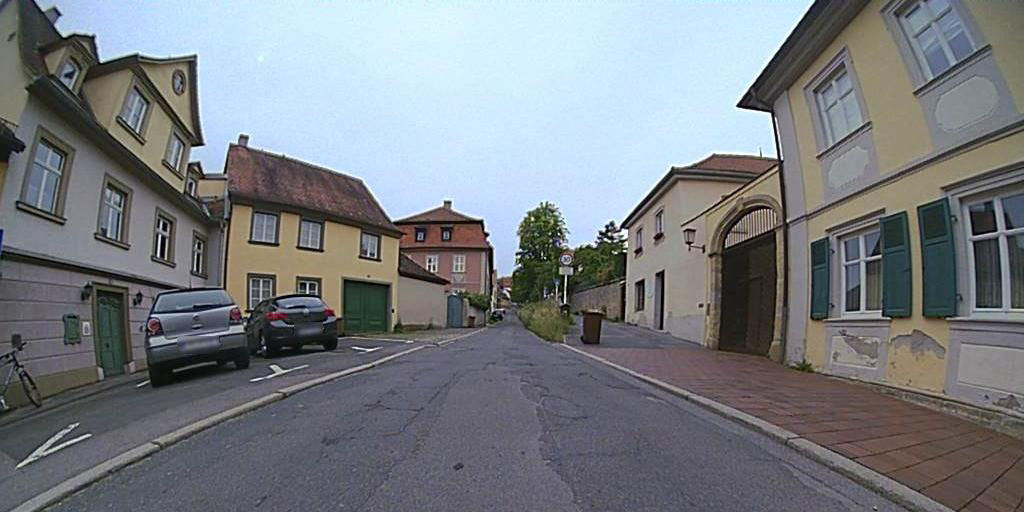} \\

{\rotatebox{90}{\hspace{0mm}\scriptsize}} &
\includegraphics[height=\turnheightnew]{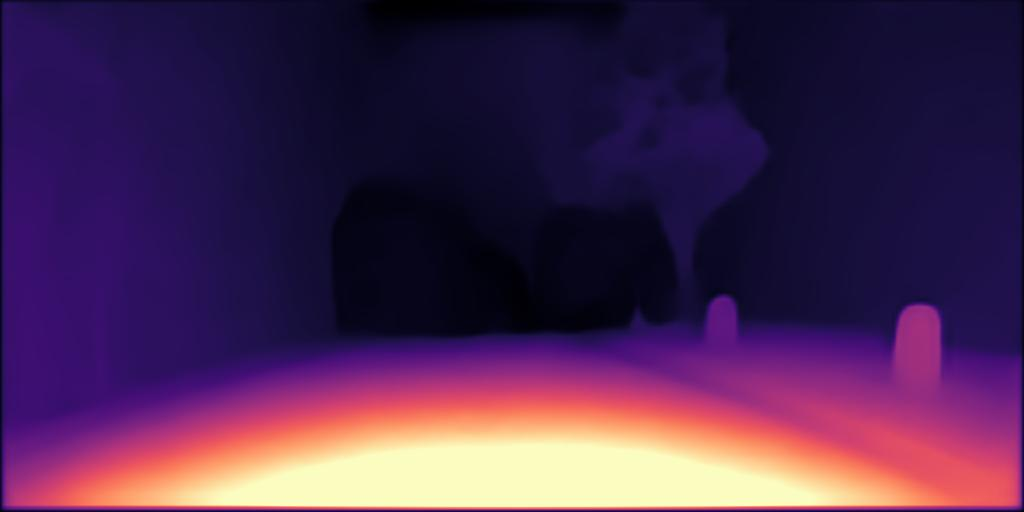} &
\includegraphics[height=\turnheightnew]{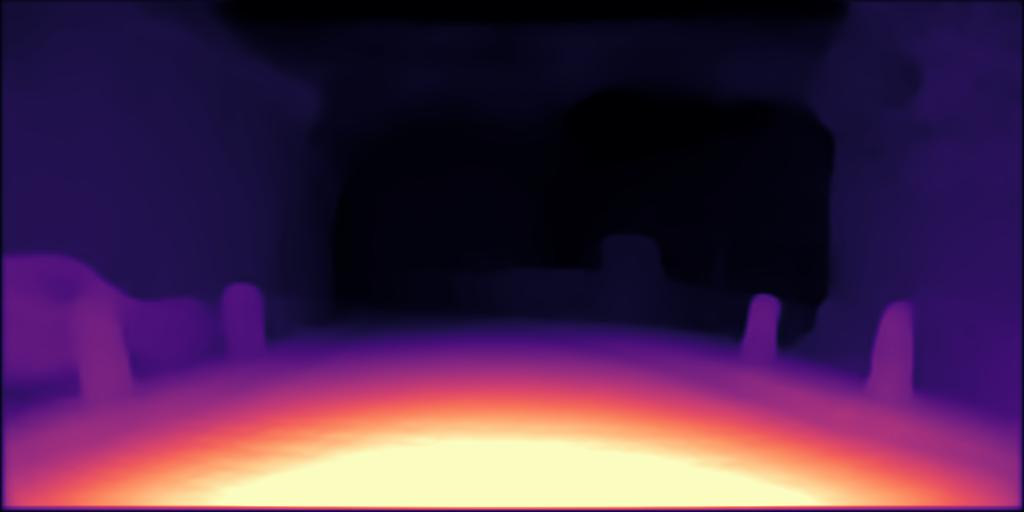} &
\includegraphics[height=\turnheightnew]{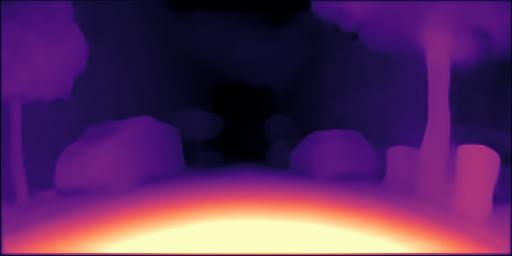} &
\includegraphics[height=\turnheightnew]{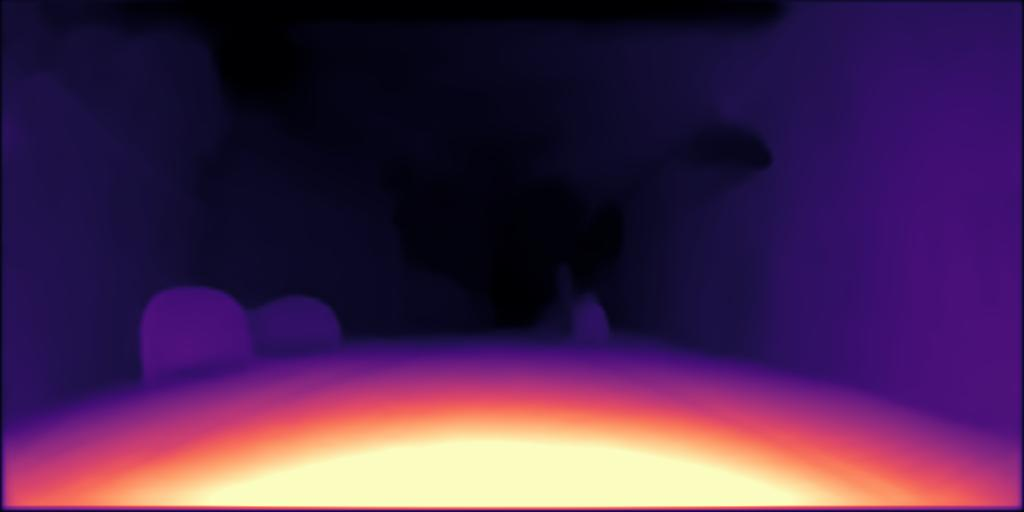} \\
\end{tabular}
}
  \caption{\textbf{Qualitative results on the Fisheye WoodScape~\cite{yogamani2019woodscape}}. In the 4th row of the table, we can see that our model adapts to the extreme distortion induced by the fisheye camera and produces sharp distance maps. In the 6th row, we can clearly see the sharp curbs on the street. Finally, in the last few rows, our model adapts to most of the complex scenes and produces very sharp scale-aware distance maps.}
  \label{fig:fisheye_suppl_qual}
\end{figure*}
% -------------------------------------------------
% FAILURE CASES for Fisheye
\begin{figure*}[!ht]
\captionsetup{belowskip=-8pt, skip=4pt, font=small, singlelinecheck=false}
  \centering
  \resizebox{\textwidth}{!}{
  \newcommand{\turnheightnew}{0.25\columnwidth}
\centering

\begin{tabular}{@{\hskip 0.5mm}c@{\hskip 0.5mm}c@{\hskip 0.5mm}c@{\hskip 0.5mm}c@{\hskip 0.5mm}c@{}}

{\rotatebox{90}{\hspace{0mm}}} &
\includegraphics[height=\turnheightnew]{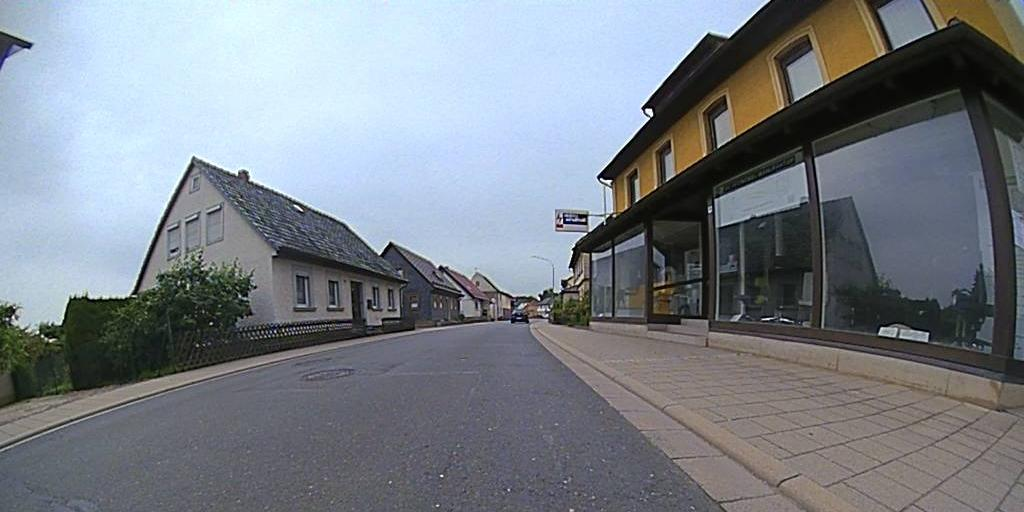} &
\includegraphics[height=\turnheightnew]{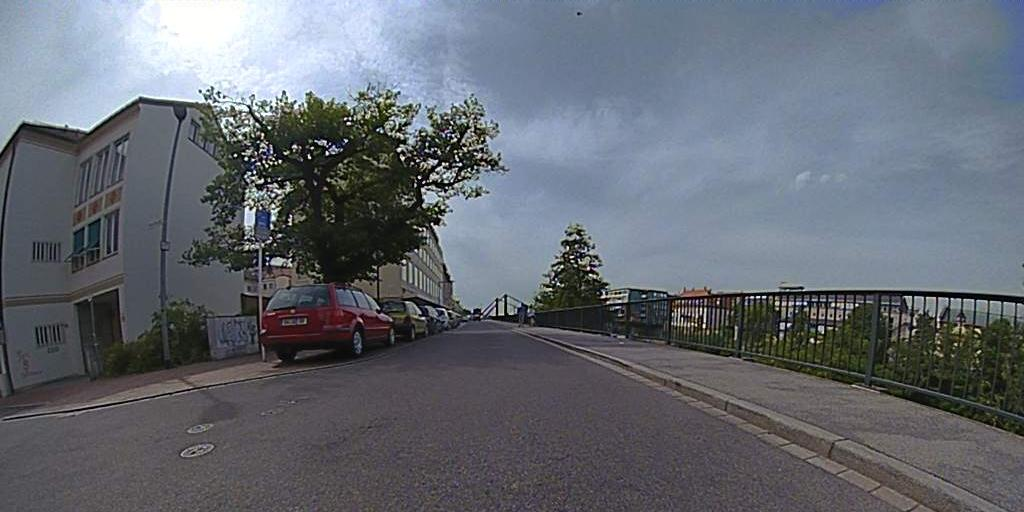} &
\includegraphics[height=\turnheightnew]{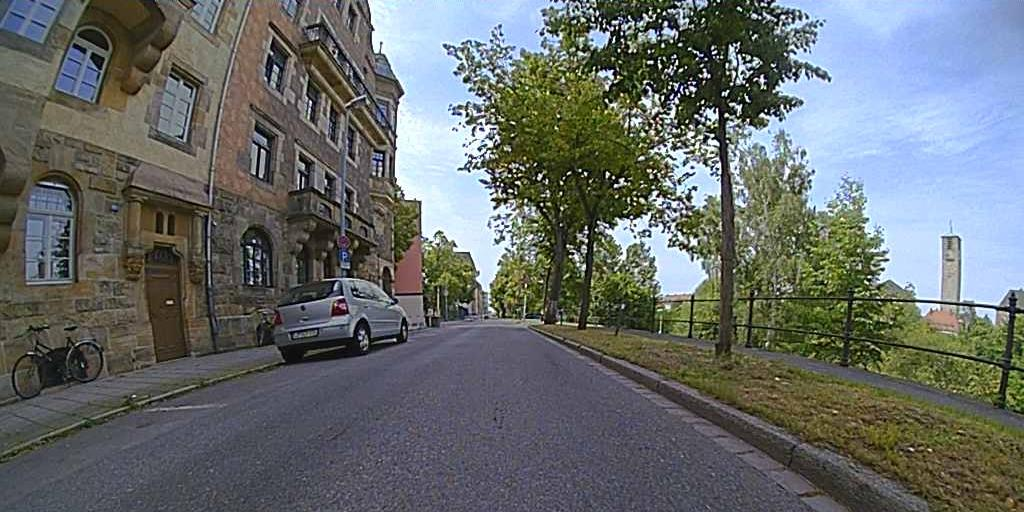} &
\includegraphics[height=\turnheightnew]{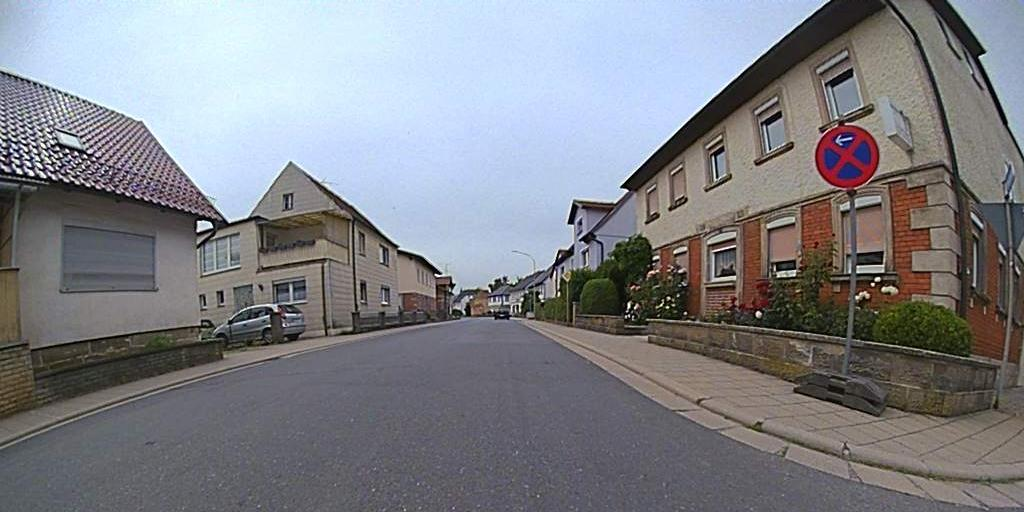}\\

{\rotatebox{90}{\hspace{0mm}\scriptsize}} &
\includegraphics[height=\turnheightnew]{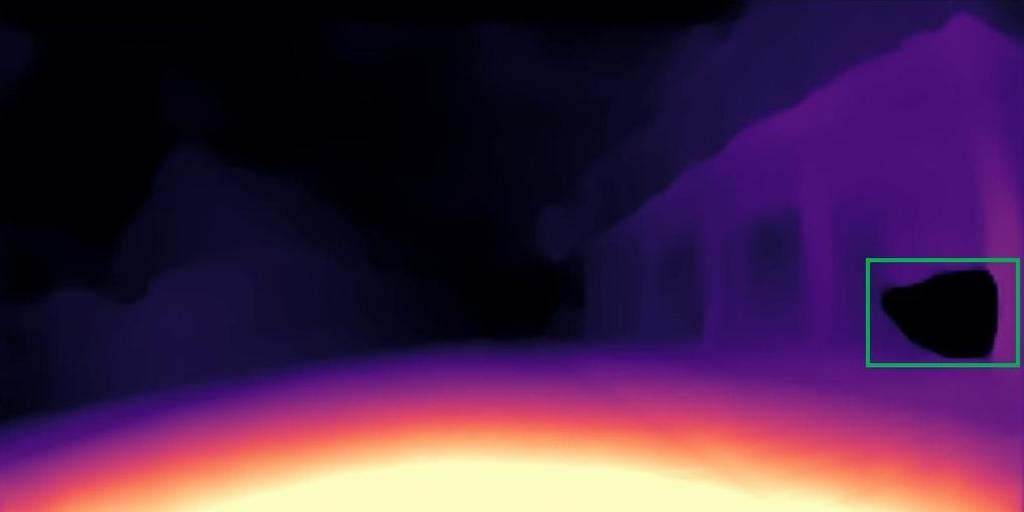} &
\includegraphics[height=\turnheightnew]{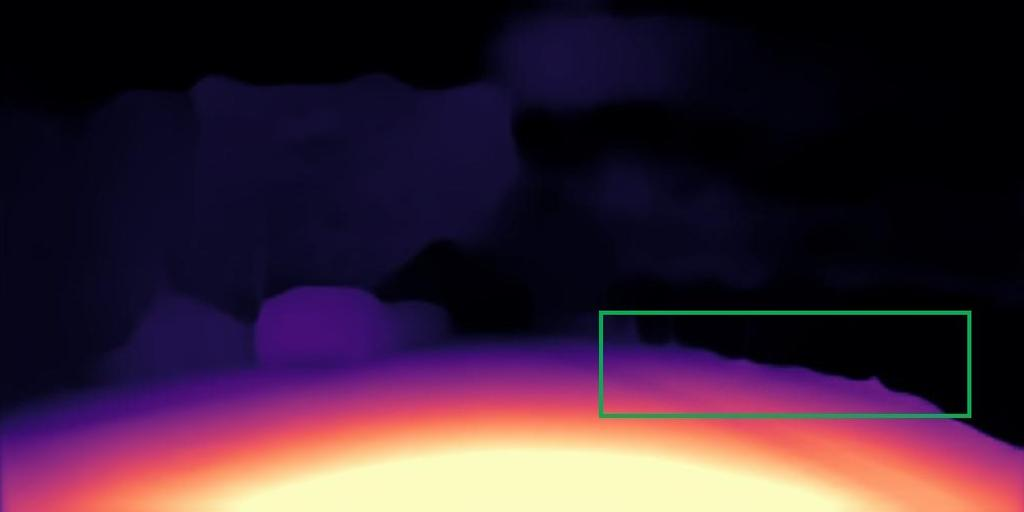} &
\includegraphics[height=\turnheightnew]{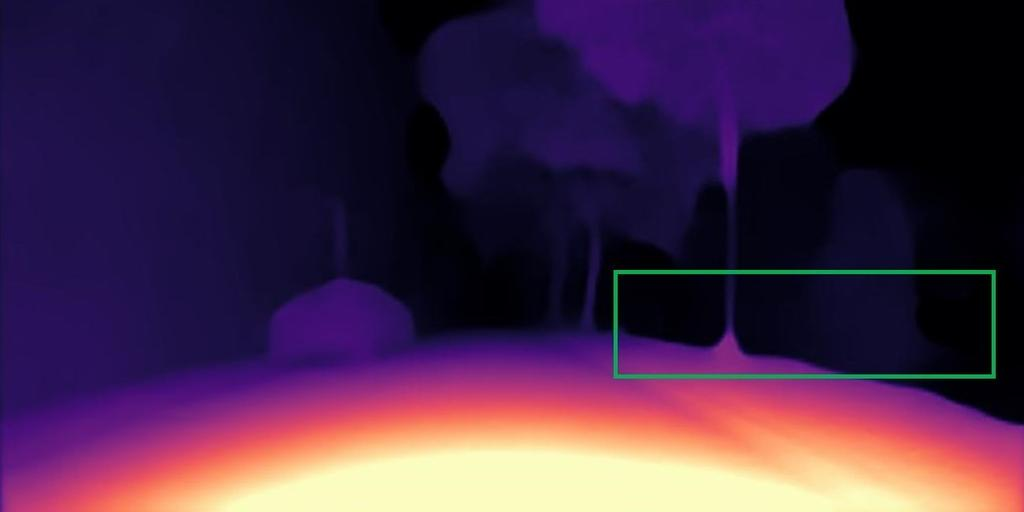} &
\includegraphics[height=\turnheightnew]{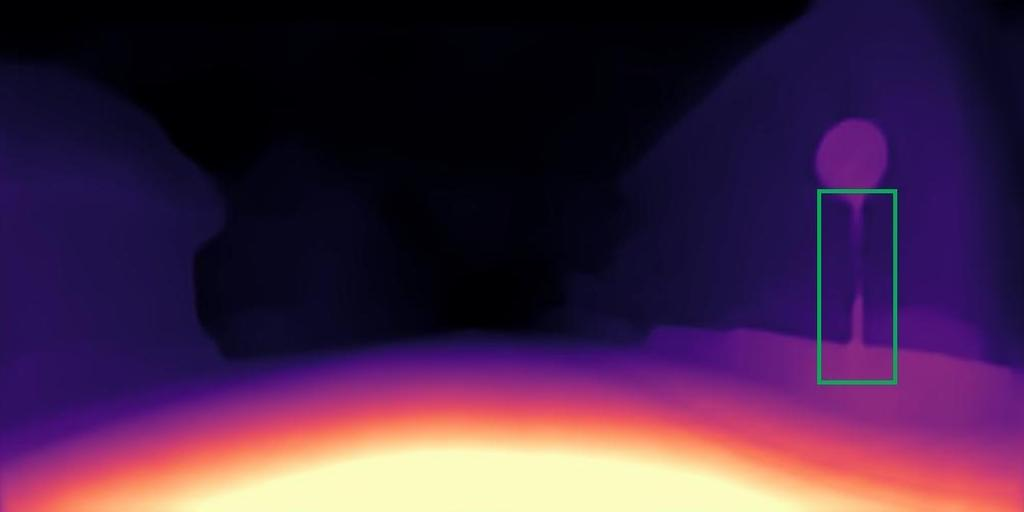} \\

\end{tabular}
}
   \caption{\textbf{Failure Cases on the Fisheye WoodScape~\cite{yogamani2019woodscape} dataset.} The photometric loss fails to learn good distances for reflective regions which can be seen in the $1^\text{st}$ figure. In the following figures shown above, the model fails to accurately delineate objects where boundaries are ambiguous.}
  \label{fig:fisheye_failure}
\end{figure*}
% -------------------------------------------------
\begin{figure*}[!ht]
\captionsetup{belowskip=-8pt, skip=4pt, font=small, singlelinecheck=false}
  \centering
  \resizebox{\textwidth}{!}{
  \newcommand{\turnheightnew}{0.5\columnwidth}
\centering
\begin{tabular}{@{\hskip 0.5mm}c@{\hskip 0.5mm}c@{\hskip 0.5mm}c@{}}

\includegraphics[height=\turnheightnew]{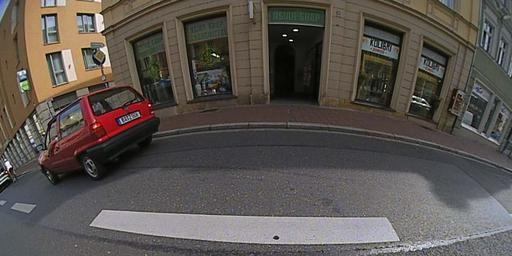} &
\includegraphics[height=\turnheightnew]{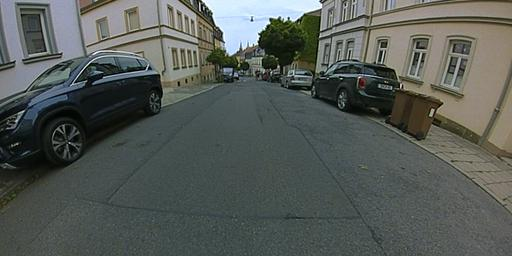} \\
\includegraphics[height=\turnheightnew]{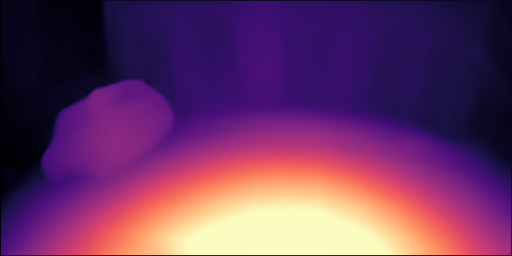} &
\includegraphics[height=\turnheightnew]{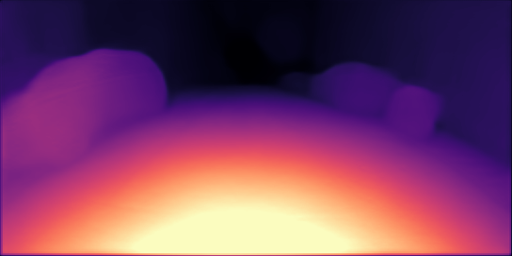} \\
\includegraphics[height=\turnheightnew]{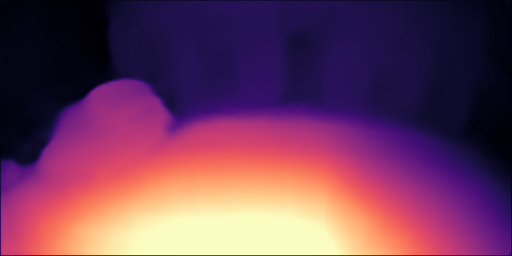} &
\includegraphics[height=\turnheightnew]{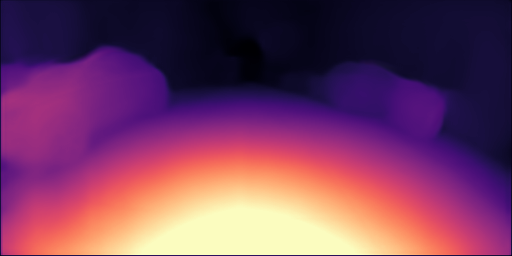} \\
\end{tabular}
}
\caption{\textbf{Qualitative results on an unseen sequence} from one of our test cars with a different camera intrinsic. $1^{st}$ row indicates the raw input images from the right and rear camera. $2^{nd}$ and $3^{rd}$ row indicates the distance estimates of the network trained with and without camera geometry tensor. Despite the notable variation in the camera parameters, the network with camera geometry tensor outputs sharp distance maps on which edges are visible.}
  \label{fig:cam_tensor_suppl}
\end{figure*}
% -------------------------------------------------
\begin{figure*}[!ht]
\captionsetup{belowskip=-8pt, font=small, singlelinecheck=false}
  \centering
  \newcommand{\turnheightnew}{0.45\columnwidth}
\centering

\begin{adjustbox}{width=\textwidth, totalheight=8.2in, keepaspectratio}
\begin{tabular}{@{\hskip 0.5mm}c@{\hskip 0.5mm}c@{\hskip 0.5mm}c@{\hskip 0.5mm}}

{\rotatebox{90}{\hspace{9mm} \large Raw Input}} &
\includegraphics[height=\turnheightnew]{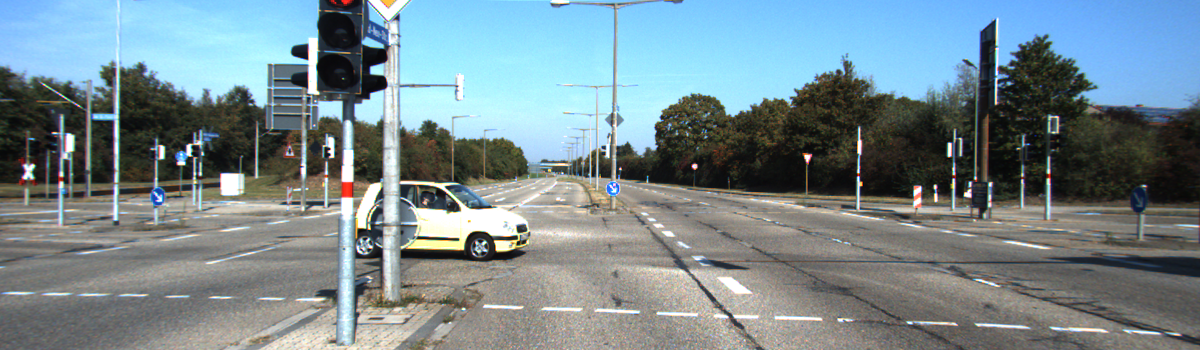} &
\includegraphics[height=\turnheightnew]{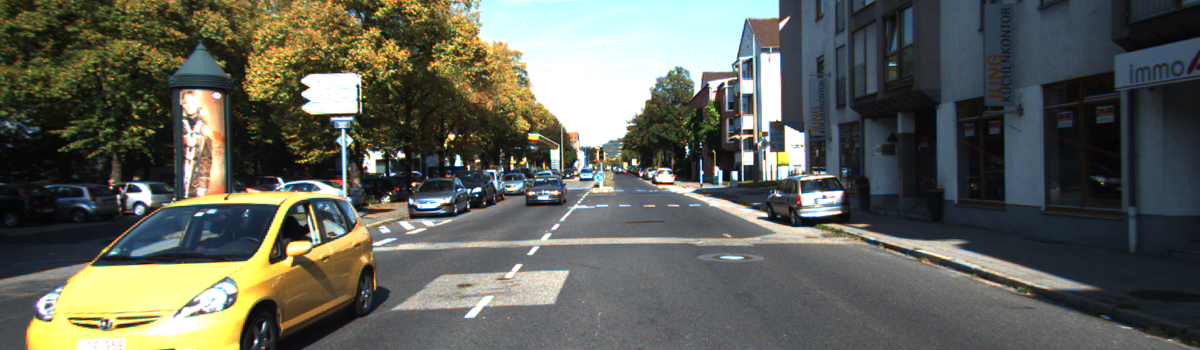} \\

{\rotatebox{90}{\hspace{9mm} \large SVDistNet}} &
\includegraphics[height=\turnheightnew]{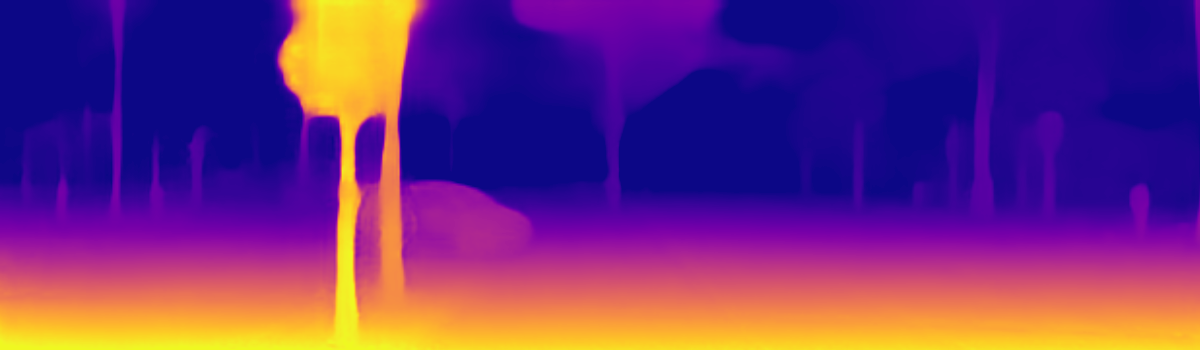} &
\includegraphics[height=\turnheightnew]{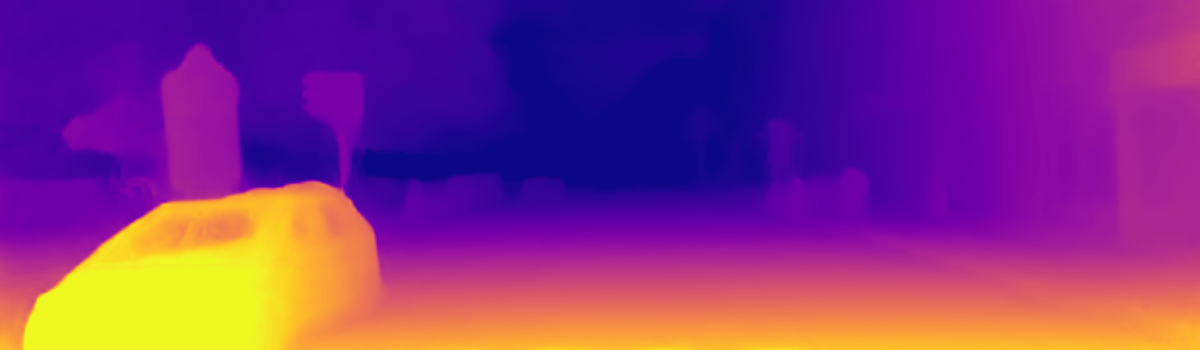} \\

{\rotatebox{90}{\hspace{9mm} \large SVDistNet}} &
\includegraphics[height=\turnheightnew]{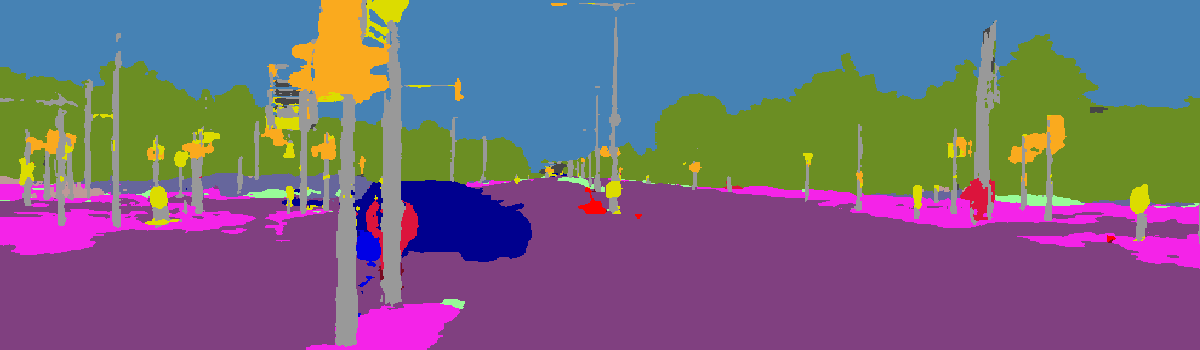} &
\includegraphics[height=\turnheightnew]{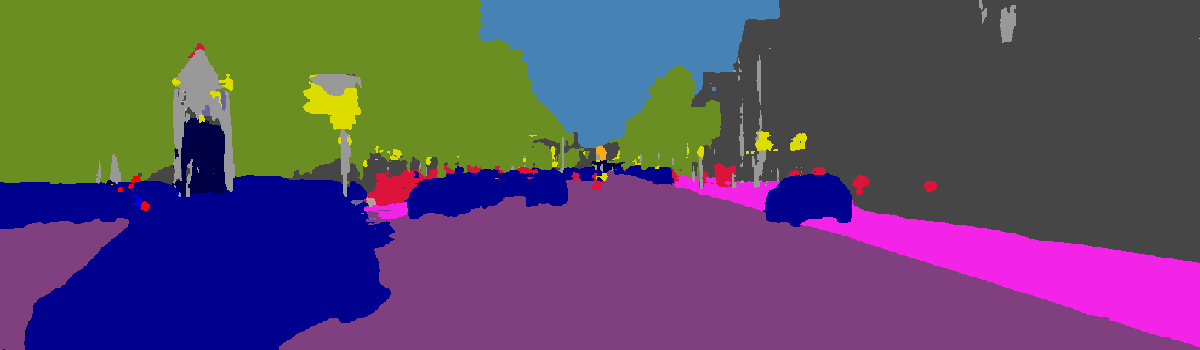} \\

{\rotatebox{90}{\hspace{9mm} \large Raw Input}} &
\includegraphics[height=\turnheightnew]{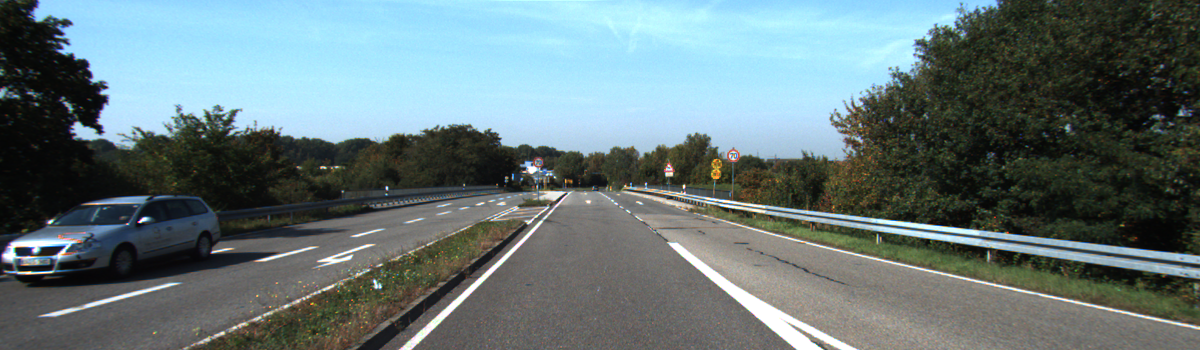} &
\includegraphics[height=\turnheightnew]{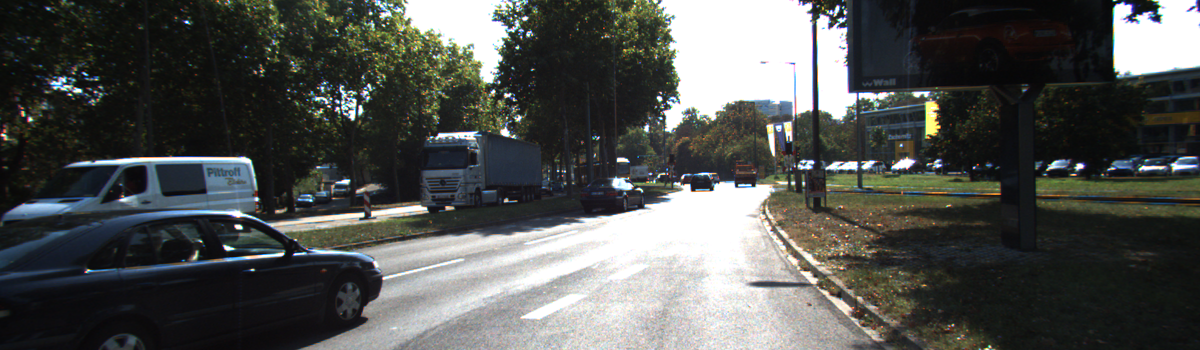} \\

{\rotatebox{90}{\hspace{9mm} \large SVDistNet}} &
\includegraphics[height=\turnheightnew]{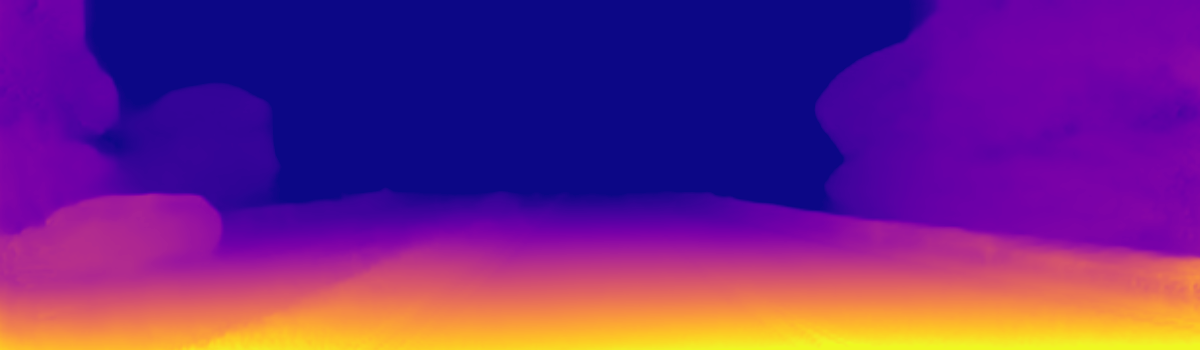} &
\includegraphics[height=\turnheightnew]{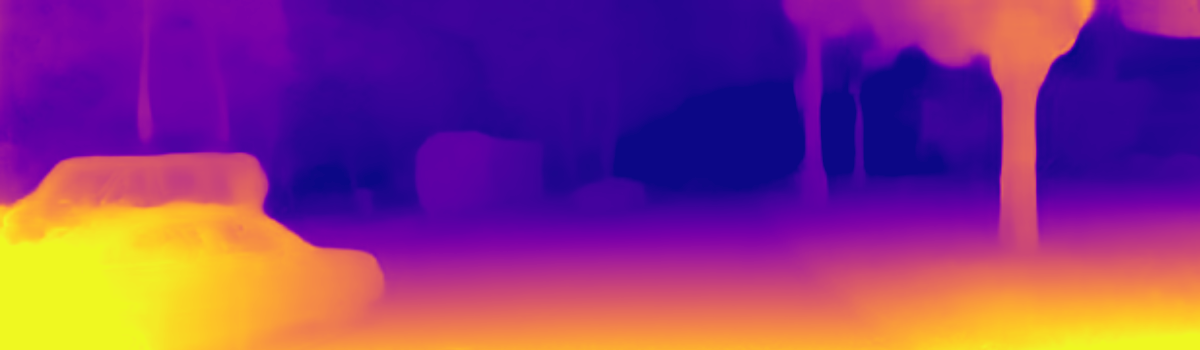} \\

{\rotatebox{90}{\hspace{9mm} \large SVDistNet}} &
\includegraphics[height=\turnheightnew]{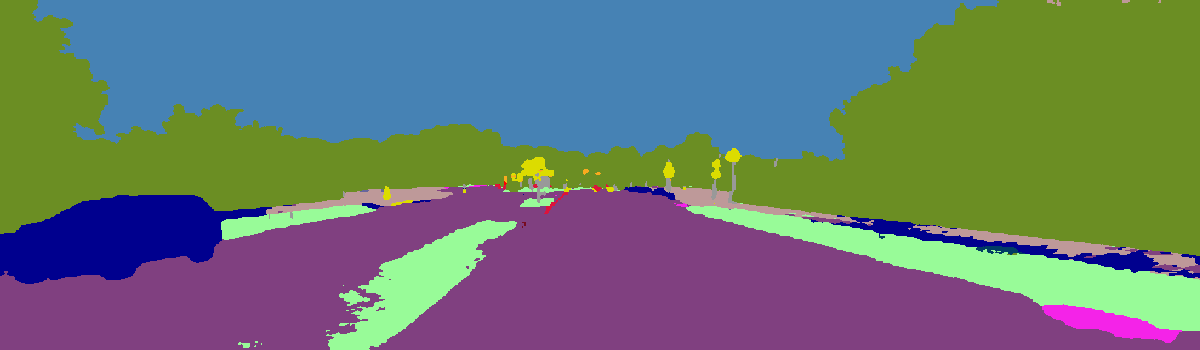} &
\includegraphics[height=\turnheightnew]{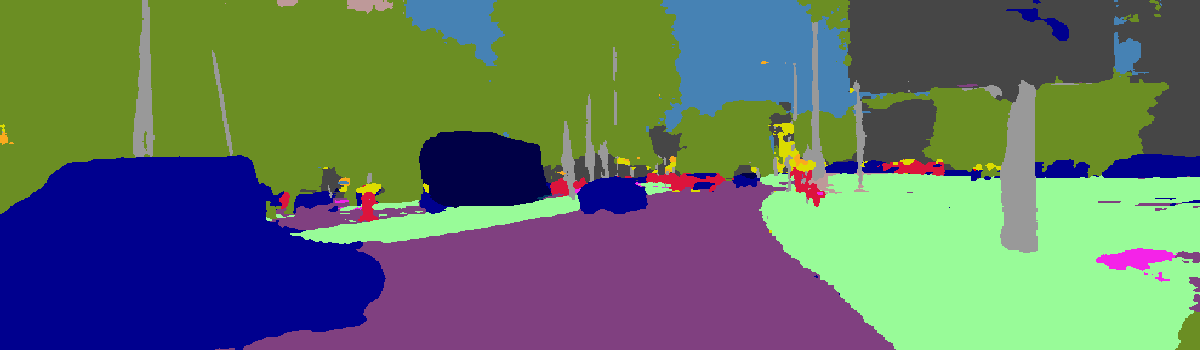} \\

{\rotatebox{90}{\hspace{9mm} \large Raw Input}} &
\includegraphics[height=\turnheightnew]{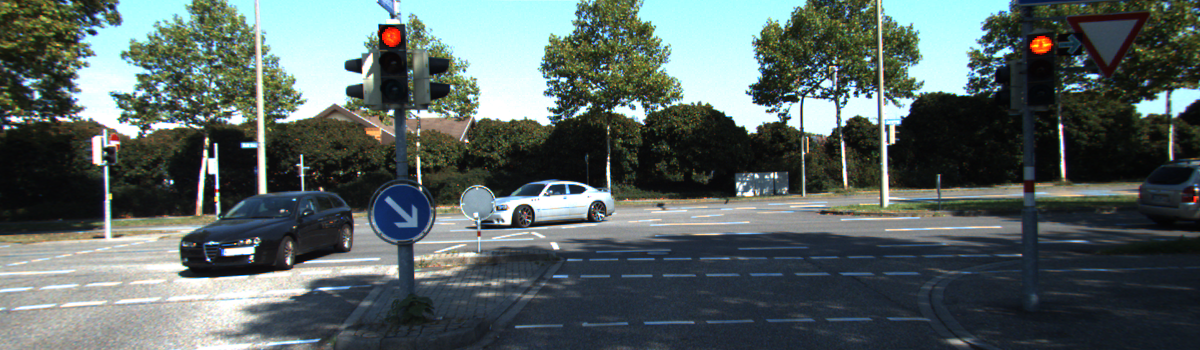} &
\includegraphics[height=\turnheightnew]{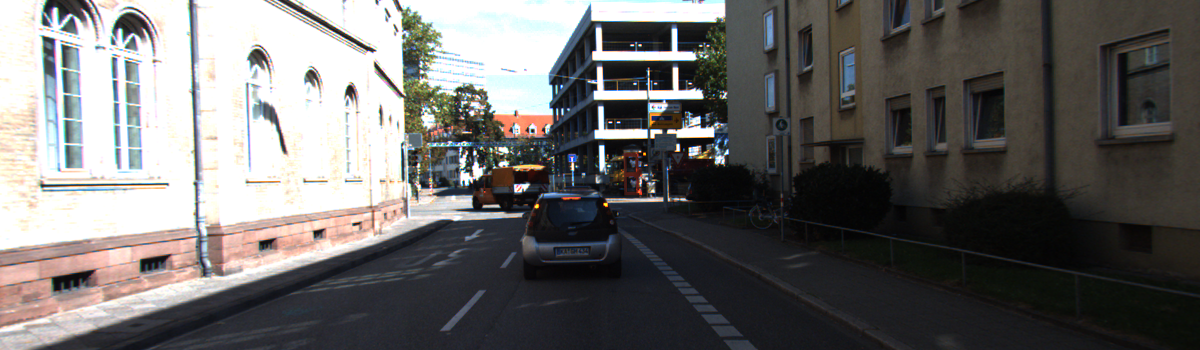} \\

{\rotatebox{90}{\hspace{9mm} \large SVDistNet}} &
\includegraphics[height=\turnheightnew]{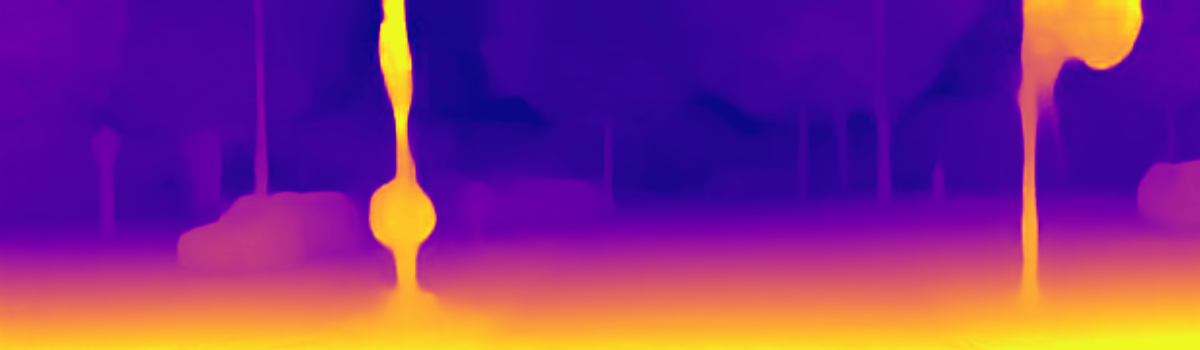} &
\includegraphics[height=\turnheightnew]{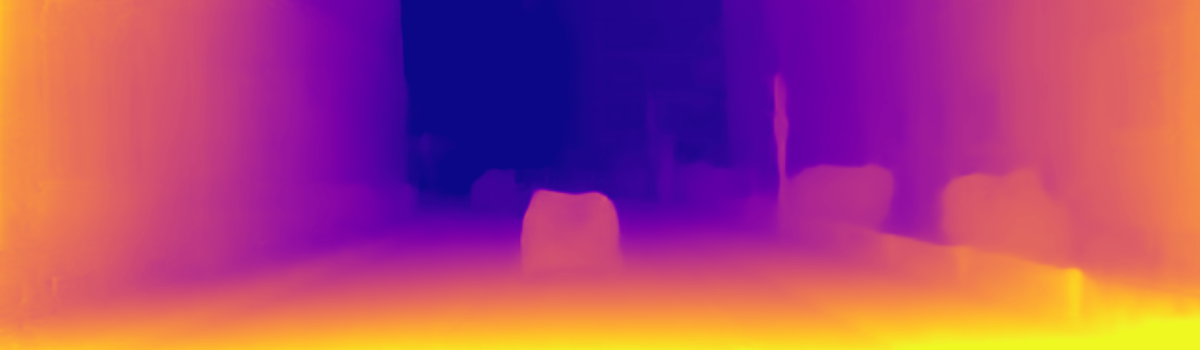} \\

{\rotatebox{90}{\hspace{9mm} \large SVDistNet}} &
\includegraphics[height=\turnheightnew]{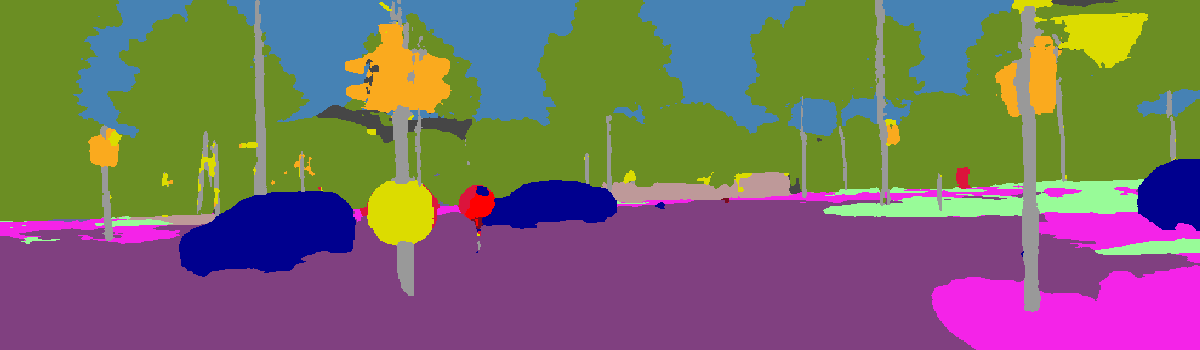} &
\includegraphics[height=\turnheightnew]{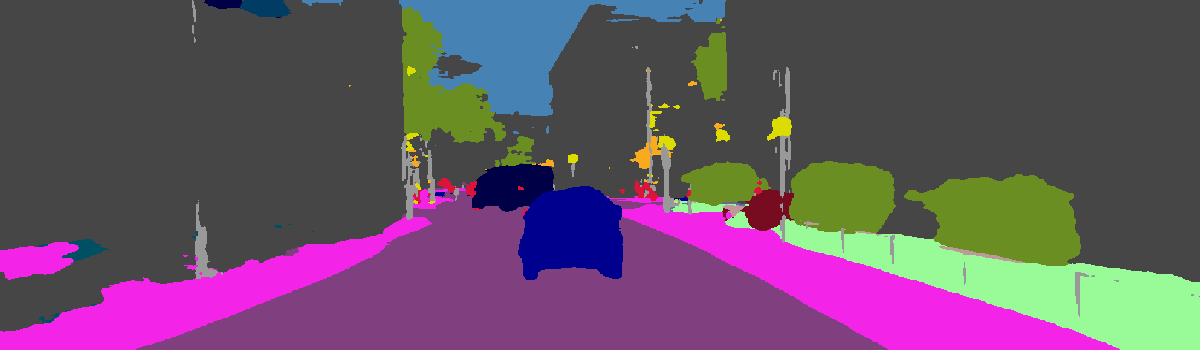} \\

%{\rotatebox{90}{\hspace{3mm}Raw Input}} &
%\includegraphics[height=\turnheightnew]{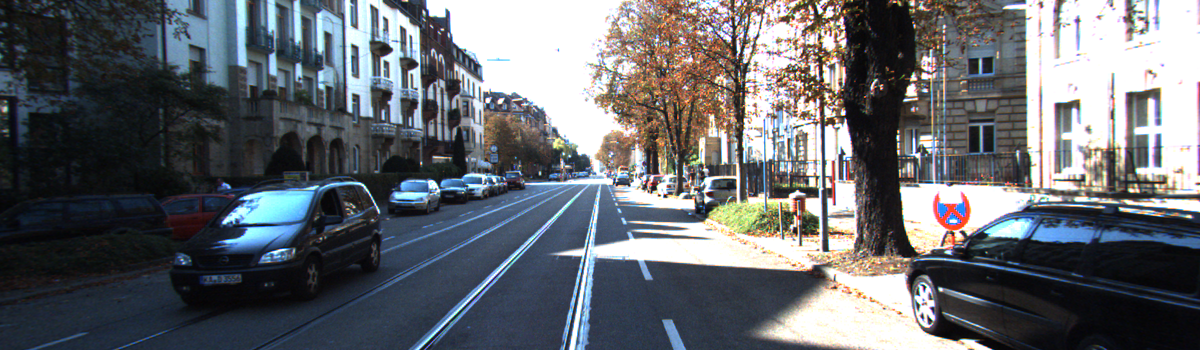} &
%\includegraphics[height=\turnheightnew]{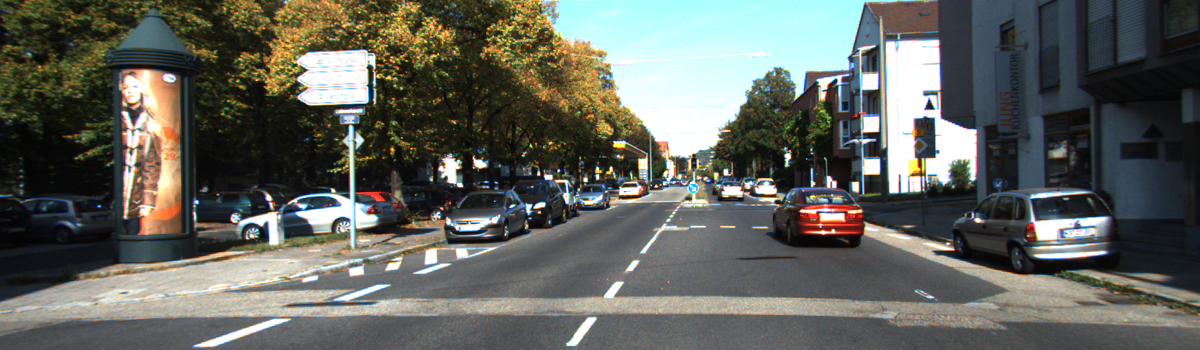} \\

%{\rotatebox{90}{\hspace{3mm}SVDistNet}} &
%\includegraphics[height=\turnheightnew]{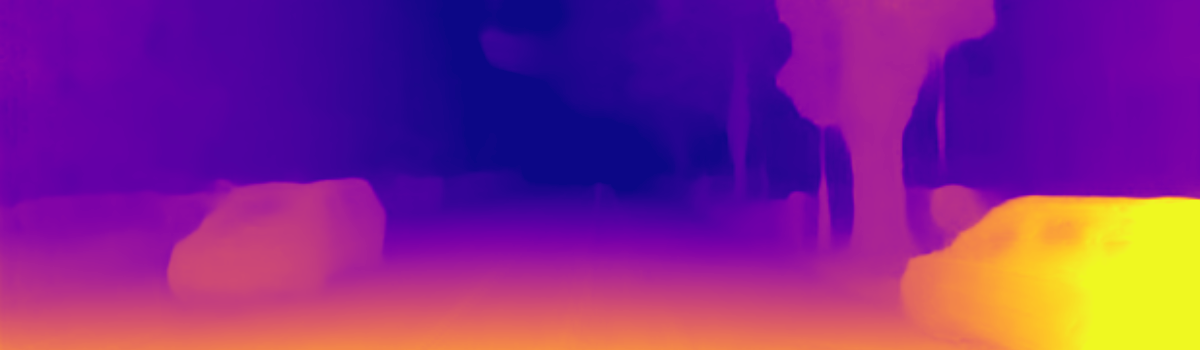} &
%\includegraphics[height=\turnheightnew]{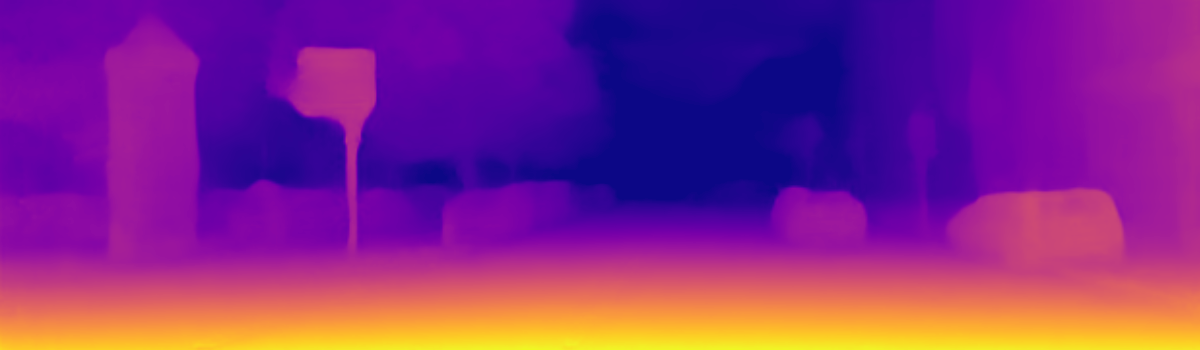} \\

%{\rotatebox{90}{\hspace{3mm}SVDistNet}} &
%\includegraphics[height=\turnheightnew]{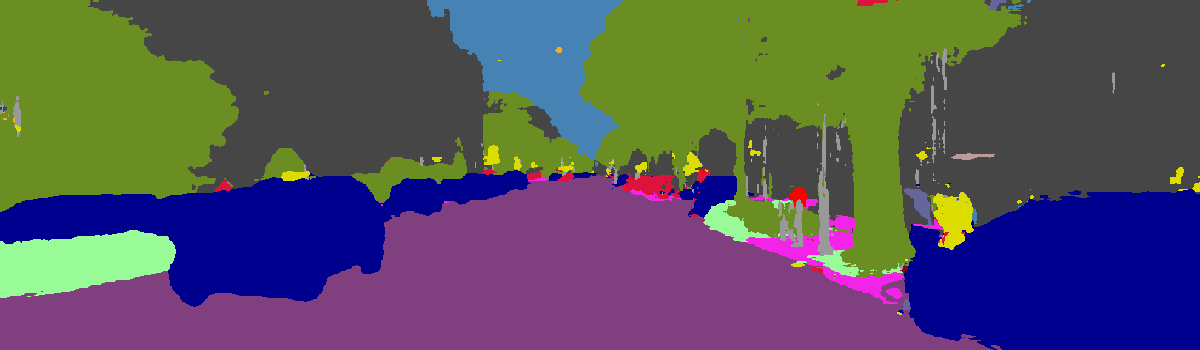} &
%\includegraphics[height=\turnheightnew]{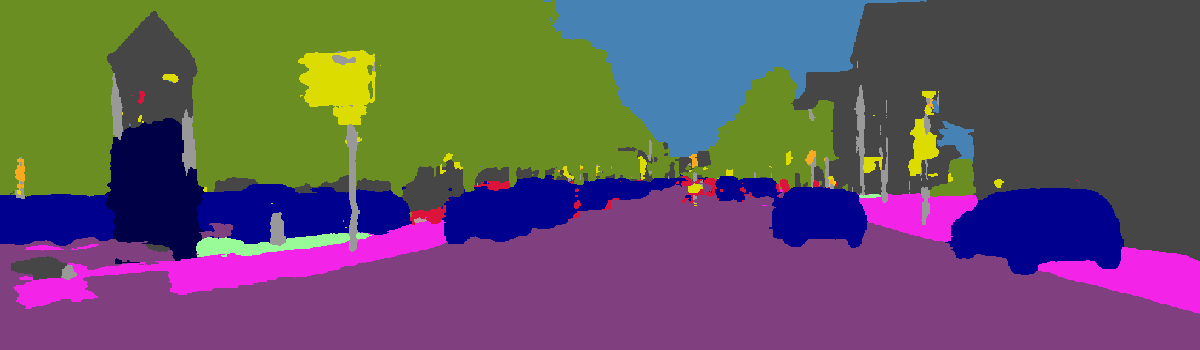}\\

\end{tabular}
\end{adjustbox}

\caption{\textbf{Qualitative results on the KITTI dataset.}
We showcase depth estimation as well as semantic segmentation outputs on the KITTI dataset using our SVDistNet model.}
  \label{fig:KITTIMTLSupplResults}
\end{figure*}
% -------------------------------------------------
\begin{figure*}[!ht]
  \captionsetup{belowskip=-8pt, font=small, singlelinecheck=false}
  \resizebox{\textwidth}{!}{
    \newcommand{\turnheightnew}{0.23\columnwidth}
\centering

\begin{tabular}{@{\hskip 0.5mm}c@{\hskip 0.5mm}c@{\hskip 0.5mm}c@{\hskip 0.5mm}c@{\hskip 0.5mm}c@{}}

{\rotatebox{90}{\hspace{5mm}\normalsize
{Input}}} &
\includegraphics[height=\turnheightnew]{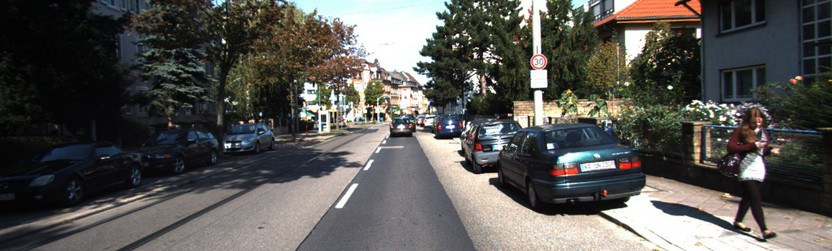} &
\includegraphics[height=\turnheightnew]{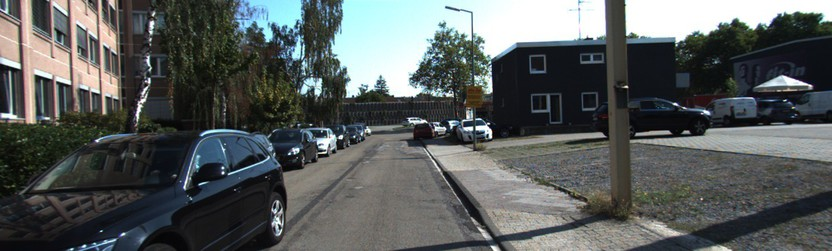} &
\includegraphics[height=\turnheightnew]{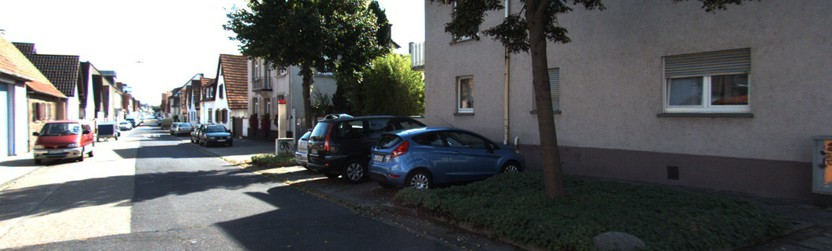} &
\includegraphics[height=\turnheightnew]{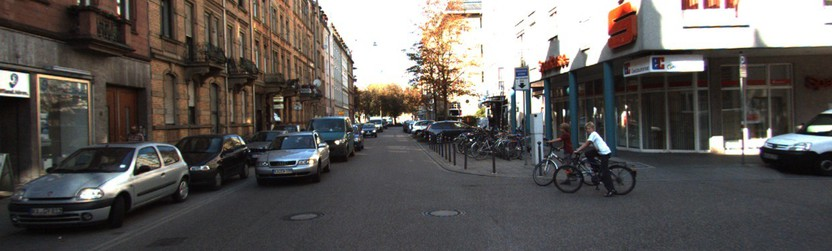}\\

{\rotatebox{90}{\hspace{0mm}\small
{Monodepth~\cite{Godard2017}}}} &
\includegraphics[height=\turnheightnew]{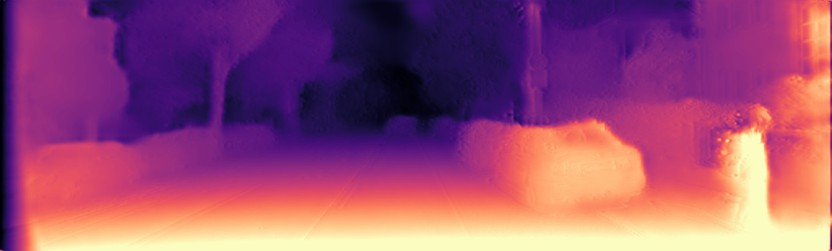} &
\includegraphics[height=\turnheightnew]{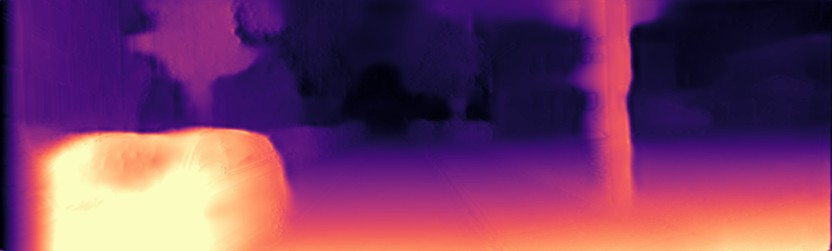} &
\includegraphics[height=\turnheightnew]{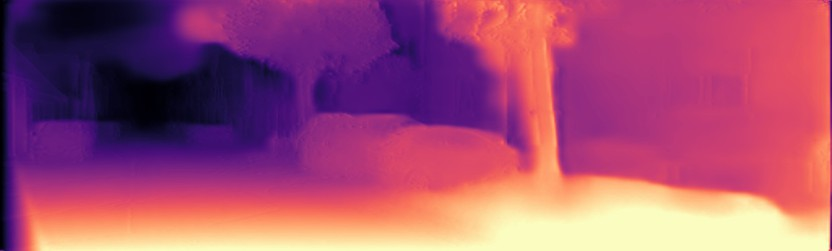} &
\includegraphics[height=\turnheightnew]{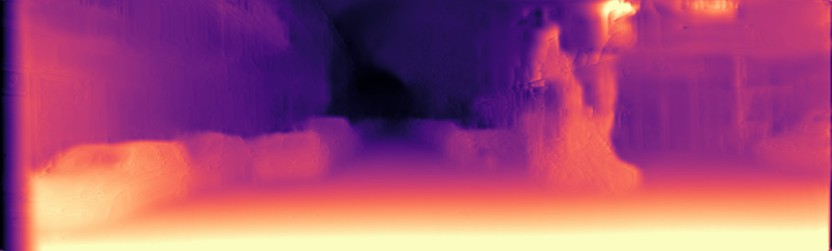} \\

{\rotatebox{90}{\hspace{0mm}\small
{Zhou \etal~\cite{zhou2017unsupervised}}}} &
\includegraphics[height=\turnheightnew]{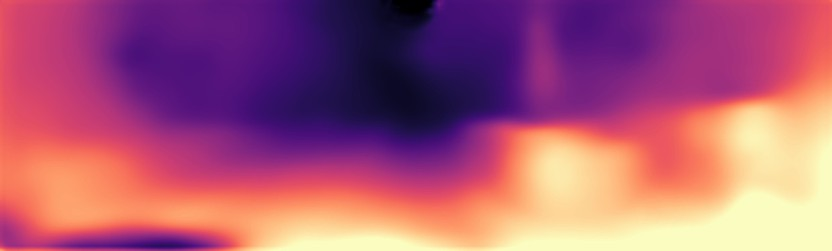} &
\includegraphics[height=\turnheightnew]{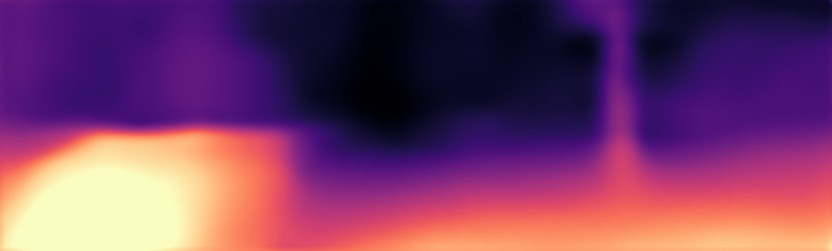} &
\includegraphics[height=\turnheightnew]{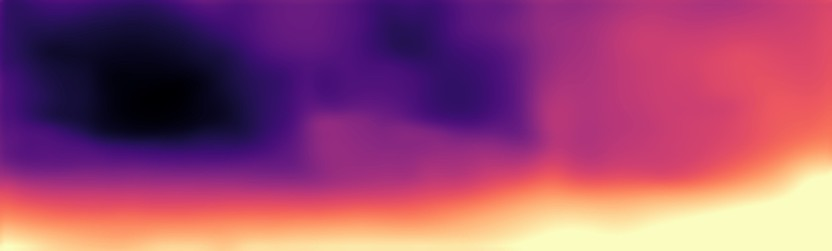} &
\includegraphics[height=\turnheightnew]{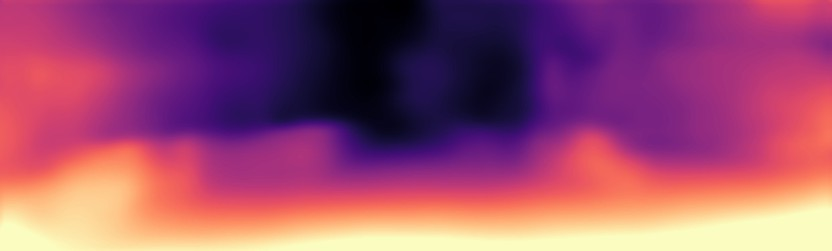} \\

{\rotatebox{90}{\hspace{2mm}\small
{DDVO~\cite{Wang2018e}}}} &
\includegraphics[height=\turnheightnew]{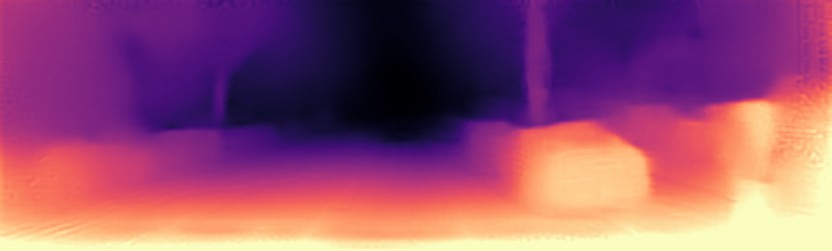} &
\includegraphics[height=\turnheightnew]{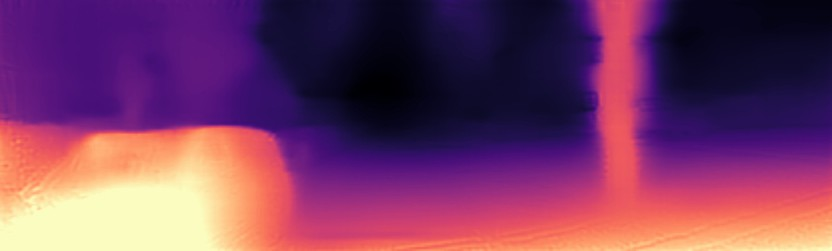} &
\includegraphics[height=\turnheightnew]{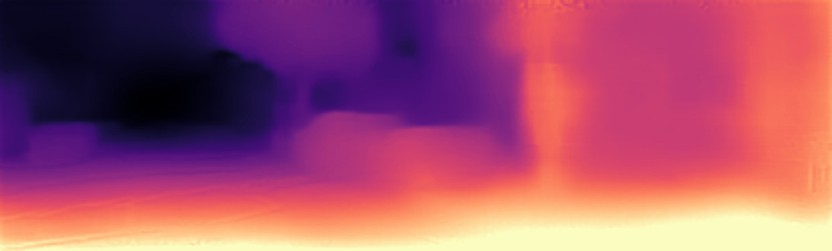} &
\includegraphics[height=\turnheightnew]{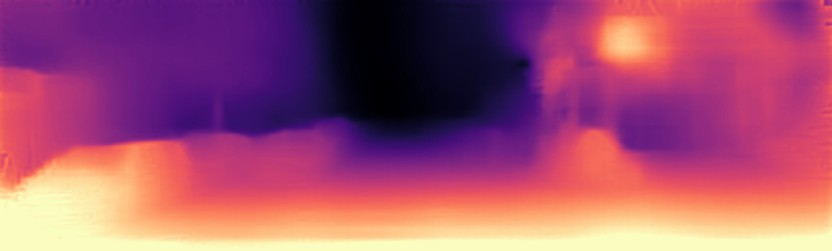} \\

{\rotatebox{90}{\hspace{2mm}\small
{GeoNet~\cite{Yin2018}}}} &
\includegraphics[height=\turnheightnew]{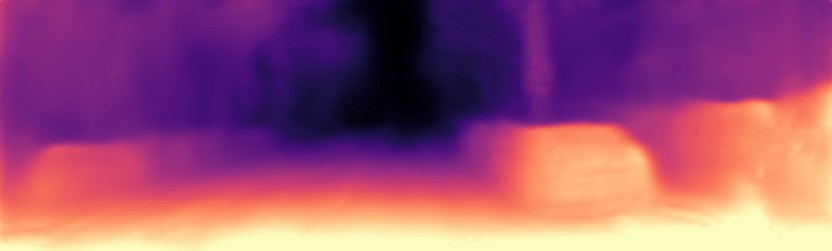} &
\includegraphics[height=\turnheightnew]{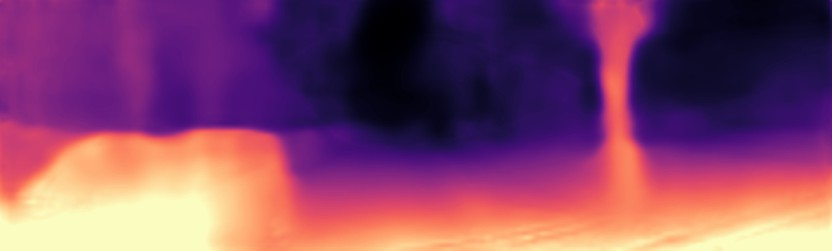} &
\includegraphics[height=\turnheightnew]{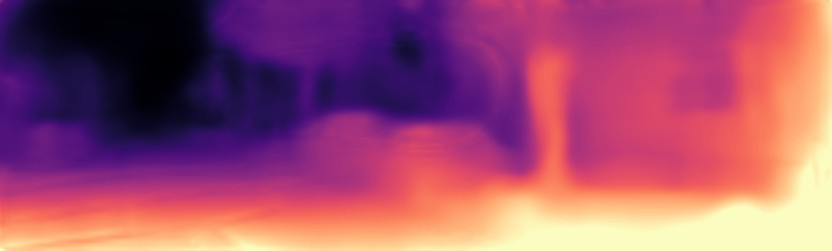} &
\includegraphics[height=\turnheightnew]{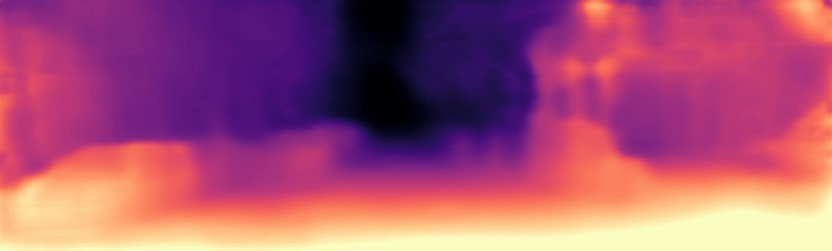} \\

{\rotatebox{90}{\hspace{0mm}\small
{Zhan \etal~\cite{zhan2018unsupervised}}}} &
\includegraphics[height=\turnheightnew]{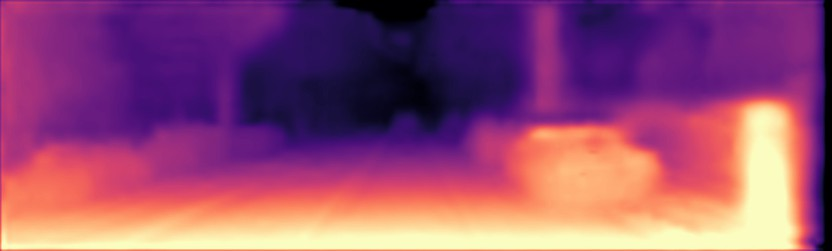} &
\includegraphics[height=\turnheightnew]{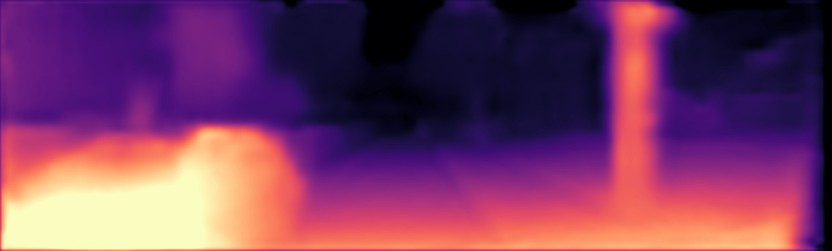} &
\includegraphics[height=\turnheightnew]{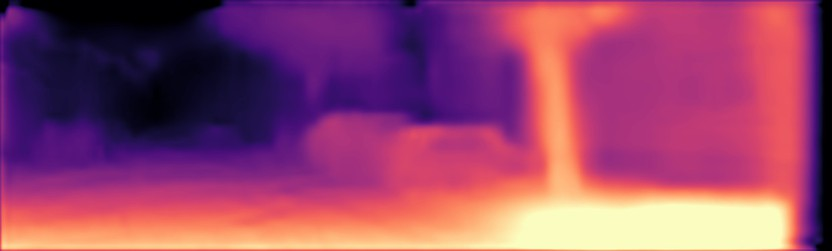} &
\includegraphics[height=\turnheightnew]{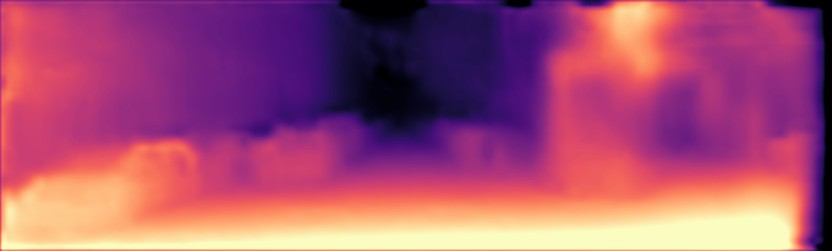} \\

{\rotatebox{90}{\hspace{0mm}\small
Ranjan et al.~\cite{Ranjan2019}}} &
\includegraphics[height=\turnheightnew]{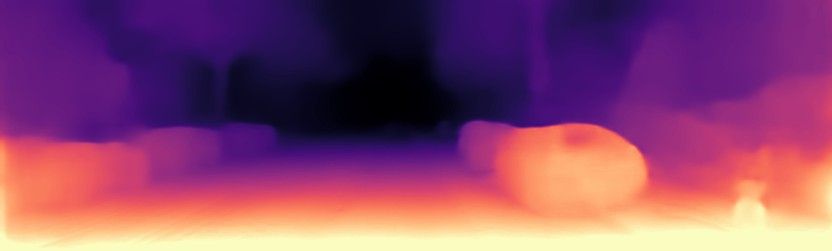} &
\includegraphics[height=\turnheightnew]{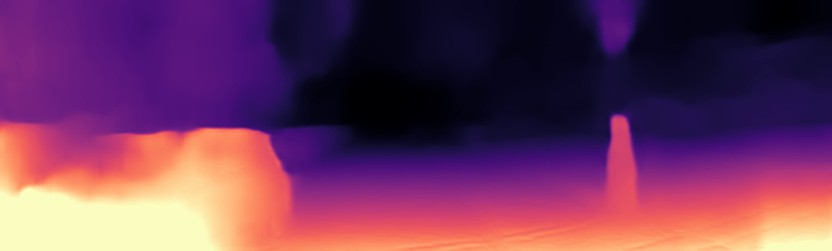} &
\includegraphics[height=\turnheightnew]{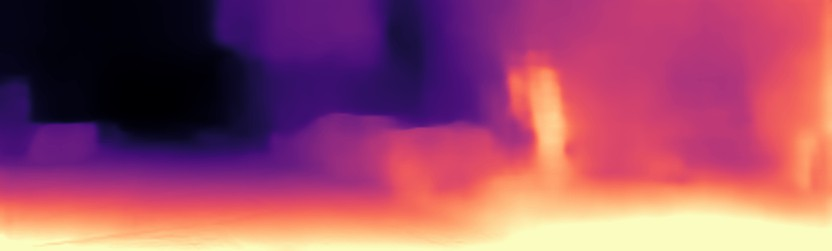} &
\includegraphics[height=\turnheightnew]{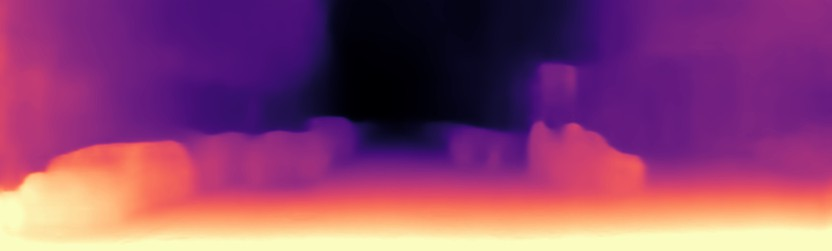} \\

{\rotatebox{90}{\hspace{0mm} \small
3Net-R50~\cite{Luo2019a}}} &
\includegraphics[height=\turnheightnew]{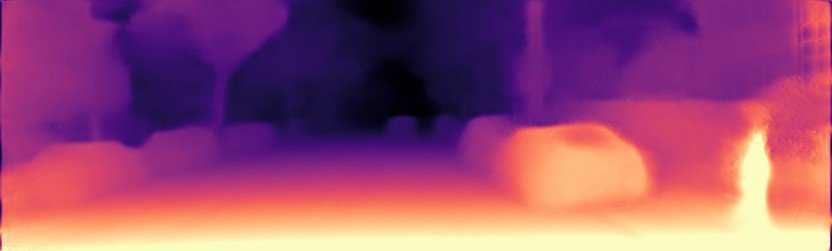} &
\includegraphics[height=\turnheightnew]{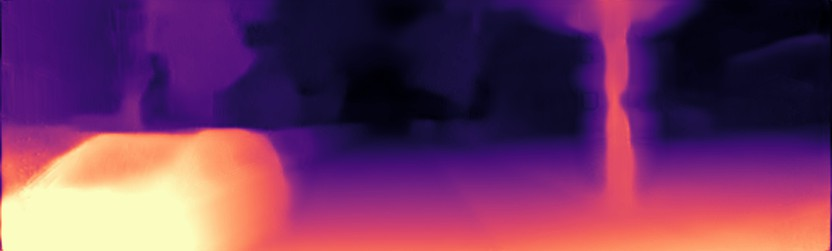} &
\includegraphics[height=\turnheightnew]{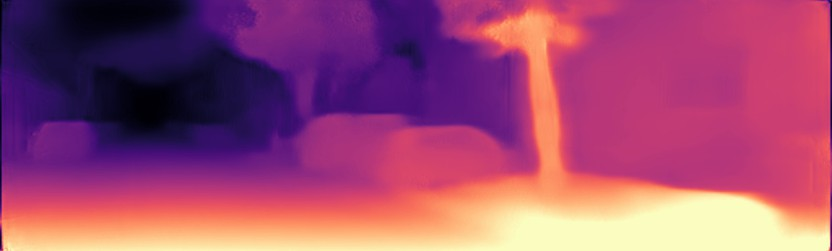} &
\includegraphics[height=\turnheightnew]{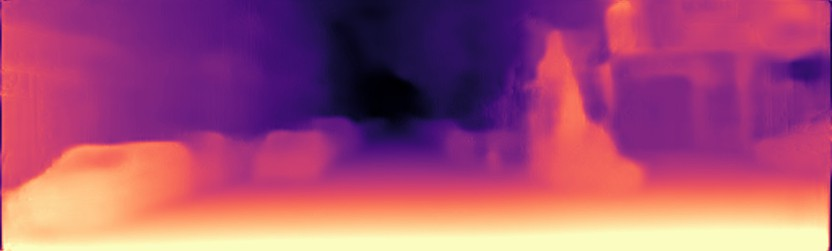} \\ 

{\rotatebox{90}{\hspace{0mm} \small
EPC++ (MS) \newline \cite{Luo2019a}}} &
\includegraphics[height=\turnheightnew]{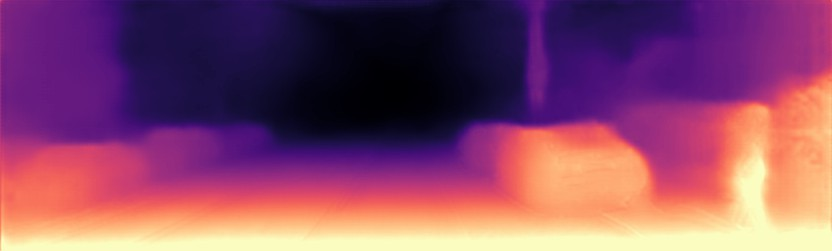} &
\includegraphics[height=\turnheightnew]{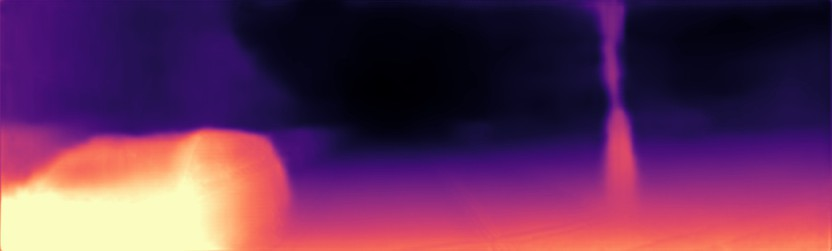} &
\includegraphics[height=\turnheightnew]{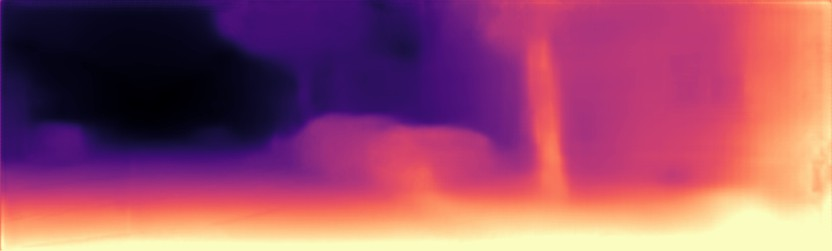} &
\includegraphics[height=\turnheightnew]{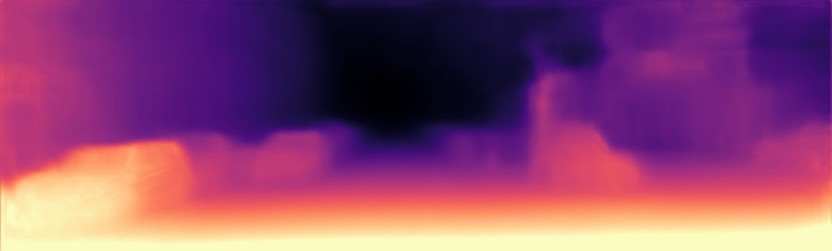} \\ 

{\rotatebox{90}{\hspace{0mm}\small
Monodepth2 M~\cite{Godard2019}}} &
\includegraphics[height=\turnheightnew]{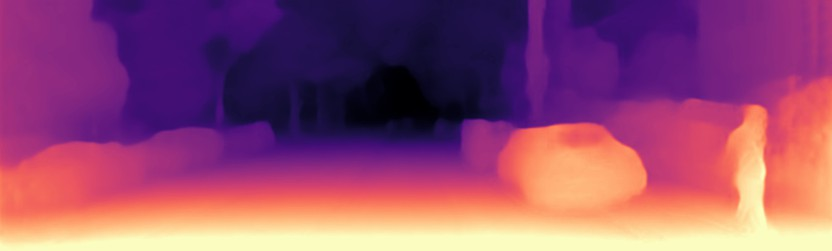} &
\includegraphics[height=\turnheightnew]{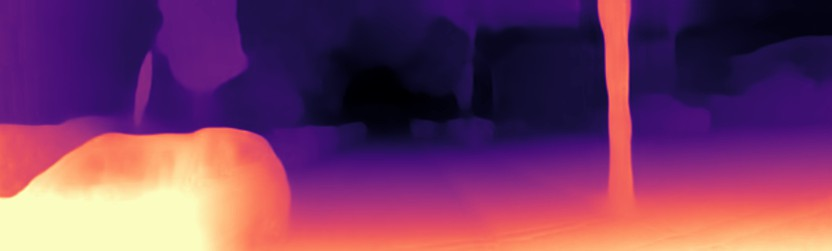} &
\includegraphics[height=\turnheightnew]{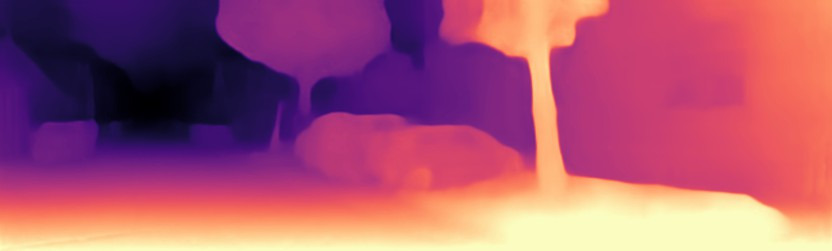} &
\includegraphics[height=\turnheightnew]{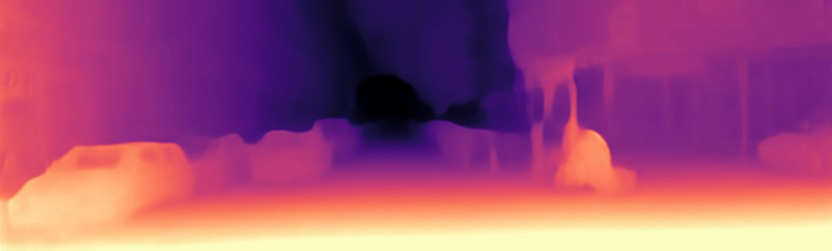} \\

{\rotatebox{90}{\hspace{3mm}\small
\textbf{SVDistNet}}} &
\includegraphics[height=\turnheightnew]{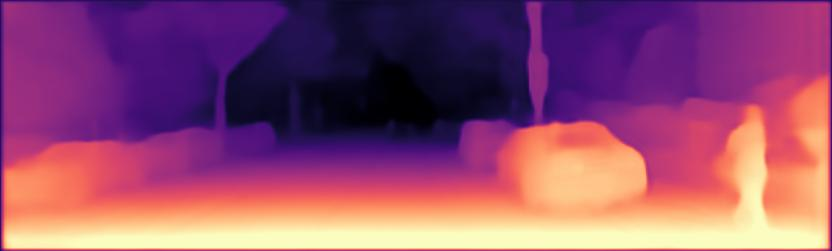} &
\includegraphics[height=\turnheightnew]{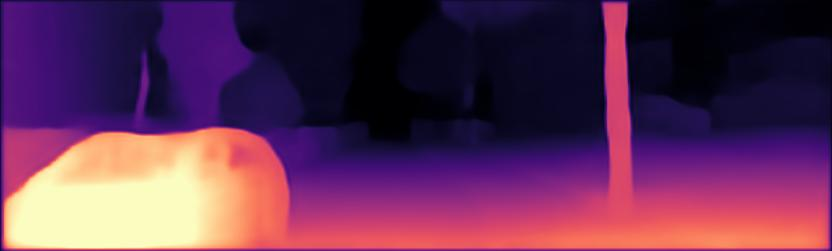} &
\includegraphics[height=\turnheightnew]{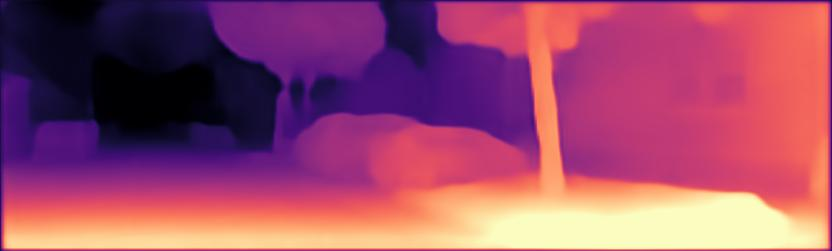} &
\includegraphics[height=\turnheightnew]{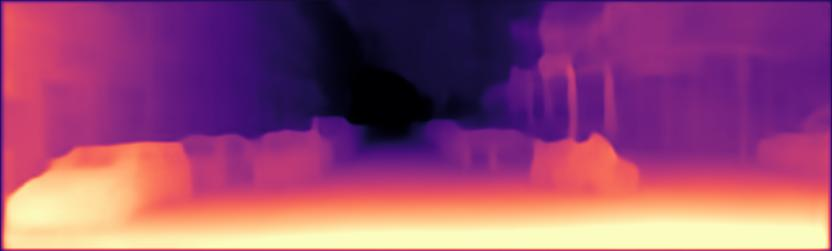} \\

\end{tabular}
}
\caption{\textbf{Qualitative results on the KITTI dataset.}
Our SynDistNet produces sharp depth maps on raw pinhole camera images and can recover the distance of dynamic objects.}
\label{fig:KITTIDepthComparison}
\end{figure*}
% -------------------------------------------------
\begin{figure*}[!ht]
\captionsetup{belowskip=-8pt, singlelinecheck=false, font=small}
  \centering
  \resizebox{\textwidth}{!}{
  \newcommand{\turnheightnew}{0.3\columnwidth}
\centering

\begin{tabular}{@{\hskip 0.5mm}c@{\hskip 0.5mm}c@{\hskip 0.5mm}c@{\hskip 0.5mm}c@{\hskip 0.5mm}c@{}}

{\rotatebox{90}{\hspace{3mm}Raw Input}} &
\includegraphics[height=\turnheightnew]{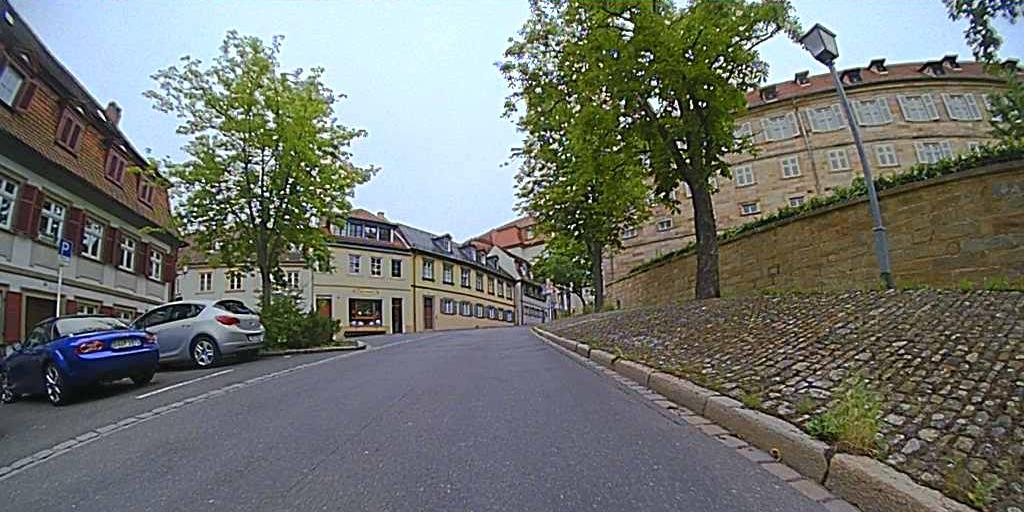} &
\includegraphics[height=\turnheightnew]{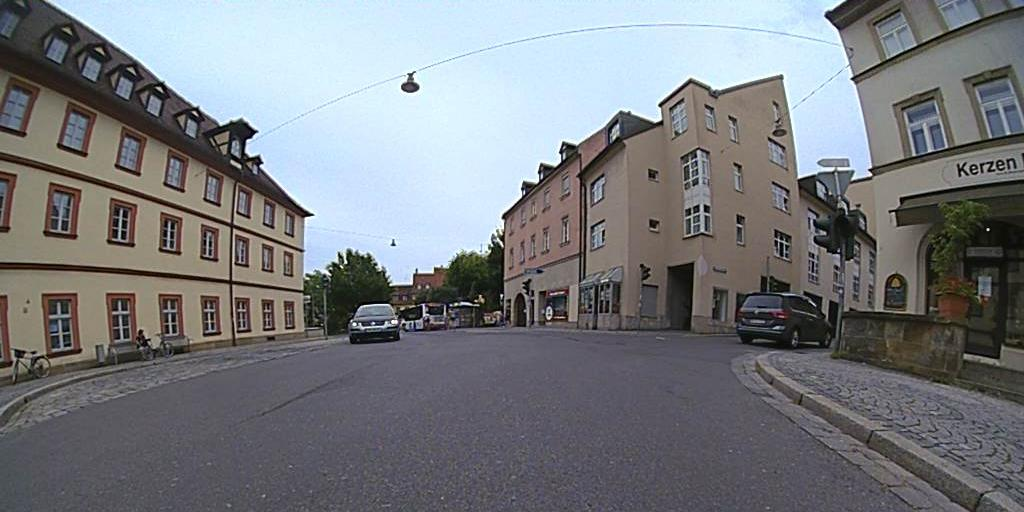} &
\includegraphics[height=\turnheightnew]{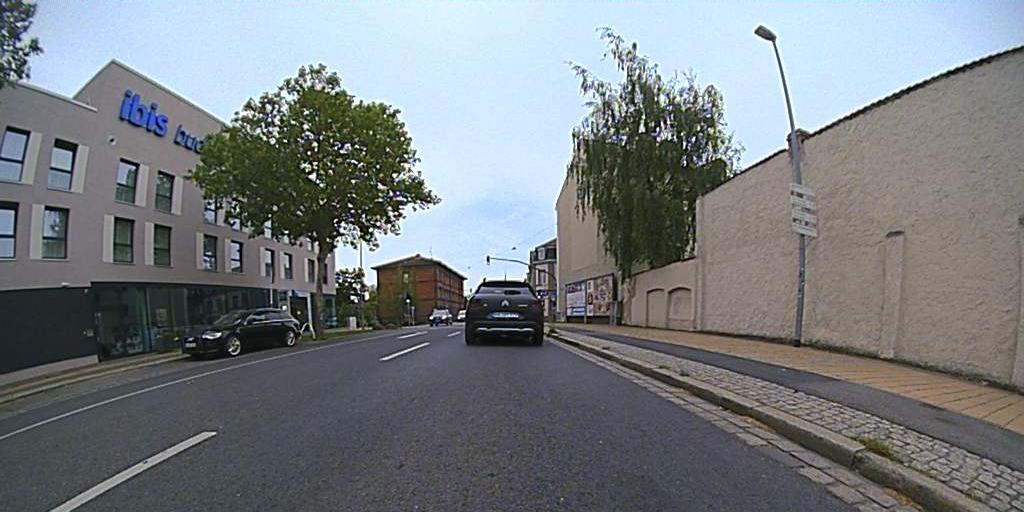} &
\includegraphics[height=\turnheightnew]{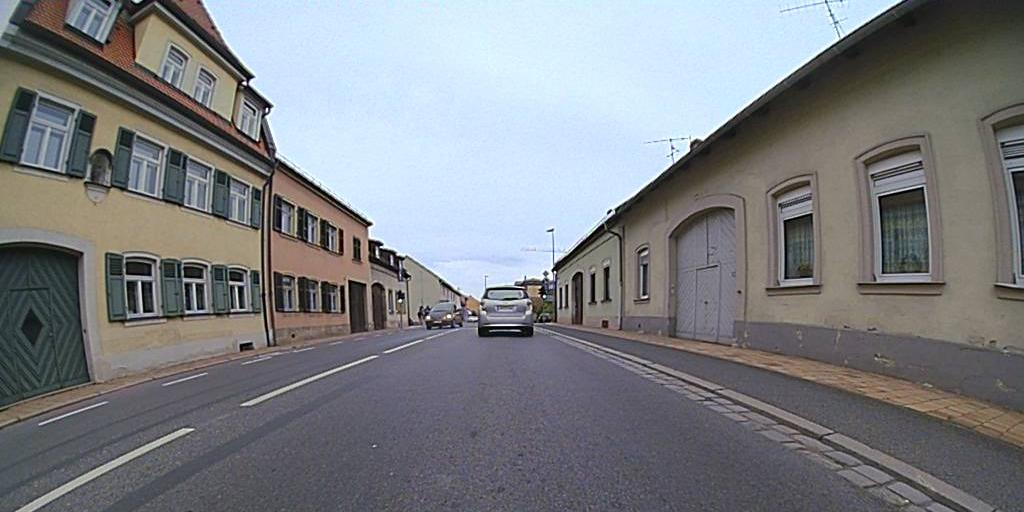}\\

{\rotatebox{90}{\hspace{3mm}Baseline~\cite{kumar2020fisheyedistancenet}}} &
\includegraphics[height=\turnheightnew]{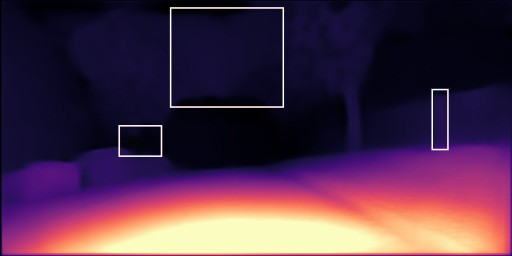} &
\includegraphics[height=\turnheightnew]{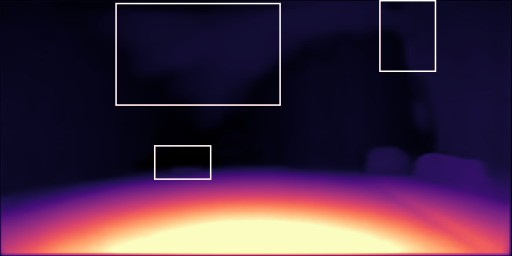} &
\includegraphics[height=\turnheightnew]{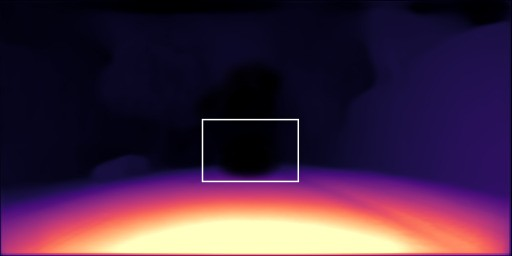} &
\includegraphics[height=\turnheightnew]{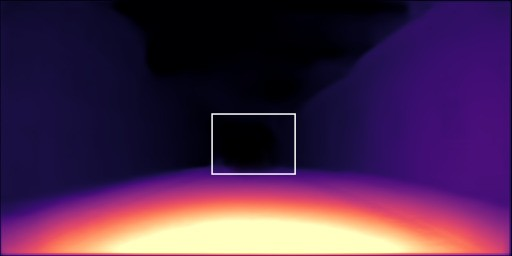}\\

{\rotatebox{90}{\hspace{3mm}SVDistNet}} &
\includegraphics[height=\turnheightnew]{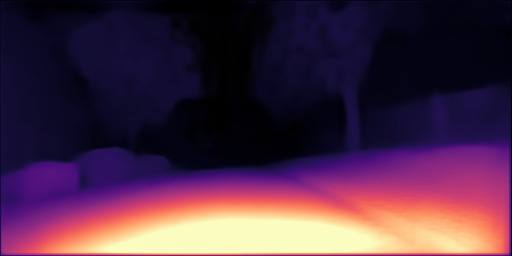} &
\includegraphics[height=\turnheightnew]{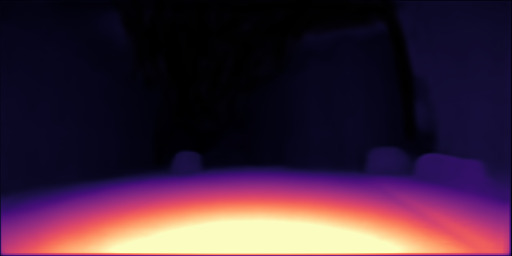} &
\includegraphics[height=\turnheightnew]{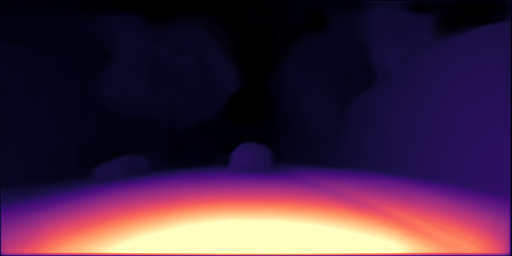} &
\includegraphics[height=\turnheightnew]{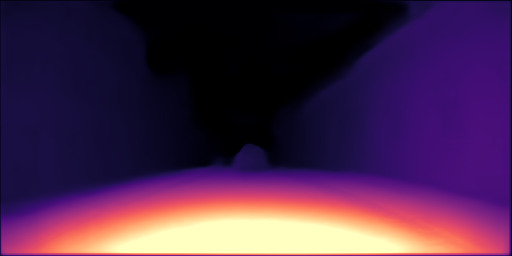} \\

{\rotatebox{90}{\hspace{3mm}SVDistNet}} &
\includegraphics[height=\turnheightnew]{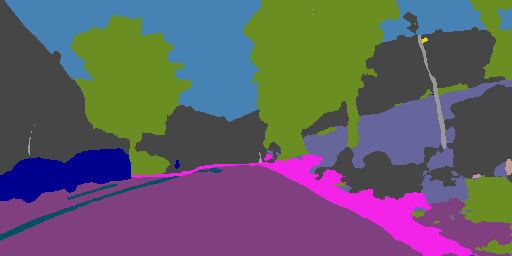} &
\includegraphics[height=\turnheightnew]{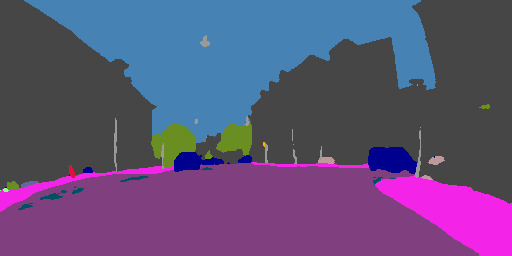} &
\includegraphics[height=\turnheightnew]{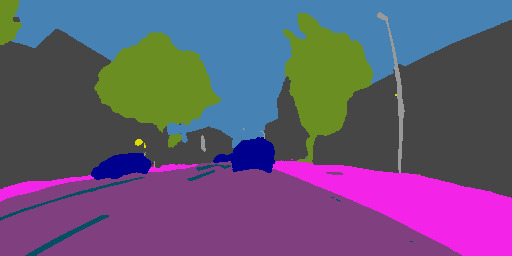} &
\includegraphics[height=\turnheightnew]{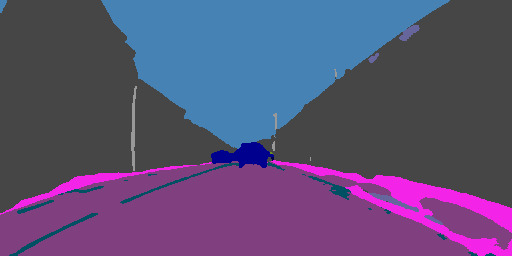}

\end{tabular}}
\caption{\textbf{Evaluation of our SVDistNet model on the Fisheye WoodScape dataset.} We compare our baseline work FisheyeDistanceNet~\cite{kumar2020fisheyedistancenet} trained only for the task of distance estimation to our SVDistNet, which is trained in a multi-task fashion. We observe that using semantic guidance inside the SVDistNet model helps recover thin structures inside the distance map (left images). We also solve the infinite depth issue for dynamic objects by incorporating the mask described in Section~\ref{sec:dynamic-object-mask} (right images).}
  \label{fig:fisheye_qual}
\end{figure*}
% -------------------------------------------------
