# Supplementary material for: SVDistNet: Self-Supervised Near-Field Distance Estimation on Surround View Fisheye Cameras
Source: arXiv:2104.04420 source file (2021-04-09)
Supplement: Supplementary file 2 [file cam_tensor_suppl.tex]

\newcommand{\turnheightnew}{0.5\columnwidth}
\centering
\begin{tabular}{@{\hskip 0.5mm}c@{\hskip 0.5mm}c@{\hskip 0.5mm}c@{}}

\includegraphics[height=\turnheightnew]{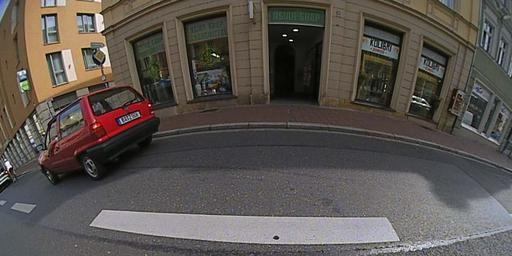} &
\includegraphics[height=\turnheightnew]{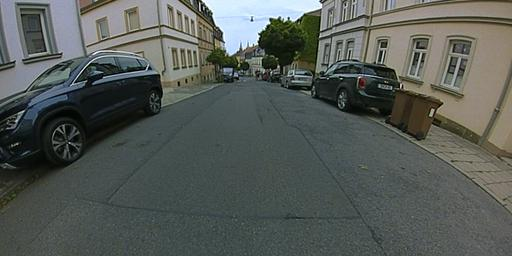} \\
\includegraphics[height=\turnheightnew]{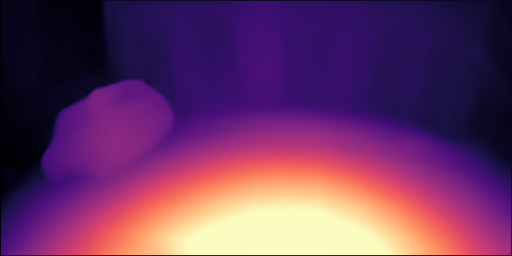} &
\includegraphics[height=\turnheightnew]{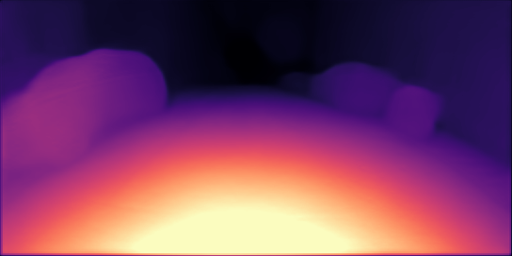} \\
\includegraphics[height=\turnheightnew]{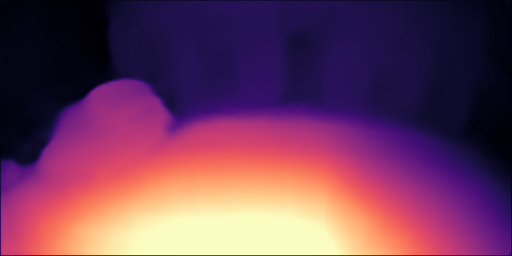} &
\includegraphics[height=\turnheightnew]{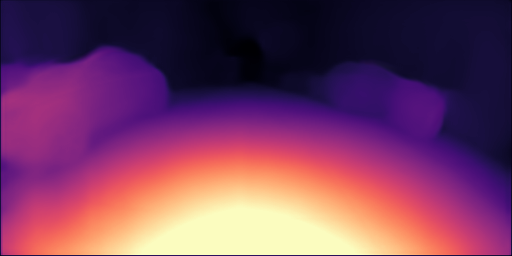} \\
\end{tabular}
