# Supplementary material for: SVDistNet: Self-Supervised Near-Field Distance Estimation on Surround View Fisheye Cameras
Source: arXiv:2104.04420 source file (2021-04-09)
Supplement: Supplementary file 4 [file kitti_sem_suppl.tex]

\newcommand{\turnheightnew}{0.45\columnwidth}
\centering

\begin{adjustbox}{width=\textwidth, totalheight=8.2in, keepaspectratio}
\begin{tabular}{@{\hskip 0.5mm}c@{\hskip 0.5mm}c@{\hskip 0.5mm}c@{\hskip 0.5mm}}

{\rotatebox{90}{\hspace{9mm} \large Raw Input}} &
\includegraphics[height=\turnheightnew]{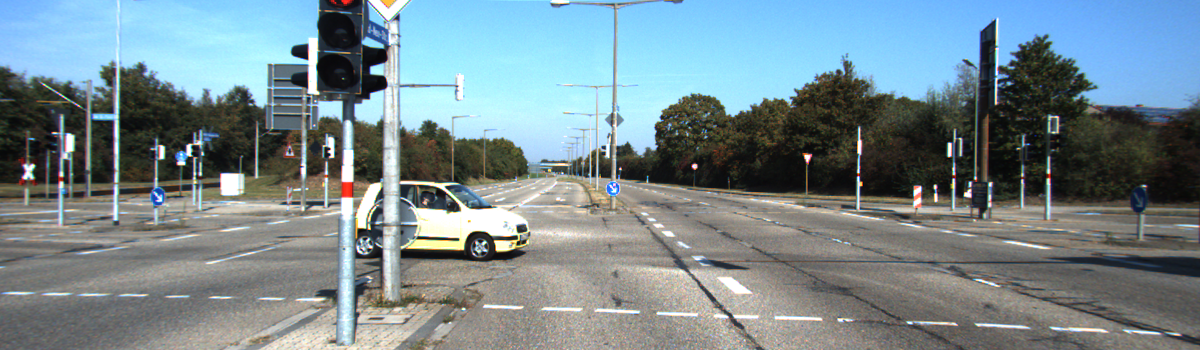} &
\includegraphics[height=\turnheightnew]{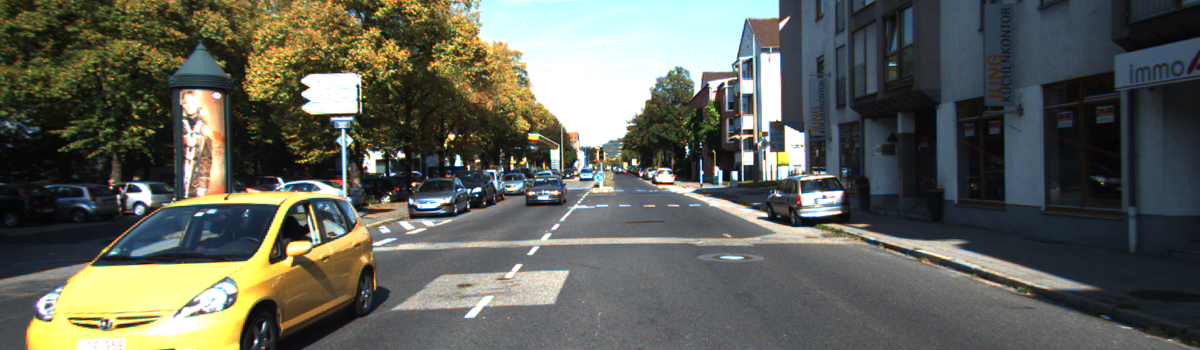} \\

{\rotatebox{90}{\hspace{9mm} \large SVDistNet}} &
\includegraphics[height=\turnheightnew]{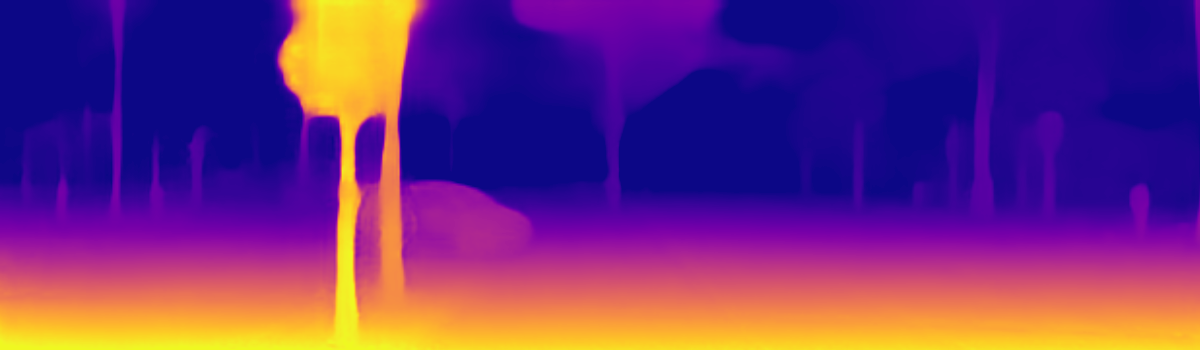} &
\includegraphics[height=\turnheightnew]{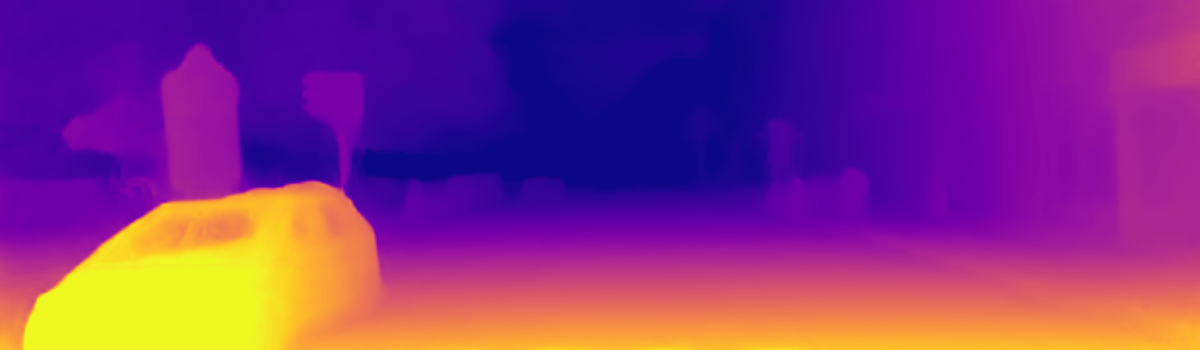} \\

{\rotatebox{90}{\hspace{9mm} \large SVDistNet}} &
\includegraphics[height=\turnheightnew]{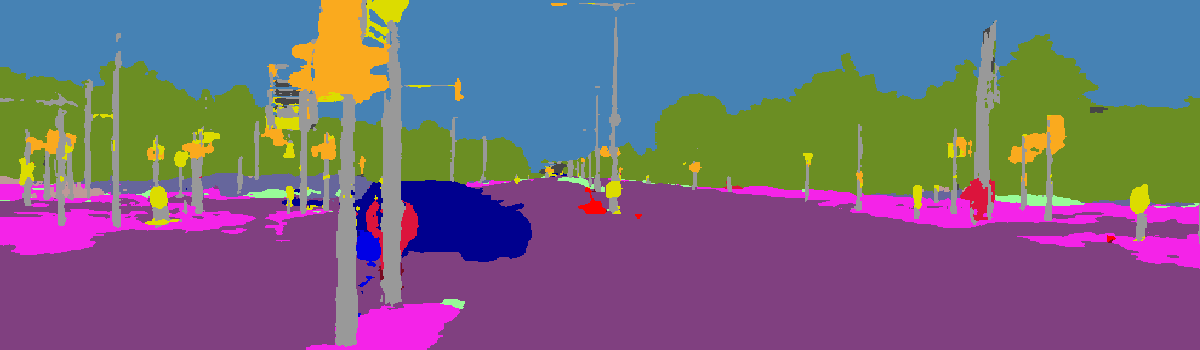} &
\includegraphics[height=\turnheightnew]{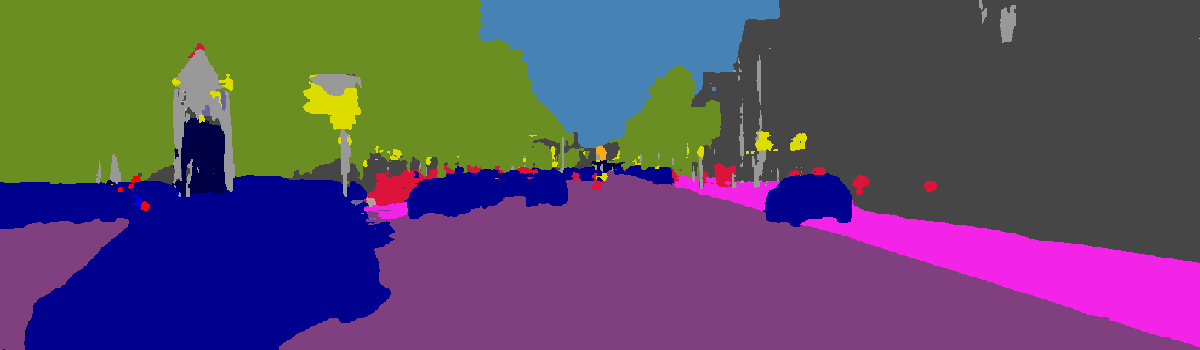} \\

{\rotatebox{90}{\hspace{9mm} \large Raw Input}} &
\includegraphics[height=\turnheightnew]{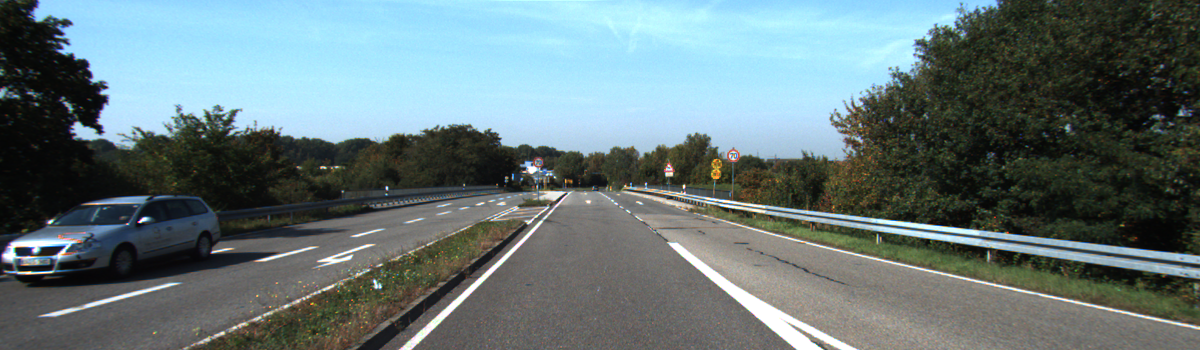} &
\includegraphics[height=\turnheightnew]{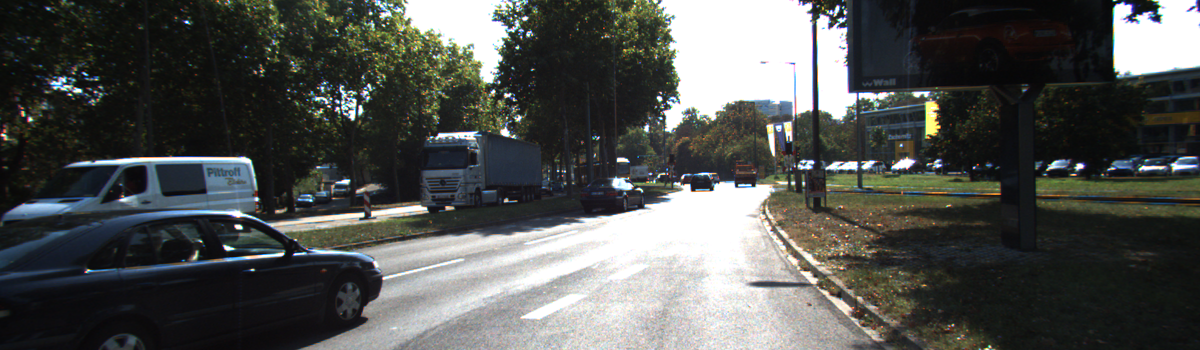} \\

{\rotatebox{90}{\hspace{9mm} \large SVDistNet}} &
\includegraphics[height=\turnheightnew]{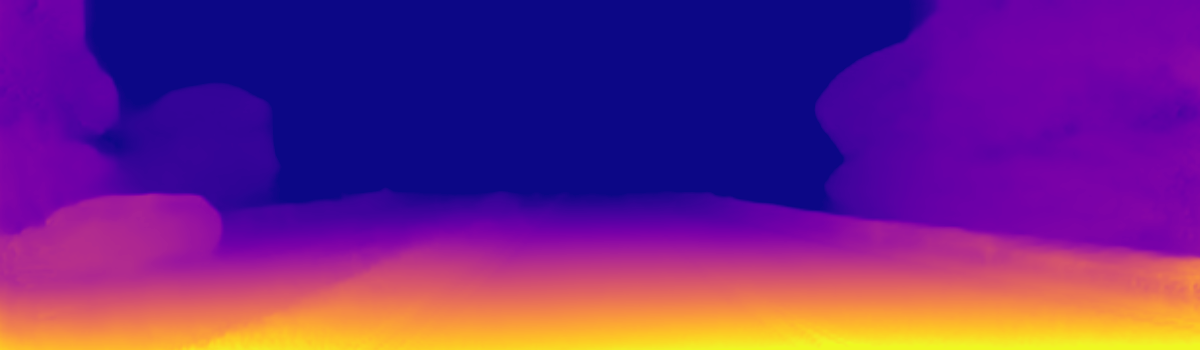} &
\includegraphics[height=\turnheightnew]{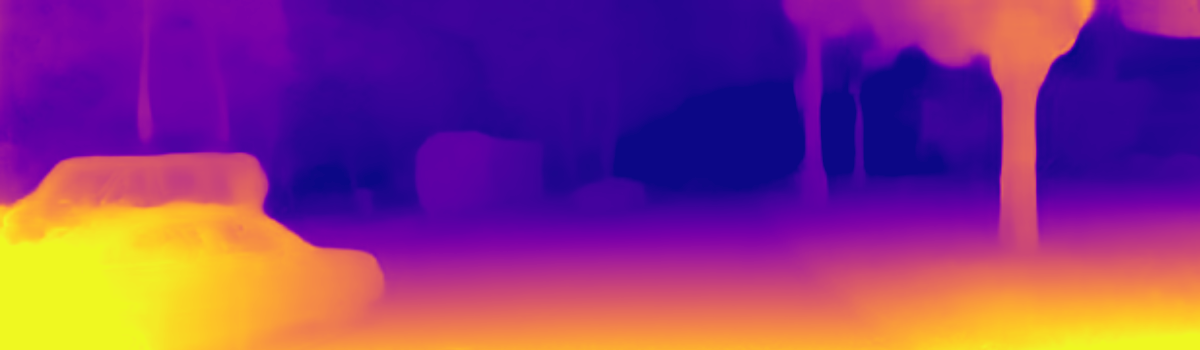} \\

{\rotatebox{90}{\hspace{9mm} \large SVDistNet}} &
\includegraphics[height=\turnheightnew]{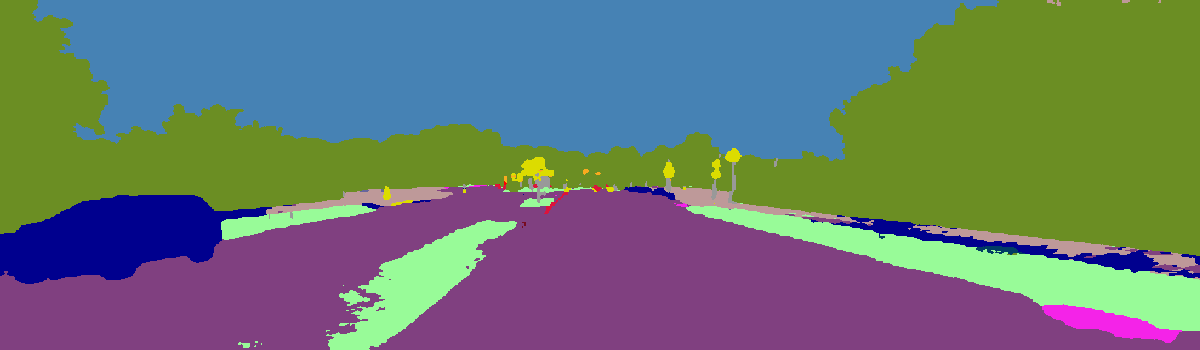} &
\includegraphics[height=\turnheightnew]{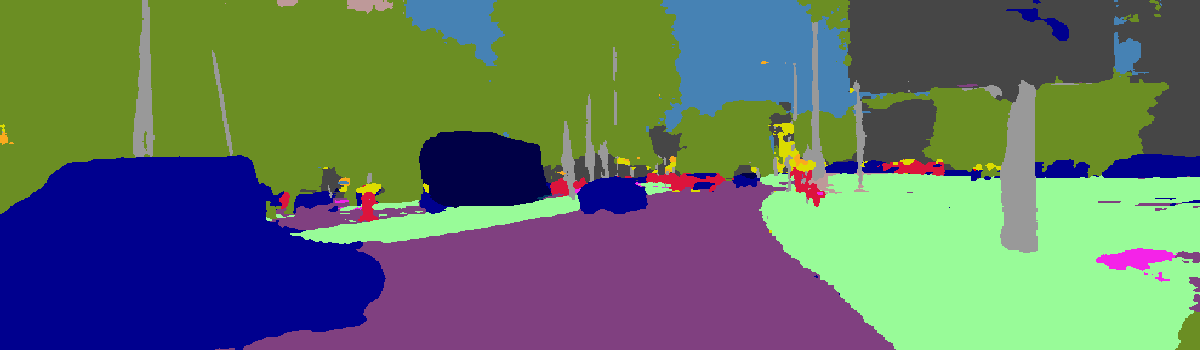} \\

{\rotatebox{90}{\hspace{9mm} \large Raw Input}} &
\includegraphics[height=\turnheightnew]{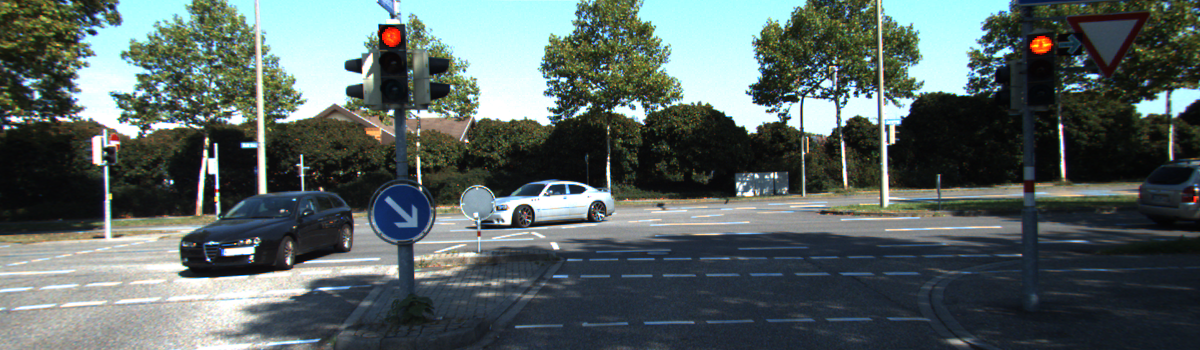} &
\includegraphics[height=\turnheightnew]{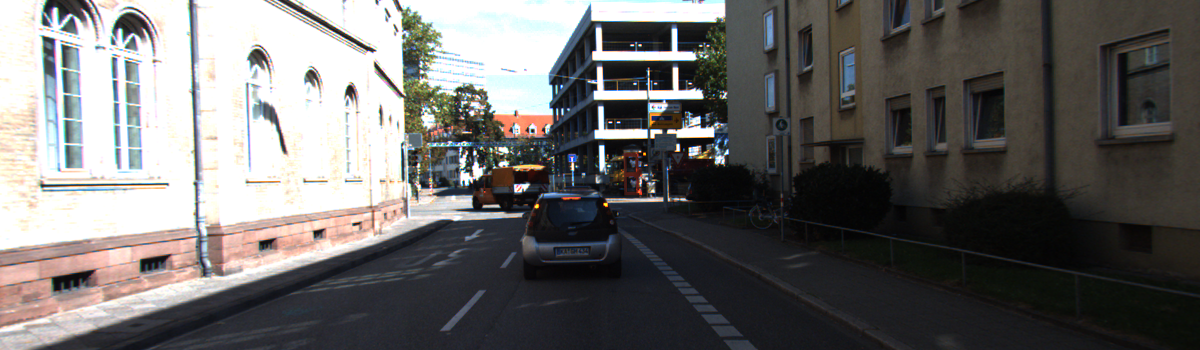} \\

{\rotatebox{90}{\hspace{9mm} \large SVDistNet}} &
\includegraphics[height=\turnheightnew]{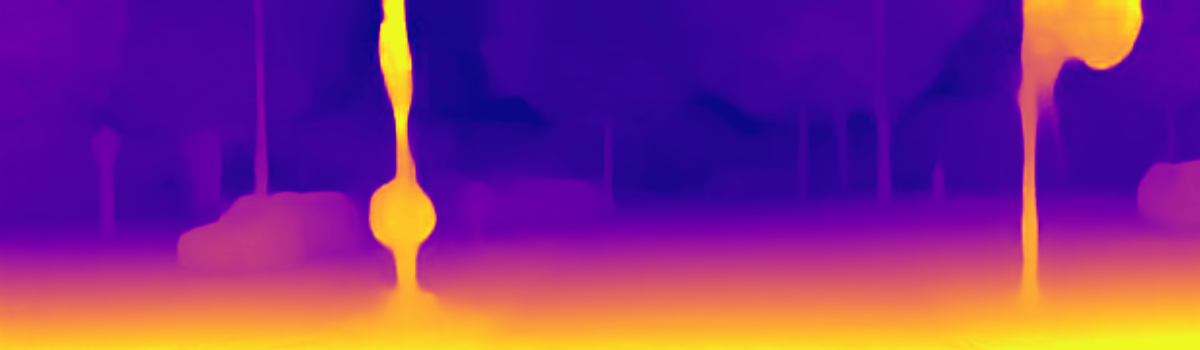} &
\includegraphics[height=\turnheightnew]{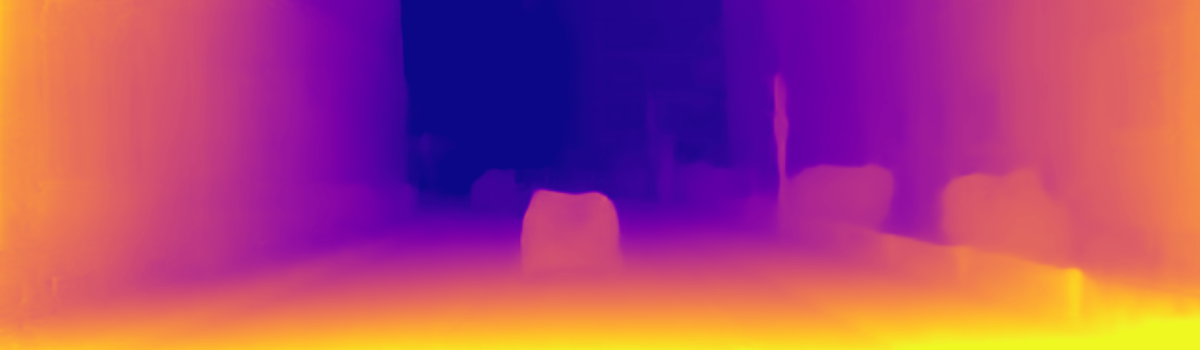} \\

{\rotatebox{90}{\hspace{9mm} \large SVDistNet}} &
\includegraphics[height=\turnheightnew]{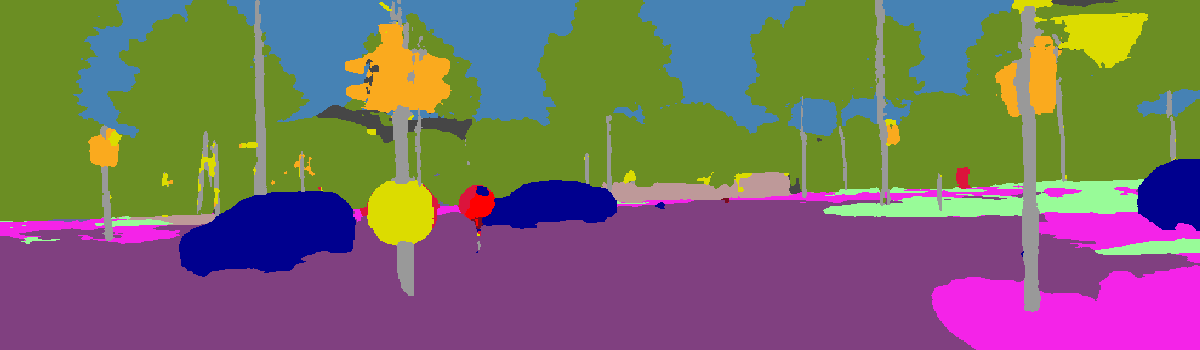} &
\includegraphics[height=\turnheightnew]{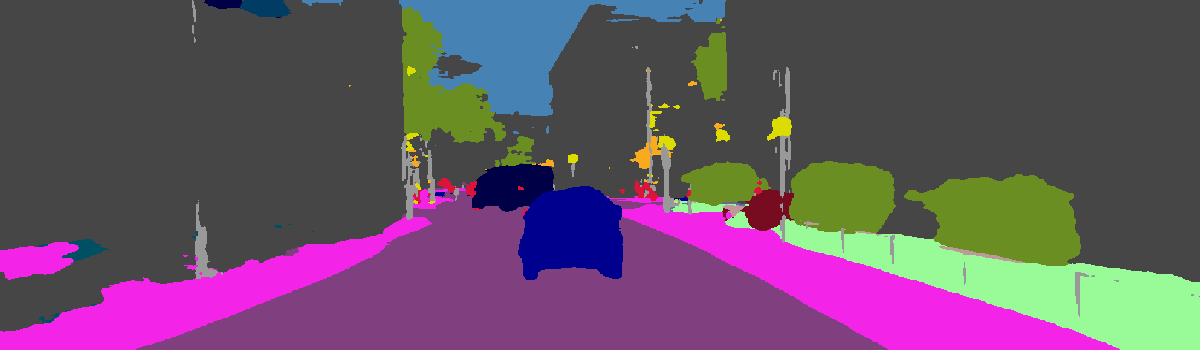} \\

%{\rotatebox{90}{\hspace{3mm}Raw Input}} &
%\includegraphics[height=\turnheightnew]{img/kitti_fig/imgs_sem/rgb_baseline_image000.png} &
%\includegraphics[height=\turnheightnew]{img/kitti_fig/imgs_sem/rgb_baseline_image140.png} \\

%{\rotatebox{90}{\hspace{3mm}SVDistNet}} &
%\includegraphics[height=\turnheightnew]{img/kitti_fig/imgs_sem/depth_predicted000.png} &
%\includegraphics[height=\turnheightnew]{img/kitti_fig/imgs_sem/depth_predicted140.png} \\

%{\rotatebox{90}{\hspace{3mm}SVDistNet}} &
%\includegraphics[height=\turnheightnew]{img/kitti_fig/imgs_sem/sem_predicted_image000.png} &
%\includegraphics[height=\turnheightnew]{img/kitti_fig/imgs_sem/sem_predicted_image140.png}\\

\end{tabular}
\end{adjustbox}
